# Supplementary material for: A homogeneous measurement of the delay between the onsets of gas stripping and star formation quenching in satellite galaxies of groups and clusters
Source: arXiv:2009.00667 source file (2024-06-07)
Supplement: Supplementary file 1 [file appendices.pdf]

Mon. Not. R. Astron. Soc. **000**, 000–000 (0000) Printed 19 November 2020 (MN LaTeX style file v2.2)

# A homogeneous measurement of the delay between the onsets of gas stripping and star formation quenching in satellite galaxies of groups and clusters: Appendices

Kyle A. Oman[1,2], Yannick M. Bahé[3], Julia Healy[2,4], Kelley M. Hess[2,5], Michael J. Hudson[6,7], Marc A. W. Verheijen[2]

[1] *Institute for Computational Cosmology, Department of Physics, Durham University, South Road, Durham DH1 3LE, United Kingdom*
[2] *Kapteyn Astronomical Institute, University of Groningen, Postbus 800, NL-9700 AV Groningen, The Netherlands*
[3] *Leiden Observatory, Leiden University, PO Box 9513, NL-2300 RA Leiden, the Netherlands*
[4] *Department of Astronomy, University of Cape Town, Private Bag X3, Rondebosch 7701, South Africa*
[5] *ASTRON, the Netherlands Institute for Radio Astronomy, Postbus 2, NL-7990 AA Dwingeloo, the Netherlands*
[6] *Department of Physics and Astronomy, University of Waterloo, Waterloo, ON N2L 3G1, Canada*
[7] *Perimeter Institute for Theoretical Physics, Waterloo, ON N2L 2Y5, Canada*

19 November 2020

These appendices include:

- Appendix A: Figures similar to Fig. 3 for all bins in host mass and satellite stellar mass.
- Appendix B: Expanded version of Fig. 10 including $\Delta t$, and alternative version of Fig. 10 where $f_{\mathrm{after}}$ is a free parameter.
- Appendix C: Re-derivations of our main results assuming different definitions of what constitutes a 'gas rich' galaxy.
- Appendix D: Figures similar to Figs. 7 and 8 for the other stellar mass bins included in Fig. 9.
- Appendix E: Tables with the median and 68 per cent confidence intervals for all the marginalized posterior probability distributions shown in the supplementary Figs. B1–B4 (i.e. including those from Fig. 10).
- Appendix F: Figures showing the individual and pairwise marginalized probability distributions (i.e. similar to Fig. 8) for the parameters summarized in Fig. 10, and similar constraints when $f_{\mathrm{after}}$ is a free parameter.

© 0000 RAS

## APPENDIX A: BLUE, ACTIVE AND H I-DETECTED FRACTIONS IN PROJECTED PHASE SPACE

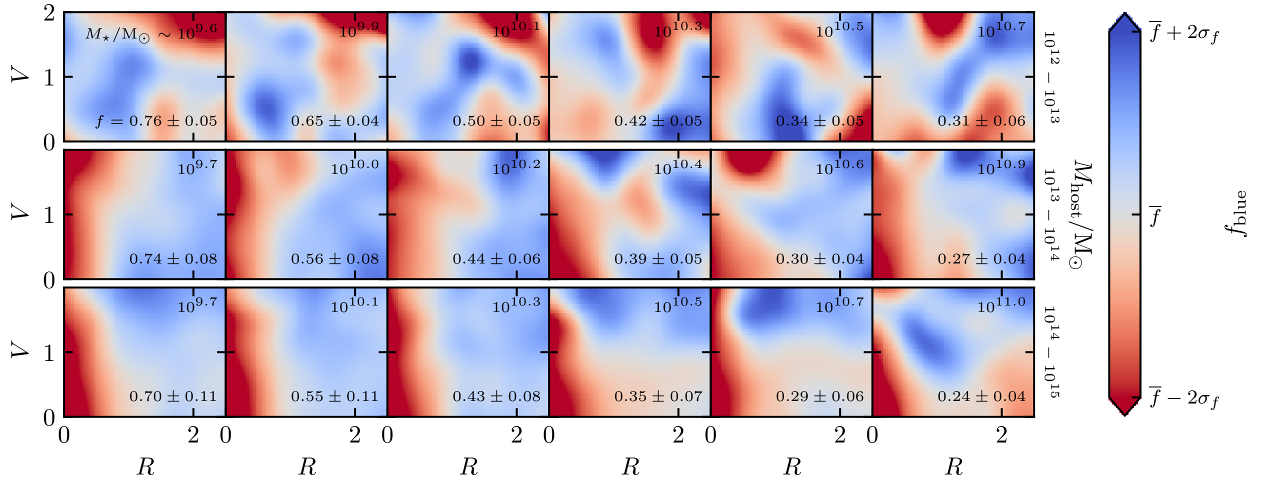


**Figure A1.** Similar to Fig. 3. Fraction of blue (see Fig. 2) galaxies as a function of normalized projected position $R/r_{\rm vir}$ and velocity $V/\sigma_{\rm 3D}$ offset from the host group centre. Each row corresponds to hosts in a virial mass interval as labelled at the right, and each column to an interval in satellite stellar mass (the same used for the six points in Figs. 10 and 11); the median is noted in the upper right of each panel. The colour scale is different for each panel and is centered at the mean plotted fraction ($\overline{f}$) and extends to $\pm 2\sigma_f$, where $\sigma_f$ is the root mean square scatter. The values of $\overline{f} \pm \sigma_f$ are noted in the lower right of each panel.

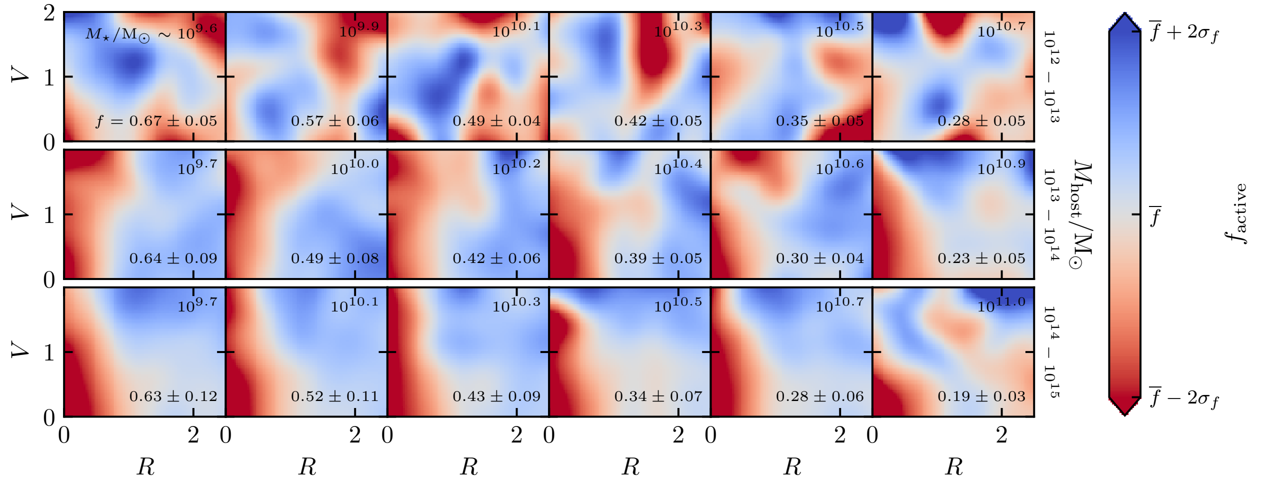


**Figure A2.** As in Fig. A1, but for the active fraction.

© 0000 RAS, MNRAS **000**, 000–000

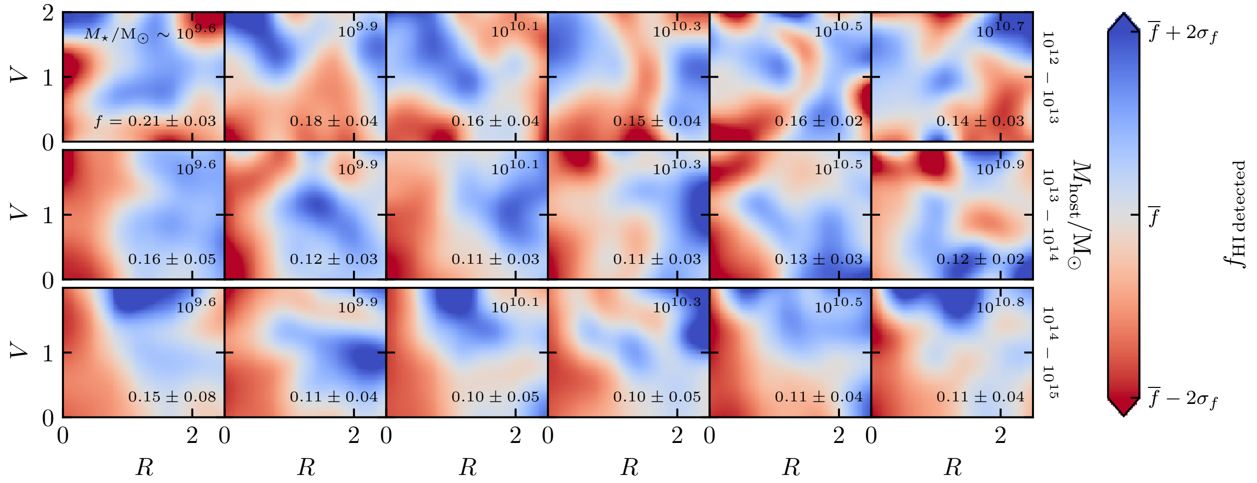


**Figure A3.** As in Fig. A1, but for the fraction detected in the ALFALFA survey.

## APPENDIX B: MODEL CONSTRAINTS INCLUDING $\Delta t$, AND ALTERNATE CONSTRAINTS WITH $f_{\rm after}$ FREE

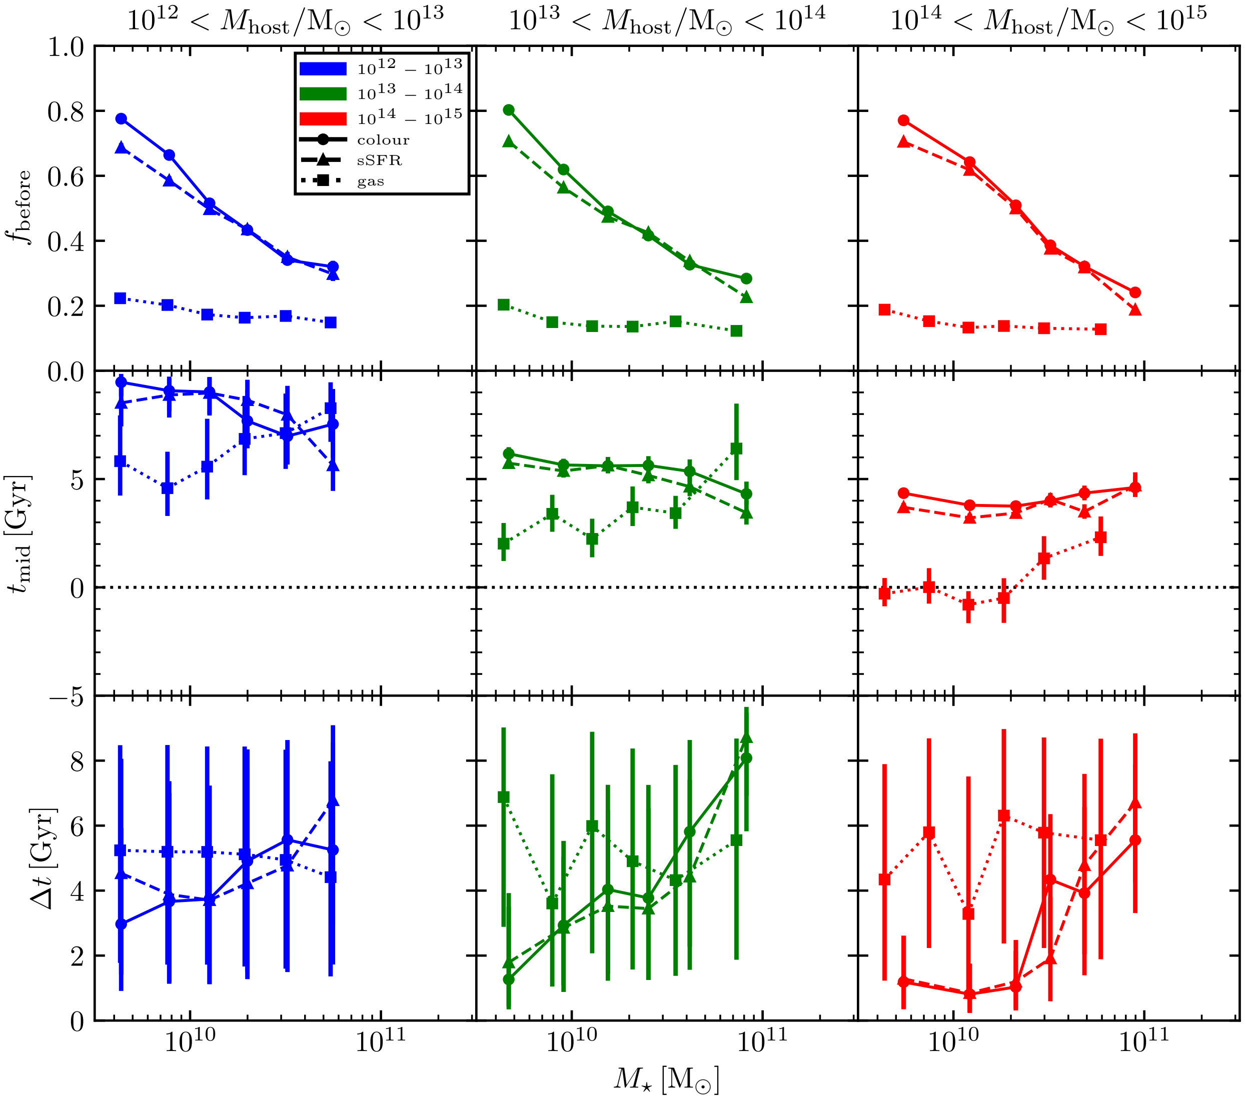


**Figure B1.** Similar to Fig. 10, upper panels – the upper two rows are repeated from that figure. The lower row shows the marginalized 16–84$^{\rm th}$ percentile confidence intervals for the $\Delta t$ parameter, which is in general poorly constrained and which we have treated as a 'nuisance parameter', marginalizing over it, in our analysis.

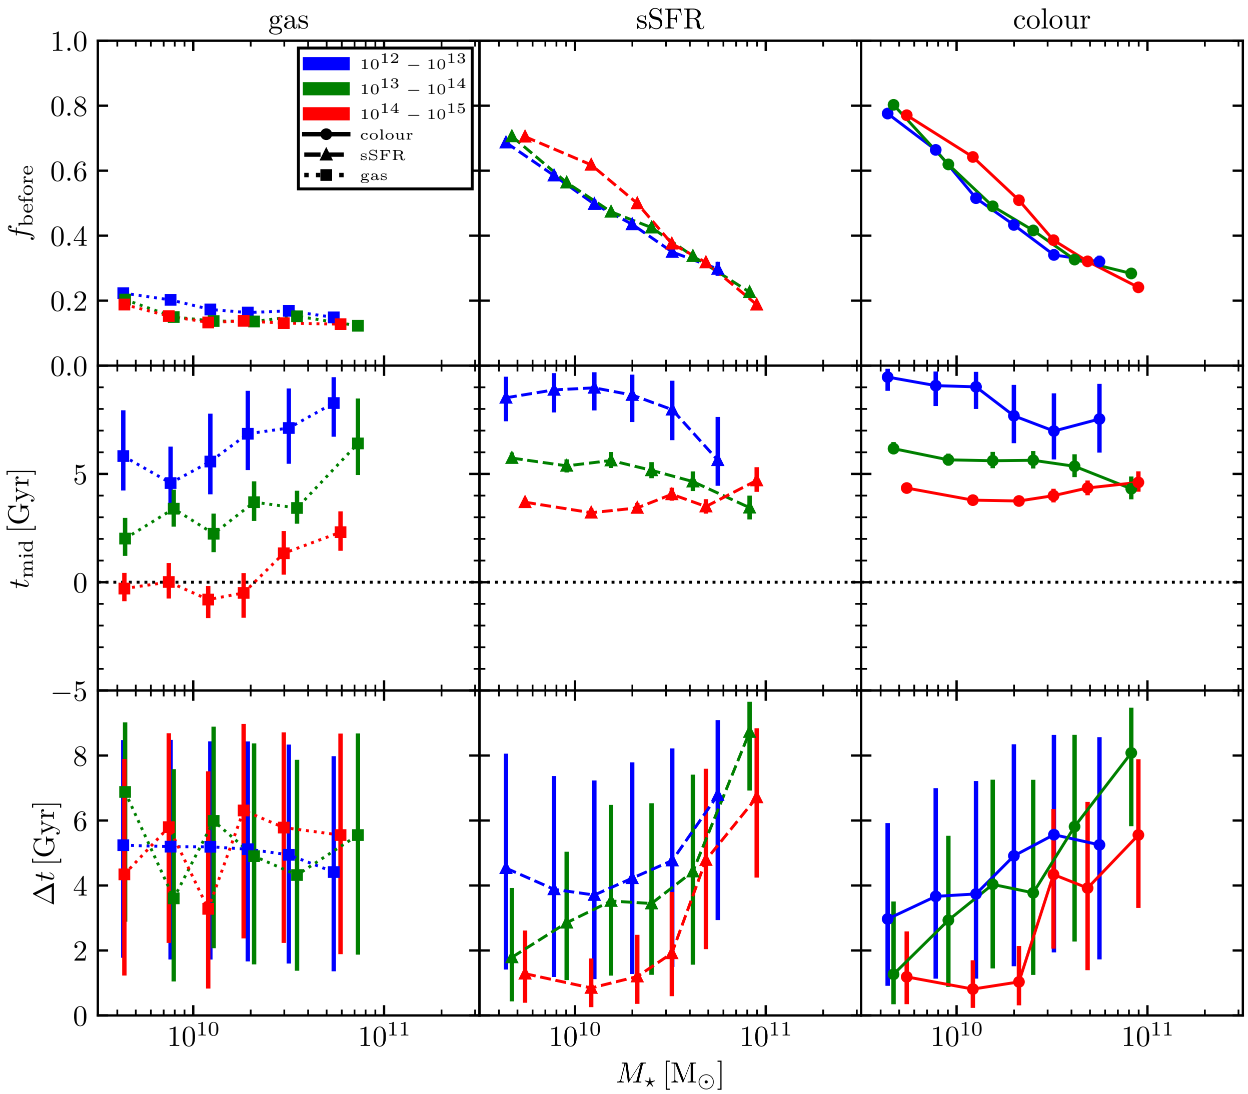


**Figure B2.** Similar to Fig. 10, lower panels, but including the constraints on $\Delta t$, as in Fig. B1.

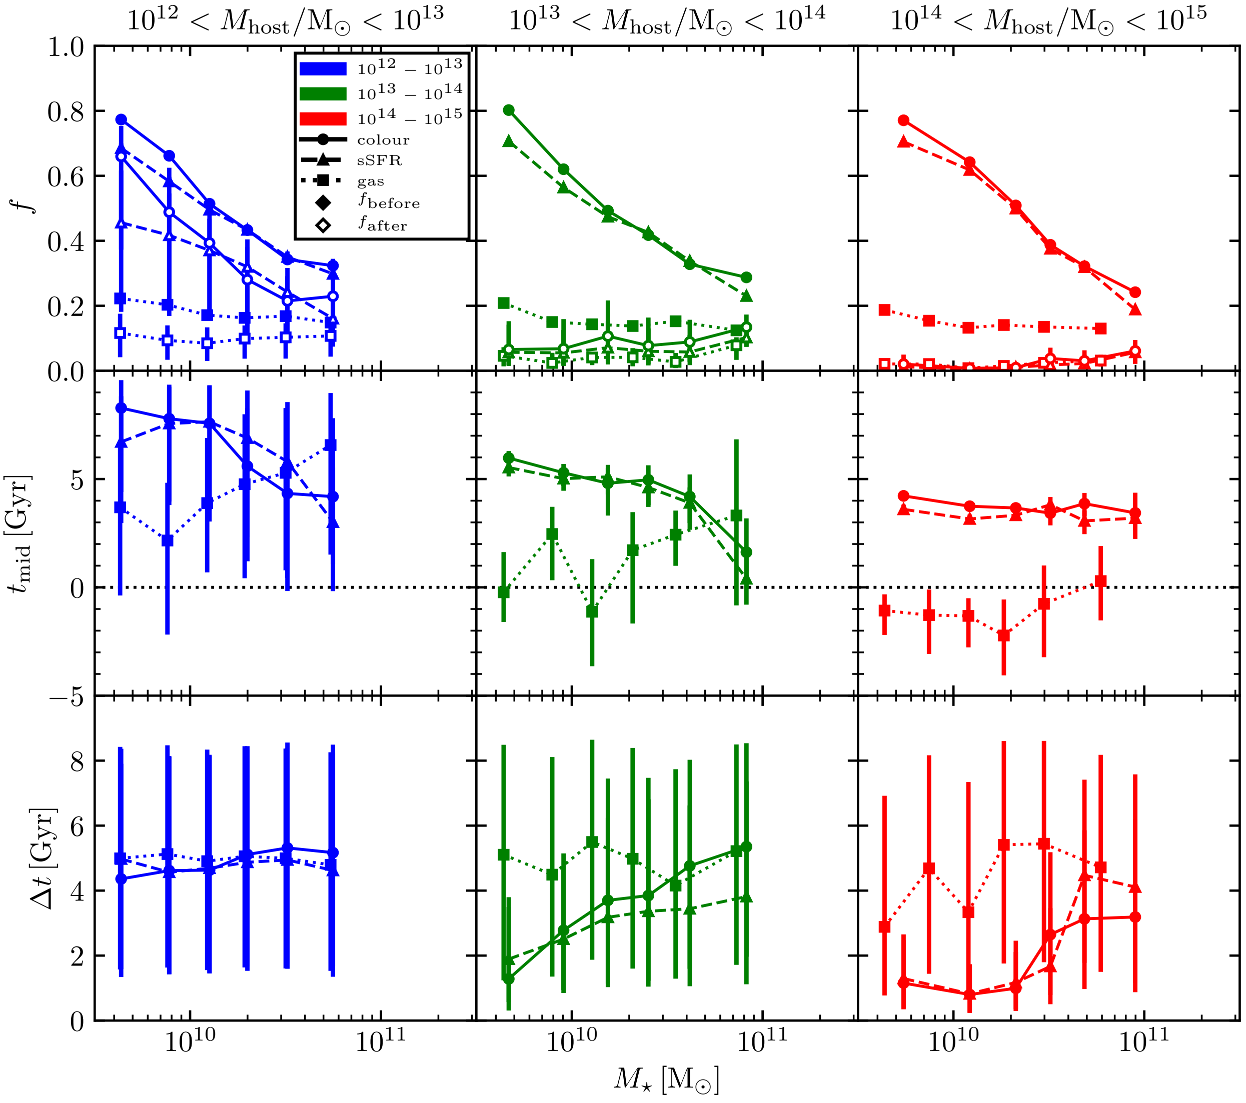


**Figure B3.** As in Fig. B1, but showing the parameter constraints when $f_{\rm after}$ is treated as a free parameter, rather than fixed to $f_{\rm after} = 0$. The open symbols in the upper row of panels show the median and 16–84$^{\rm th}$ percentile confidence interval for $f_{\rm after}$, with the same colour, symbol and line styles as for $f_{\rm before}$.

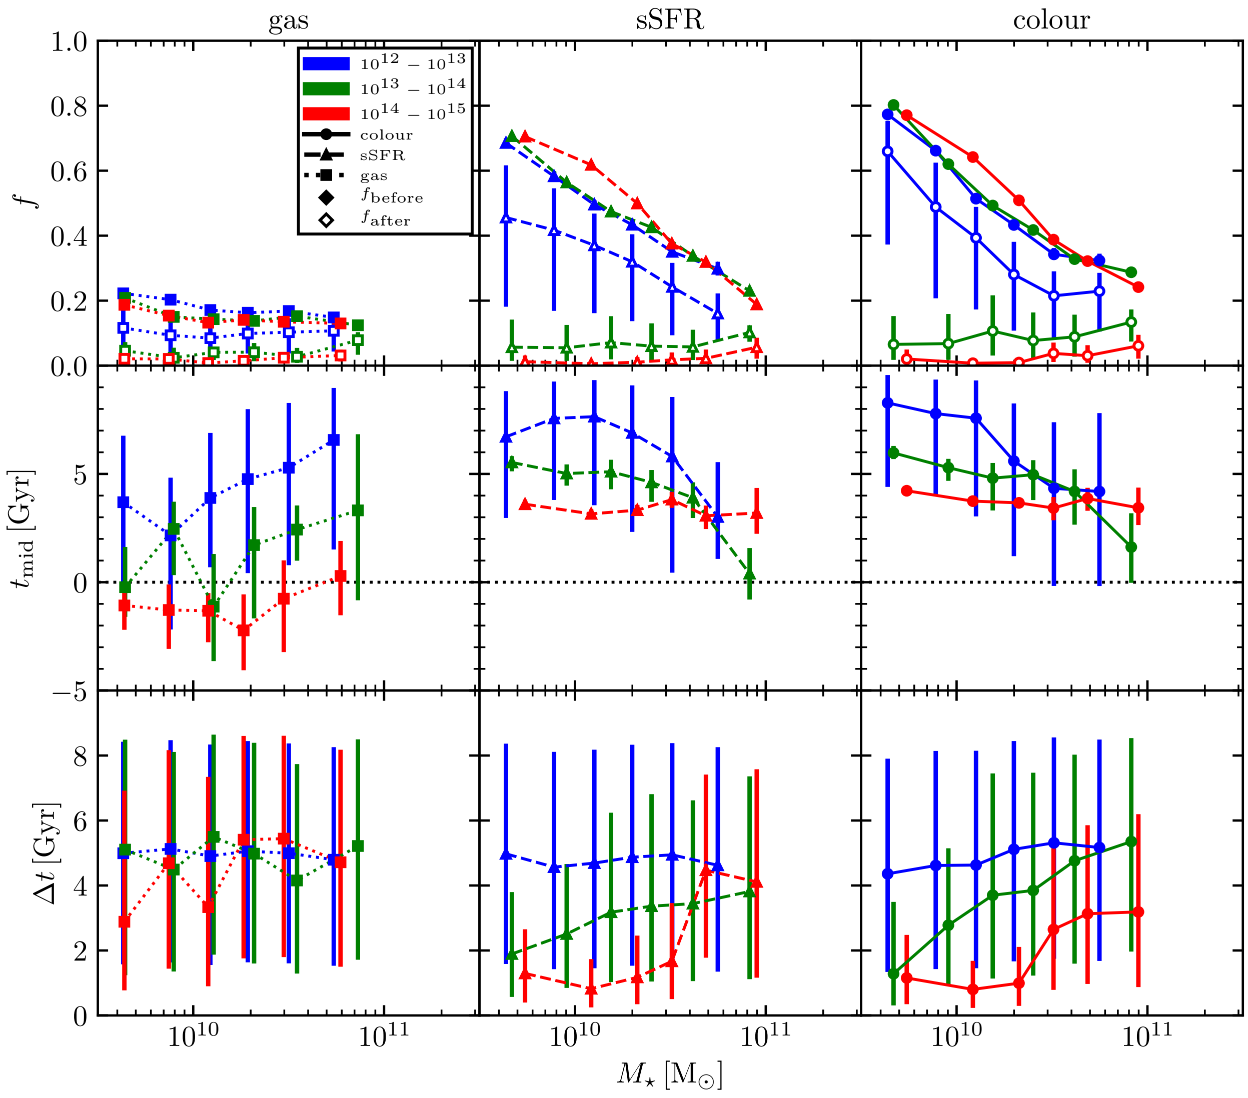


**Figure B4.** As Fig. B3, but with the curves re-arranged to emphasize trends with $M_{\rm host}$.

## APPENDIX C: MODEL CONSTRAINTS USING ALTERNATIVE DEFINITIONS OF 'GAS RICH'

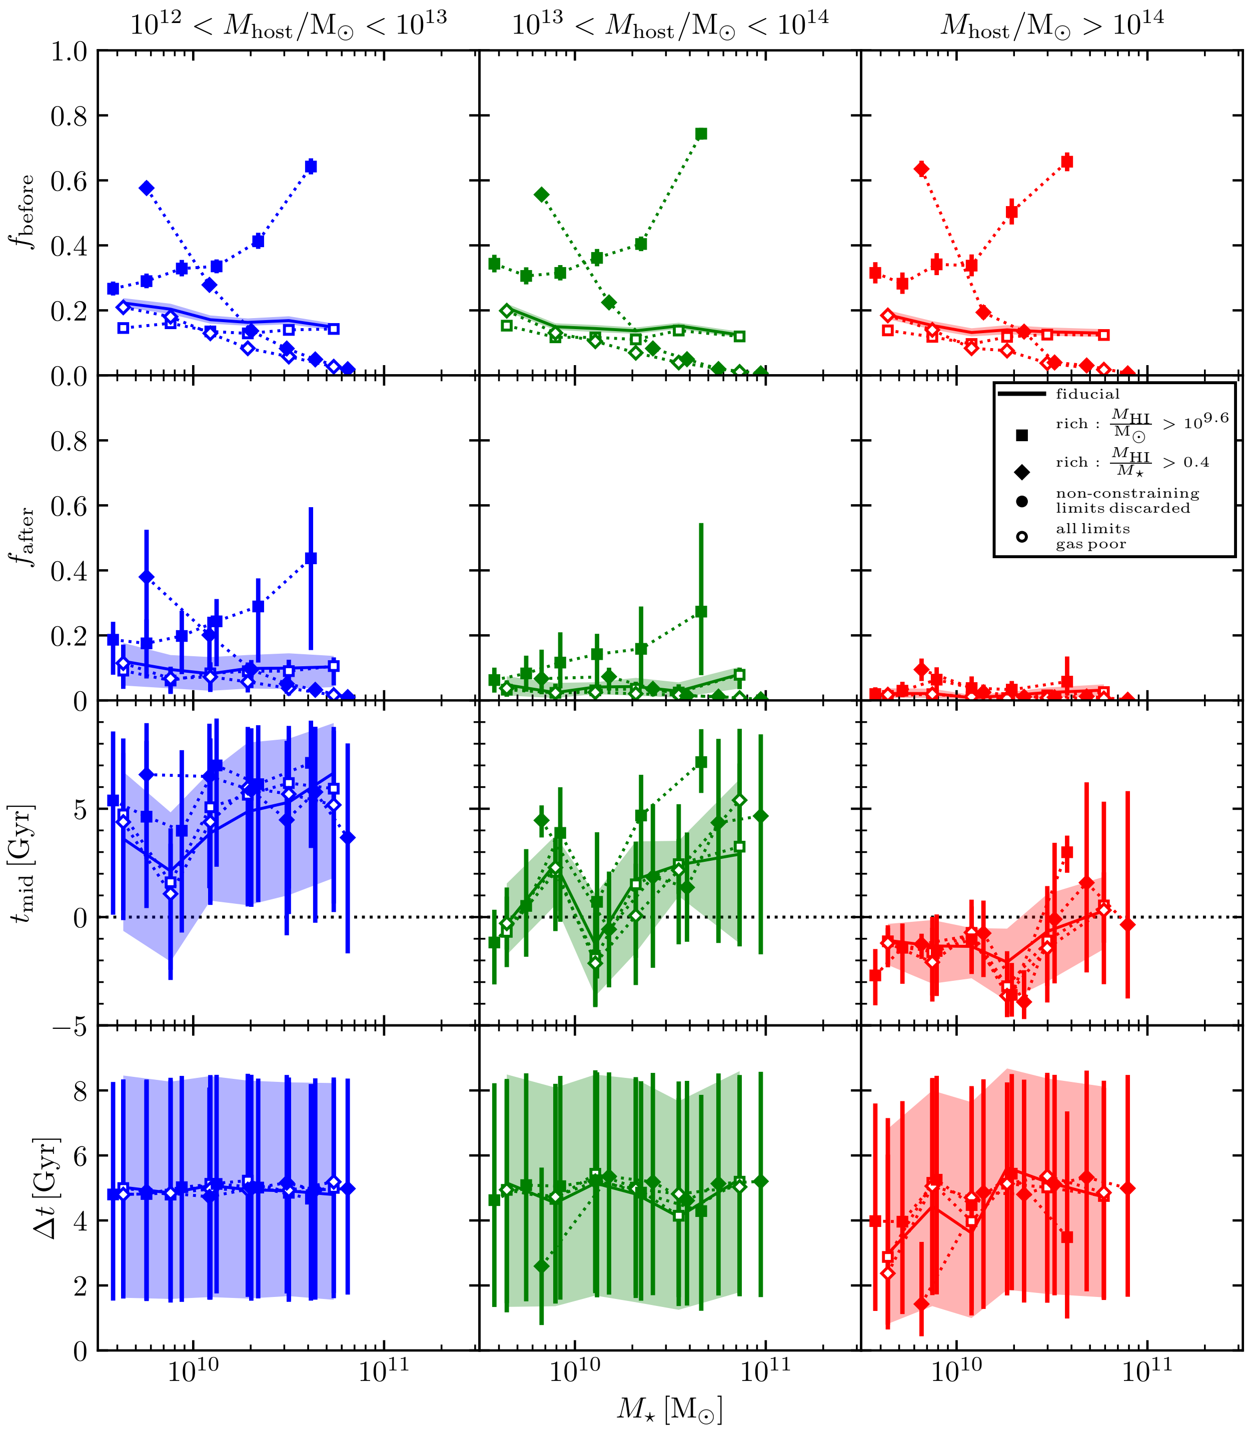


**Figure C1.** Model constraints for variations in the definition of ‘gas rich’ used. The fiducial definition is that galaxies detected in ALFALFA are labelled ‘gas rich’, while those not detected are ‘gas poor’. The solid lines and shaded regions show the median and $16^{\rm th}$ to $84^{\rm th}$ percentile constraints for the fiducial definition, with $f_{\rm after}$ free to vary, and correspond to those shown in Figs. B3 and B4. We show the alternative constraints for four cases. We vary the limit where galaxies are defined as ‘gas rich’, either as those with H I fractions ($M_{\rm HI}/M_\star$) larger than 0.4 (squares) or H I masses larger than $10^{9.6}$ M$_\odot$ (diamonds). Qualitatively similar results are obtained for reasonably variations in these thresholds. We also vary the treatment of ALFALFA non-detections, either discarding all galaxies whose upper limits are not constraining (i.e. which are greater than the ‘gas rich’ threshold; filled points) or considering galaxies with upper limits as ‘gas poor’ (open points). The discrepancies in $f_{\rm before}$ and $f_{\rm after}$ are expected as these parameters are more a reflection of the definition of ‘gas rich’ rather than any intrinsic property of the galaxies. The $t_{\rm mid}$ constraints, however, are consistent within the statistical uncertainties: our qualitative conclusion that ‘quenching lags stripping’ is therefore robust to reasonable changes in the definition of ‘gas richness’.

## APPENDIX D: ADDITIONAL DETAILS ON TESTS OF THE MODEL WITH HYDRANGEA MOCKS

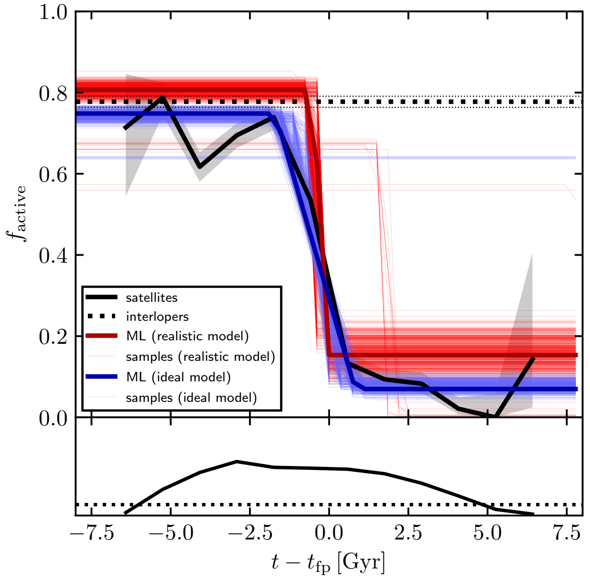


**Figure D1.** As Fig. 7, but for the first stellar mass bin (leftmost points in Fig. 9).

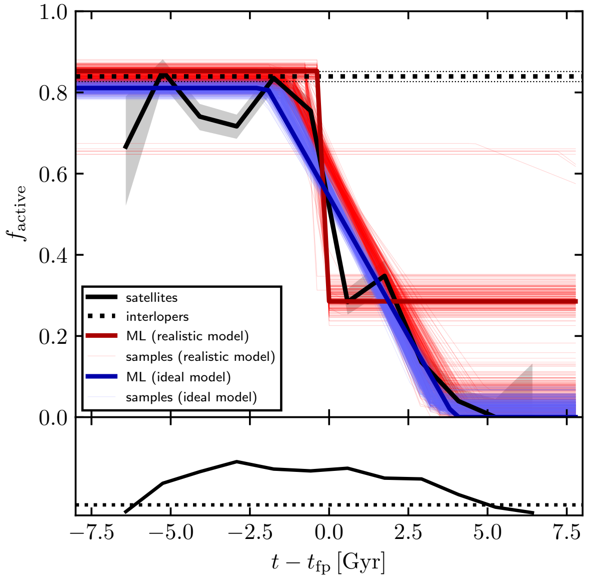


**Figure D2.** As Fig. 7, but for the second stellar mass bin (centre-left points in Fig. 9).

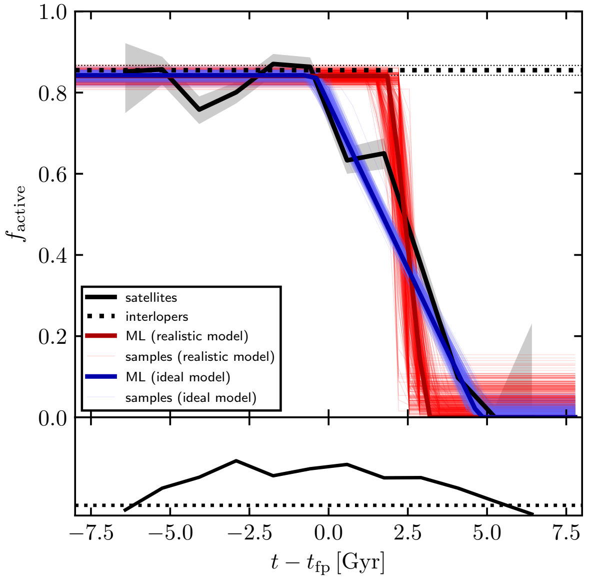


**Figure D3.** As Fig. 7, but for the third stellar mass bin (centre-right points in Fig. 9).

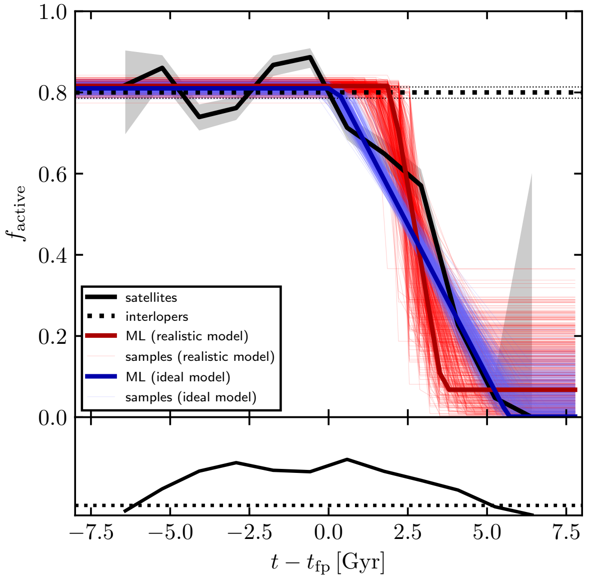


**Figure D4.** Identical to Fig. 7, reproduced here to facilitate comparison with Figs. D1–D3.

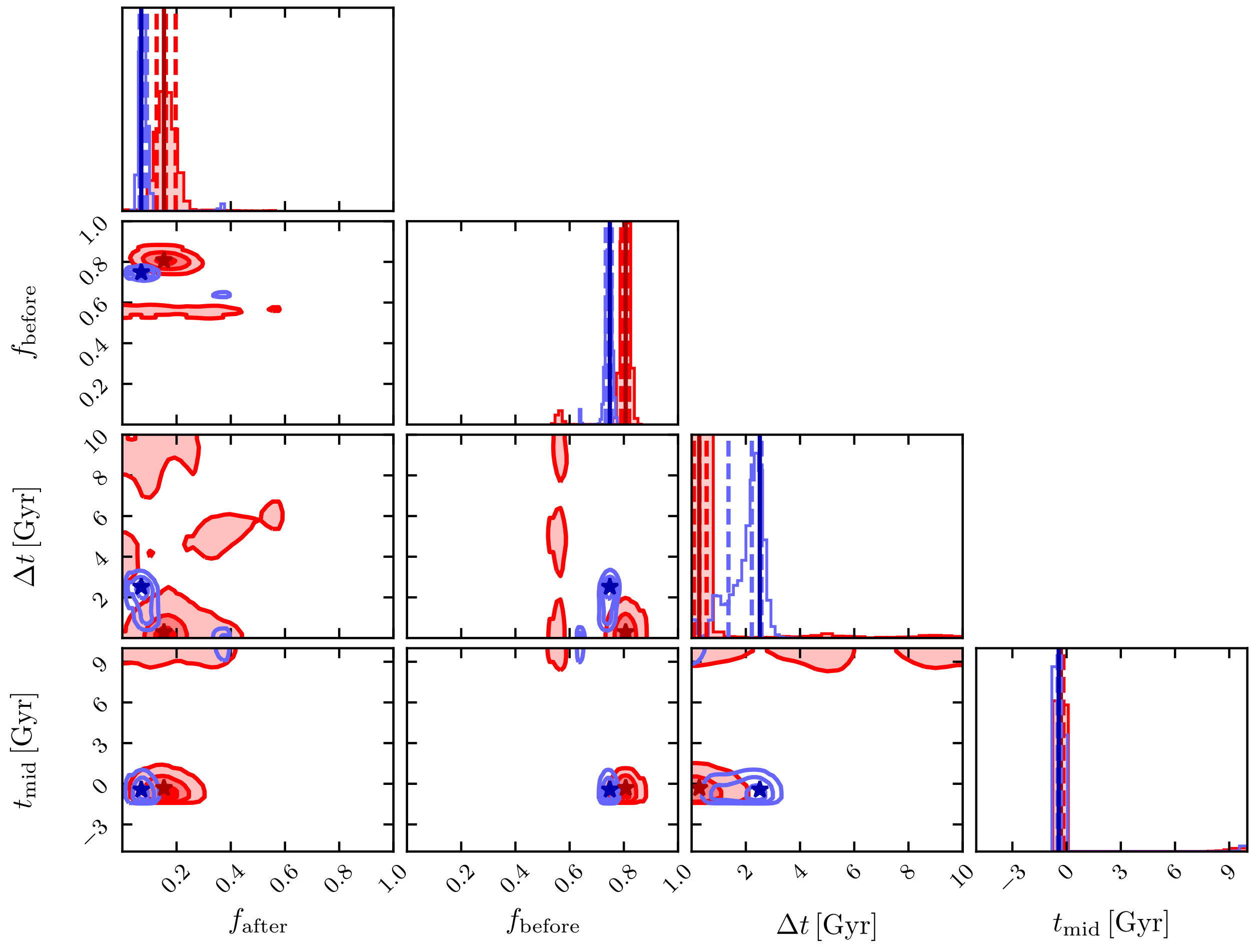


**Figure D5.** As Fig. 8, but for the first stellar mass bin (leftmost points in Fig. 9).

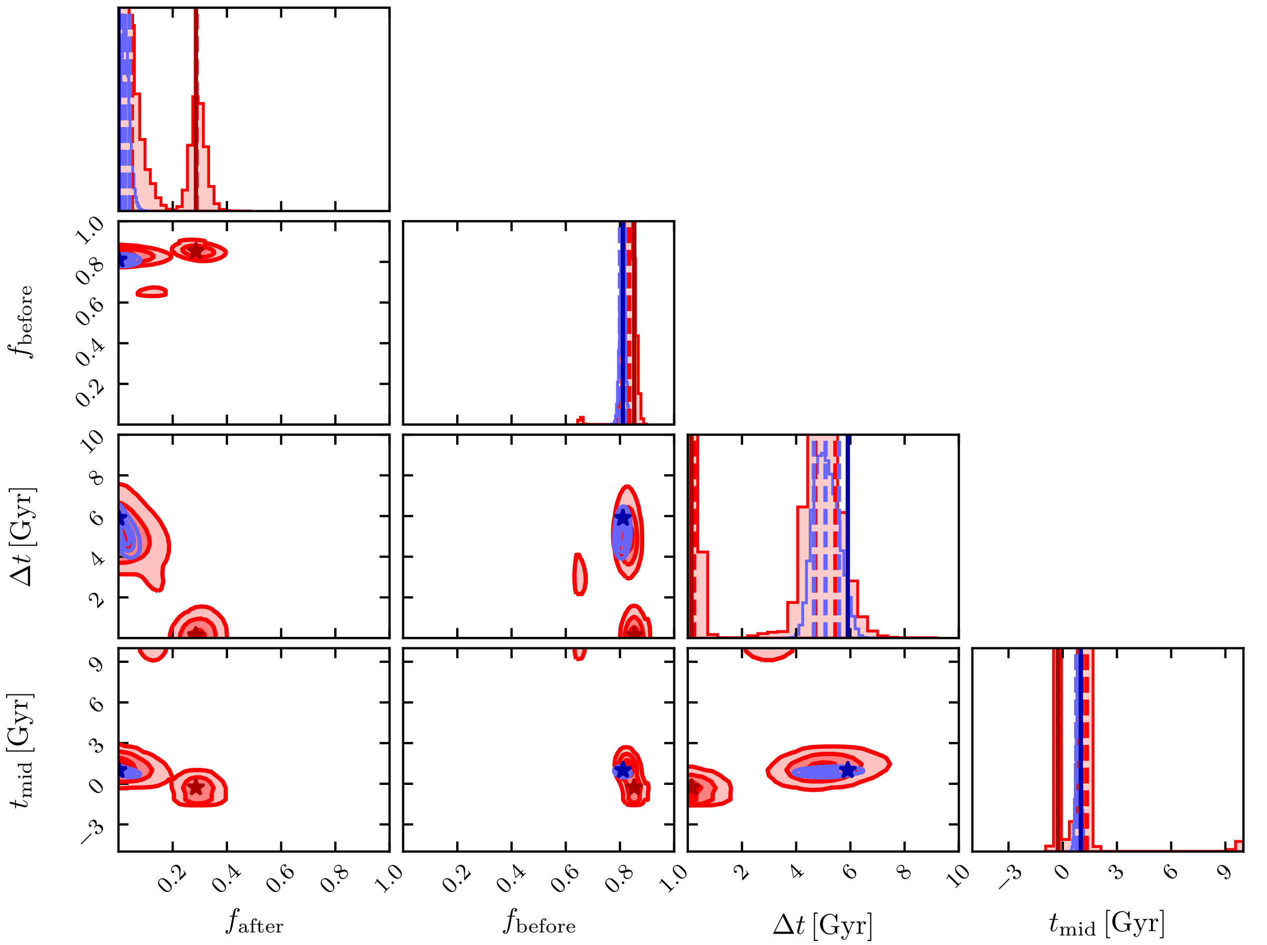


**Figure D6.** As Fig. 8, but for the second stellar mass bin (centre-left points in Fig. 9).

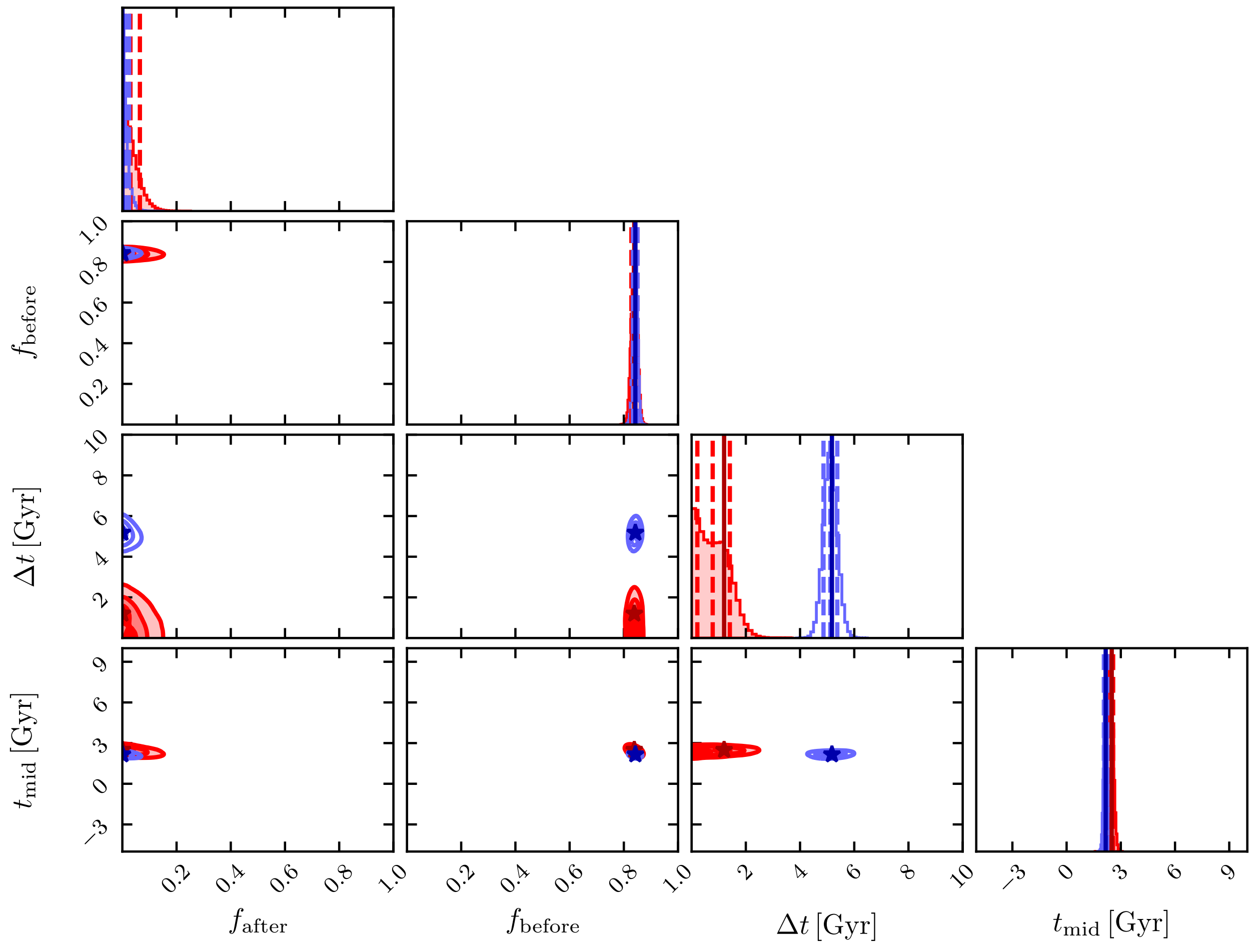


**Figure D7.** As Fig. 8, but for the third stellar mass bin (centre-right points in Fig. 9).

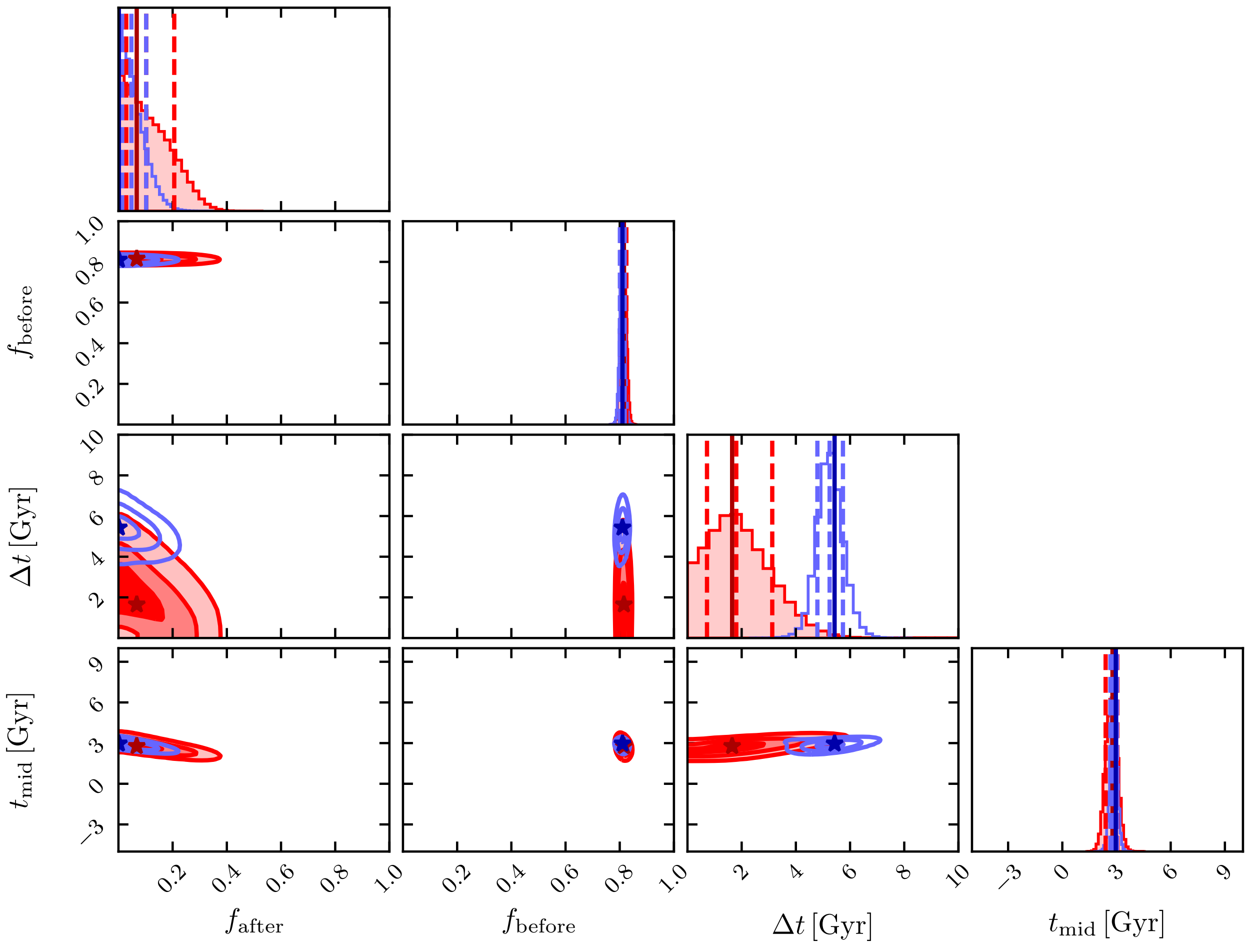


**Figure D8.** Identical to Fig. 8, reproduced here to facilitate comparison with Figs. D5–D7.

## APPENDIX E: TABLES OF MODEL PARAMETER CONSTRAINTS

© 0000 RAS, MNRAS **000**, 000–000



**Table E1.** Summary of model parameter constraints when $f_{\rm after}$ is fixed to 0. All quoted uncertainties are 16–84$^{\rm th}$ percentile confidence intervals. These are the values plotted in Figs. B1 and B2, and in Fig. 10, where $\Delta t$ is omitted. **(1)** Host mass interval; **(2)** median stellar mass; **(3–5)** $f_{\rm before}$, $t_{\rm mid}$ and $\Delta t$ for the $(g-r)$ colour analysis; **(6–8)** $f_{\rm before}$, $t_{\rm mid}$ and $\Delta t$ for the sSFR analysis; **(9–11)** $f_{\rm before}$, $t_{\rm mid}$ and $\Delta t$ for the gas analysis.

| | | $(g-r)$ | | | sSFR | | | gas | | |
|---|---|---|---|---|---|---|---|---|---|---|
| $M_{\rm host}$ [M$_\odot$] | $\log_{10}(M_\star/{\rm M}_\odot)$ | $f_{\rm before}$ | $t_{\rm mid}$ [Gyr] | $\Delta t$ [Gyr] | $f_{\rm before}$ | $t_{\rm mid}$ [Gyr] | $\Delta t$ [Gyr] | $f_{\rm before}$ | $t_{\rm mid}$ [Gyr] | $\Delta t$ [Gyr] |
| $10^{12}$–$10^{13}$ | 9.64 | $0.78^{+0.01}_{-0.01}$ | $9.5^{+0.4}_{-0.6}$ | $3.0^{+3.0}_{-2.1}$ | $0.69^{+0.01}_{-0.01}$ | $8.5^{+1.0}_{-1.1}$ | $4.5^{+3.5}_{-3.1}$ | $0.22^{+0.01}_{-0.01}$ | $5.8^{+2.1}_{-1.6}$ | $5.2^{+3.2}_{-3.5}$ |
| | 9.89 | $0.66^{+0.01}_{-0.01}$ | $9.1^{+0.7}_{-0.9}$ | $3.7^{+3.3}_{-2.5}$ | $0.59^{+0.01}_{-0.01}$ | $8.9^{+0.8}_{-1.0}$ | $3.9^{+3.5}_{-2.7}$ | $0.20^{+0.01}_{-0.01}$ | $4.6^{+1.7}_{-1.3}$ | $5.2^{+3.3}_{-3.5}$ |
| | 10.10 | $0.52^{+0.01}_{-0.01}$ | $9.0^{+0.7}_{-1.0}$ | $3.7^{+3.5}_{-2.6}$ | $0.50^{+0.01}_{-0.01}$ | $9.0^{+0.7}_{-1.0}$ | $3.7^{+3.5}_{-2.6}$ | $0.17^{+0.01}_{-0.01}$ | $5.6^{+2.2}_{-1.5}$ | $5.2^{+3.2}_{-3.5}$ |
| | 10.30 | $0.43^{+0.02}_{-0.02}$ | $7.7^{+1.4}_{-1.3}$ | $4.9^{+3.4}_{-3.4}$ | $0.43^{+0.01}_{-0.01}$ | $8.6^{+0.9}_{-1.2}$ | $4.2^{+3.6}_{-2.9}$ | $0.16^{+0.01}_{-0.01}$ | $6.9^{+2.0}_{-1.7}$ | $5.1^{+3.3}_{-3.5}$ |
| | 10.51 | $0.34^{+0.02}_{-0.02}$ | $7.0^{+1.7}_{-1.3}$ | $5.6^{+3.1}_{-3.6}$ | $0.35^{+0.02}_{-0.01}$ | $8.0^{+1.3}_{-1.4}$ | $4.8^{+3.5}_{-3.3}$ | $0.17^{+0.01}_{-0.01}$ | $7.1^{+1.8}_{-1.7}$ | $4.9^{+3.4}_{-3.3}$ |
| | 10.75 | $0.32^{+0.02}_{-0.02}$ | $7.5^{+1.6}_{-1.6}$ | $5.3^{+3.3}_{-3.5}$ | $0.30^{+0.02}_{-0.02}$ | $5.6^{+2.0}_{-1.2}$ | $6.8^{+2.3}_{-3.8}$ | $0.15^{+0.01}_{-0.01}$ | $8.3^{+1.2}_{-1.6}$ | $4.4^{+3.6}_{-3.1}$ |
| $10^{13}$–$10^{14}$ | 9.67 | $0.80^{+0.01}_{-0.01}$ | $6.2^{+0.3}_{-0.2}$ | $1.3^{+2.2}_{-0.9}$ | $0.71^{+0.01}_{-0.01}$ | $5.7^{+0.3}_{-0.2}$ | $1.8^{+2.1}_{-1.4}$ | $0.20^{+0.01}_{-0.01}$ | $2.0^{+1.0}_{-0.8}$ | $6.9^{+2.1}_{-4.0}$ |
| | 9.96 | $0.62^{+0.01}_{-0.01}$ | $5.7^{+0.3}_{-0.3}$ | $2.9^{+2.6}_{-2.1}$ | $0.56^{+0.01}_{-0.01}$ | $5.4^{+0.3}_{-0.3}$ | $2.9^{+2.2}_{-1.8}$ | $0.15^{+0.01}_{-0.01}$ | $3.4^{+0.9}_{-0.8}$ | $3.6^{+4.0}_{-2.6}$ |
| | 10.19 | $0.49^{+0.01}_{-0.01}$ | $5.6^{+0.4}_{-0.3}$ | $4.0^{+3.2}_{-2.6}$ | $0.47^{+0.01}_{-0.01}$ | $5.6^{+0.4}_{-0.3}$ | $3.5^{+3.0}_{-2.3}$ | $0.14^{+0.01}_{-0.01}$ | $2.2^{+0.9}_{-0.8}$ | $6.0^{+2.9}_{-3.9}$ |
| | 10.40 | $0.42^{+0.01}_{-0.01}$ | $5.6^{+0.4}_{-0.4}$ | $3.8^{+3.5}_{-2.5}$ | $0.42^{+0.01}_{-0.01}$ | $5.2^{+0.4}_{-0.4}$ | $3.4^{+3.1}_{-2.2}$ | $0.14^{+0.01}_{-0.01}$ | $3.7^{+1.0}_{-0.9}$ | $4.9^{+3.5}_{-3.3}$ |
| | 10.62 | $0.33^{+0.01}_{-0.01}$ | $5.4^{+0.6}_{-0.5}$ | $5.8^{+2.8}_{-3.5}$ | $0.34^{+0.01}_{-0.01}$ | $4.6^{+0.5}_{-0.4}$ | $4.4^{+3.0}_{-2.9}$ | $0.15^{+0.01}_{-0.01}$ | $3.4^{+0.8}_{-0.7}$ | $4.3^{+3.5}_{-2.9}$ |
| | 10.92 | $0.28^{+0.01}_{-0.01}$ | $4.3^{+0.6}_{-0.5}$ | $8.1^{+1.4}_{-2.3}$ | $0.23^{+0.01}_{-0.01}$ | $3.4^{+0.6}_{-0.5}$ | $8.7^{+0.9}_{-1.8}$ | $0.12^{+0.01}_{-0.01}$ | $6.4^{+2.1}_{-1.5}$ | $5.6^{+3.1}_{-3.7}$ |
| $10^{14}$–$10^{15}$ | 9.74 | $0.77^{+0.01}_{-0.01}$ | $4.3^{+0.2}_{-0.2}$ | $1.2^{+1.4}_{-0.8}$ | $0.70^{+0.01}_{-0.01}$ | $3.7^{+0.2}_{-0.2}$ | $1.3^{+1.3}_{-0.9}$ | $0.19^{+0.01}_{-0.01}$ | $-0.3^{+0.7}_{-0.6}$ | $4.3^{+3.6}_{-3.1}$ |
| | 10.09 | $0.64^{+0.01}_{-0.01}$ | $3.8^{+0.2}_{-0.2}$ | $0.8^{+0.9}_{-0.6}$ | $0.62^{+0.01}_{-0.01}$ | $3.2^{+0.2}_{-0.2}$ | $0.8^{+0.9}_{-0.6}$ | $0.15^{+0.01}_{-0.01}$ | $0.0^{+0.9}_{-0.8}$ | $5.8^{+2.9}_{-3.6}$ |
| | 10.33 | $0.51^{+0.01}_{-0.01}$ | $3.8^{+0.2}_{-0.2}$ | $1.0^{+1.1}_{-0.7}$ | $0.50^{+0.01}_{-0.01}$ | $3.4^{+0.2}_{-0.2}$ | $1.2^{+1.3}_{-0.8}$ | $0.13^{+0.01}_{-0.01}$ | $-0.8^{+0.6}_{-0.9}$ | $3.3^{+4.2}_{-2.5}$ |
| | 10.51 | $0.39^{+0.01}_{-0.01}$ | $4.0^{+0.3}_{-0.3}$ | $4.3^{+2.0}_{-2.3}$ | $0.38^{+0.01}_{-0.01}$ | $4.1^{+0.3}_{-0.3}$ | $1.9^{+1.9}_{-1.3}$ | $0.14^{+0.01}_{-0.01}$ | $-0.5^{+0.9}_{-1.1}$ | $6.3^{+2.7}_{-3.9}$ |
| | 10.69 | $0.32^{+0.01}_{-0.01}$ | $4.4^{+0.3}_{-0.3}$ | $3.9^{+2.7}_{-2.5}$ | $0.32^{+0.01}_{-0.01}$ | $3.5^{+0.3}_{-0.3}$ | $4.8^{+2.8}_{-2.7}$ | $0.13^{+0.01}_{-0.01}$ | $1.3^{+1.0}_{-1.0}$ | $5.8^{+2.9}_{-3.6}$ |
| | 10.95 | $0.24^{+0.01}_{-0.01}$ | $4.6^{+0.5}_{-0.4}$ | $5.6^{+2.3}_{-2.2}$ | $0.19^{+0.01}_{-0.01}$ | $4.7^{+0.6}_{-0.5}$ | $6.7^{+2.1}_{-2.5}$ | $0.13^{+0.01}_{-0.01}$ | $2.3^{+1.0}_{-0.9}$ | $5.6^{+3.1}_{-3.7}$ |

**Table E2.** Summary of model parameter constraints when $f_{\rm after}$ is a free paramter. All quoted uncertainties are 16–84$^{\rm th}$ percentile confidence intervals. These are the values plotted in Figs. B3 and B4. **(1)** Host mass interval; **(2)** median stellar mass; **(3–6)** $f_{\rm before}$, $f_{\rm after}$, $t_{\rm mid}$ and $\Delta t$ for the $(g-r)$ colour analysis; **(7–10)** $f_{\rm before}$, $f_{\rm after}$, $t_{\rm mid}$ and $\Delta t$ for the sSFR analysis; **(11–14)** $f_{\rm before}$, $f_{\rm after}$, $t_{\rm mid}$ and $\Delta t$ for the gas analysis.

| | | $(g-r)$ | | | | sSFR | | | | gas | | | |
|---|---|---|---|---|---|---|---|---|---|---|---|---|---|
| $M_{\rm host}$ [$M_\odot$] | $\log_{10}(M_\star/M_\odot)$ | $f_{\rm before}$ | $f_{\rm after}$ | $t_{\rm mid}$ [Gyr] | $\Delta t$ [Gyr] | $f_{\rm before}$ | $f_{\rm after}$ | $t_{\rm mid}$ [Gyr] | $\Delta t$ [Gyr] | $f_{\rm before}$ | $f_{\rm after}$ | $t_{\rm mid}$ [Gyr] | $\Delta t$ [Gyr] |
| | 9.64 | $0.77^{+0.01}_{-0.01}$ | $0.66^{+0.09}_{-0.29}$ | $8.3^{+1.3}_{-3.9}$ | $4.4^{+3.5}_{-3.0}$ | $0.69^{+0.01}_{-0.01}$ | $0.46^{+0.16}_{-0.27}$ | $6.7^{+2.1}_{-3.7}$ | $5.0^{+3.4}_{-3.4}$ | $0.22^{+0.02}_{-0.01}$ | $0.12^{+0.06}_{-0.07}$ | $3.7^{+3.1}_{-4.1}$ | $5.0^{+3.4}_{-3.4}$ |
| | 9.89 | $0.66^{+0.01}_{-0.01}$ | $0.49^{+0.14}_{-0.28}$ | $7.8^{+1.6}_{-3.8}$ | $4.6^{+3.5}_{-3.2}$ | $0.58^{+0.01}_{-0.01}$ | $0.42^{+0.13}_{-0.25}$ | $7.6^{+1.7}_{-3.8}$ | $4.6^{+3.5}_{-3.1}$ | $0.20^{+0.02}_{-0.01}$ | $0.09^{+0.05}_{-0.06}$ | $2.2^{+2.7}_{-4.3}$ | $5.1^{+3.3}_{-3.5}$ |
| $10^{12}$–$10^{13}$ | 10.10 | $0.51^{+0.01}_{-0.01}$ | $0.39^{+0.10}_{-0.22}$ | $7.6^{+1.7}_{-4.5}$ | $4.6^{+3.5}_{-3.2}$ | $0.50^{+0.01}_{-0.01}$ | $0.37^{+0.10}_{-0.21}$ | $7.6^{+1.7}_{-4.1}$ | $4.7^{+3.5}_{-3.2}$ | $0.17^{+0.01}_{-0.01}$ | $0.08^{+0.05}_{-0.05}$ | $3.9^{+3.0}_{-3.2}$ | $4.9^{+3.4}_{-3.4}$ |
| | 10.30 | $0.43^{+0.02}_{-0.02}$ | $0.28^{+0.10}_{-0.17}$ | $5.6^{+2.7}_{-4.4}$ | $5.1^{+3.3}_{-3.4}$ | $0.43^{+0.01}_{-0.01}$ | $0.32^{+0.08}_{-0.18}$ | $6.9^{+2.2}_{-4.6}$ | $4.9^{+3.5}_{-3.3}$ | $0.16^{+0.01}_{-0.01}$ | $0.10^{+0.04}_{-0.06}$ | $4.8^{+3.2}_{-4.3}$ | $5.1^{+3.4}_{-3.4}$ |
| | 10.51 | $0.34^{+0.02}_{-0.02}$ | $0.21^{+0.08}_{-0.13}$ | $4.3^{+3.1}_{-4.5}$ | $5.3^{+3.2}_{-3.6}$ | $0.35^{+0.02}_{-0.01}$ | $0.24^{+0.07}_{-0.15}$ | $5.8^{+2.7}_{-5.4}$ | $4.9^{+3.4}_{-3.3}$ | $0.17^{+0.01}_{-0.01}$ | $0.10^{+0.04}_{-0.07}$ | $5.3^{+3.0}_{-4.5}$ | $5.0^{+3.4}_{-3.4}$ |
| | 10.75 | $0.32^{+0.02}_{-0.02}$ | $0.23^{+0.06}_{-0.12}$ | $4.2^{+3.6}_{-4.4}$ | $5.2^{+3.3}_{-3.5}$ | $0.30^{+0.02}_{-0.02}$ | $0.16^{+0.06}_{-0.09}$ | $3.0^{+2.5}_{-1.9}$ | $4.6^{+3.6}_{-3.3}$ | $0.15^{+0.01}_{-0.01}$ | $0.11^{+0.03}_{-0.06}$ | $6.6^{+2.4}_{-5.1}$ | $4.8^{+3.5}_{-3.3}$ |
| | 9.67 | $0.80^{+0.01}_{-0.01}$ | $0.07^{+0.09}_{-0.05}$ | $6.0^{+0.3}_{-0.3}$ | $1.3^{+2.2}_{-1.0}$ | $0.71^{+0.01}_{-0.01}$ | $0.06^{+0.09}_{-0.04}$ | $5.5^{+0.3}_{-0.4}$ | $1.9^{+1.9}_{-1.3}$ | $0.21^{+0.01}_{-0.01}$ | $0.05^{+0.03}_{-0.03}$ | $-0.2^{+1.9}_{-1.4}$ | $5.1^{+3.4}_{-3.9}$ |
| | 9.96 | $0.62^{+0.01}_{-0.01}$ | $0.07^{+0.09}_{-0.05}$ | $5.3^{+0.4}_{-0.6}$ | $2.8^{+2.4}_{-1.8}$ | $0.56^{+0.01}_{-0.01}$ | $0.06^{+0.07}_{-0.04}$ | $5.0^{+0.4}_{-0.6}$ | $2.5^{+2.2}_{-1.7}$ | $0.15^{+0.01}_{-0.01}$ | $0.02^{+0.03}_{-0.02}$ | $2.5^{+1.3}_{-2.1}$ | $4.5^{+3.6}_{-3.1}$ |
| $10^{13}$–$10^{14}$ | 10.19 | $0.49^{+0.01}_{-0.01}$ | $0.11^{+0.11}_{-0.08}$ | $4.8^{+0.7}_{-1.5}$ | $3.7^{+3.7}_{-2.6}$ | $0.47^{+0.01}_{-0.01}$ | $0.07^{+0.08}_{-0.05}$ | $5.1^{+0.6}_{-0.8}$ | $3.2^{+3.1}_{-2.1}$ | $0.14^{+0.01}_{-0.01}$ | $0.04^{+0.01}_{-0.02}$ | $-1.1^{+2.4}_{-2.5}$ | $5.5^{+3.1}_{-3.6}$ |
| | 10.40 | $0.42^{+0.01}_{-0.01}$ | $0.08^{+0.09}_{-0.06}$ | $5.0^{+0.7}_{-1.2}$ | $3.8^{+3.6}_{-2.6}$ | $0.43^{+0.01}_{-0.01}$ | $0.06^{+0.07}_{-0.04}$ | $4.6^{+0.6}_{-0.9}$ | $3.4^{+3.4}_{-2.3}$ | $0.14^{+0.01}_{-0.01}$ | $0.04^{+0.03}_{-0.03}$ | $1.7^{+1.8}_{-3.4}$ | $5.0^{+3.4}_{-3.4}$ |
| | 10.62 | $0.33^{+0.01}_{-0.01}$ | $0.09^{+0.07}_{-0.06}$ | $4.2^{+1.0}_{-1.5}$ | $4.8^{+3.3}_{-3.2}$ | $0.34^{+0.01}_{-0.01}$ | $0.06^{+0.05}_{-0.04}$ | $3.9^{+0.7}_{-0.9}$ | $3.4^{+3.2}_{-2.4}$ | $0.15^{+0.01}_{-0.01}$ | $0.03^{+0.03}_{-0.02}$ | $2.4^{+1.1}_{-1.4}$ | $4.2^{+3.6}_{-2.9}$ |
| | 10.92 | $0.29^{+0.01}_{-0.01}$ | $0.13^{+0.04}_{-0.06}$ | $1.6^{+1.6}_{-1.7}$ | $5.4^{+3.2}_{-3.4}$ | $0.23^{+0.01}_{-0.01}$ | $0.10^{+0.02}_{-0.03}$ | $0.4^{+1.2}_{-1.2}$ | $3.8^{+3.5}_{-2.7}$ | $0.12^{+0.01}_{-0.01}$ | $0.08^{+0.02}_{-0.05}$ | $3.3^{+3.5}_{-4.2}$ | $5.2^{+3.3}_{-3.5}$ |
| | 9.74 | $0.77^{+0.01}_{-0.01}$ | $0.02^{+0.03}_{-0.02}$ | $4.2^{+0.2}_{-0.2}$ | $1.2^{+1.3}_{-0.8}$ | $0.70^{+0.01}_{-0.01}$ | $0.01^{+0.02}_{-0.01}$ | $3.6^{+0.2}_{-0.2}$ | $1.3^{+1.4}_{-0.9}$ | $0.19^{+0.01}_{-0.01}$ | $0.02^{+0.02}_{-0.01}$ | $-1.1^{+0.8}_{-1.1}$ | $2.9^{+4.0}_{-2.1}$ |
| | 10.09 | $0.64^{+0.01}_{-0.01}$ | $0.01^{+0.01}_{-0.01}$ | $3.7^{+0.2}_{-0.2}$ | $0.8^{+0.9}_{-0.6}$ | $0.62^{+0.01}_{-0.01}$ | $0.01^{+0.01}_{-0.00}$ | $3.2^{+0.2}_{-0.2}$ | $0.8^{+0.9}_{-0.6}$ | $0.15^{+0.01}_{-0.01}$ | $0.02^{+0.01}_{-0.01}$ | $-1.3^{+1.2}_{-1.8}$ | $4.7^{+3.5}_{-3.2}$ |
| $10^{14}$–$10^{15}$ | 10.33 | $0.51^{+0.01}_{-0.01}$ | $0.01^{+0.01}_{-0.01}$ | $3.7^{+0.2}_{-0.2}$ | $1.0^{+1.1}_{-0.7}$ | $0.50^{+0.01}_{-0.01}$ | $0.01^{+0.02}_{-0.01}$ | $3.3^{+0.2}_{-0.3}$ | $1.2^{+1.3}_{-0.8}$ | $0.13^{+0.01}_{-0.01}$ | $0.01^{+0.01}_{-0.01}$ | $-1.3^{+0.8}_{-1.5}$ | $3.3^{+4.0}_{-2.4}$ |
| | 10.51 | $0.39^{+0.01}_{-0.01}$ | $0.04^{+0.03}_{-0.03}$ | $3.4^{+0.5}_{-0.6}$ | $2.6^{+2.5}_{-1.9}$ | $0.38^{+0.01}_{-0.01}$ | $0.02^{+0.02}_{-0.01}$ | $3.8^{+0.4}_{-0.4}$ | $1.7^{+1.8}_{-1.2}$ | $0.14^{+0.01}_{-0.01}$ | $0.01^{+0.01}_{-0.01}$ | $-2.2^{+1.7}_{-1.8}$ | $5.4^{+3.2}_{-3.7}$ |
| | 10.69 | $0.32^{+0.01}_{-0.01}$ | $0.03^{+0.03}_{-0.02}$ | $3.9^{+0.5}_{-0.6}$ | $3.1^{+2.7}_{-2.2}$ | $0.32^{+0.01}_{-0.01}$ | $0.02^{+0.03}_{-0.02}$ | $3.1^{+0.5}_{-0.6}$ | $4.5^{+2.9}_{-2.7}$ | $0.13^{+0.01}_{-0.01}$ | $0.02^{+0.02}_{-0.02}$ | $-0.8^{+1.8}_{-2.5}$ | $5.4^{+3.2}_{-3.6}$ |
| | 10.95 | $0.24^{+0.01}_{-0.01}$ | $0.06^{+0.03}_{-0.04}$ | $3.4^{+0.9}_{-0.8}$ | $3.2^{+3.0}_{-2.3}$ | $0.19^{+0.01}_{-0.01}$ | $0.06^{+0.03}_{-0.04}$ | $3.2^{+1.2}_{-1.0}$ | $4.1^{+3.5}_{-2.9}$ | $0.13^{+0.01}_{-0.01}$ | $0.03^{+0.02}_{-0.02}$ | $0.3^{+1.6}_{-1.8}$ | $4.7^{+3.5}_{-3.2}$ |

## APPENDIX F: MARGINALIZED POSTERIOR PROBABILITY DISTRIBUTIONS OF MODEL PARAMETERS

© 0000 RAS, MNRAS **000**, 000–000

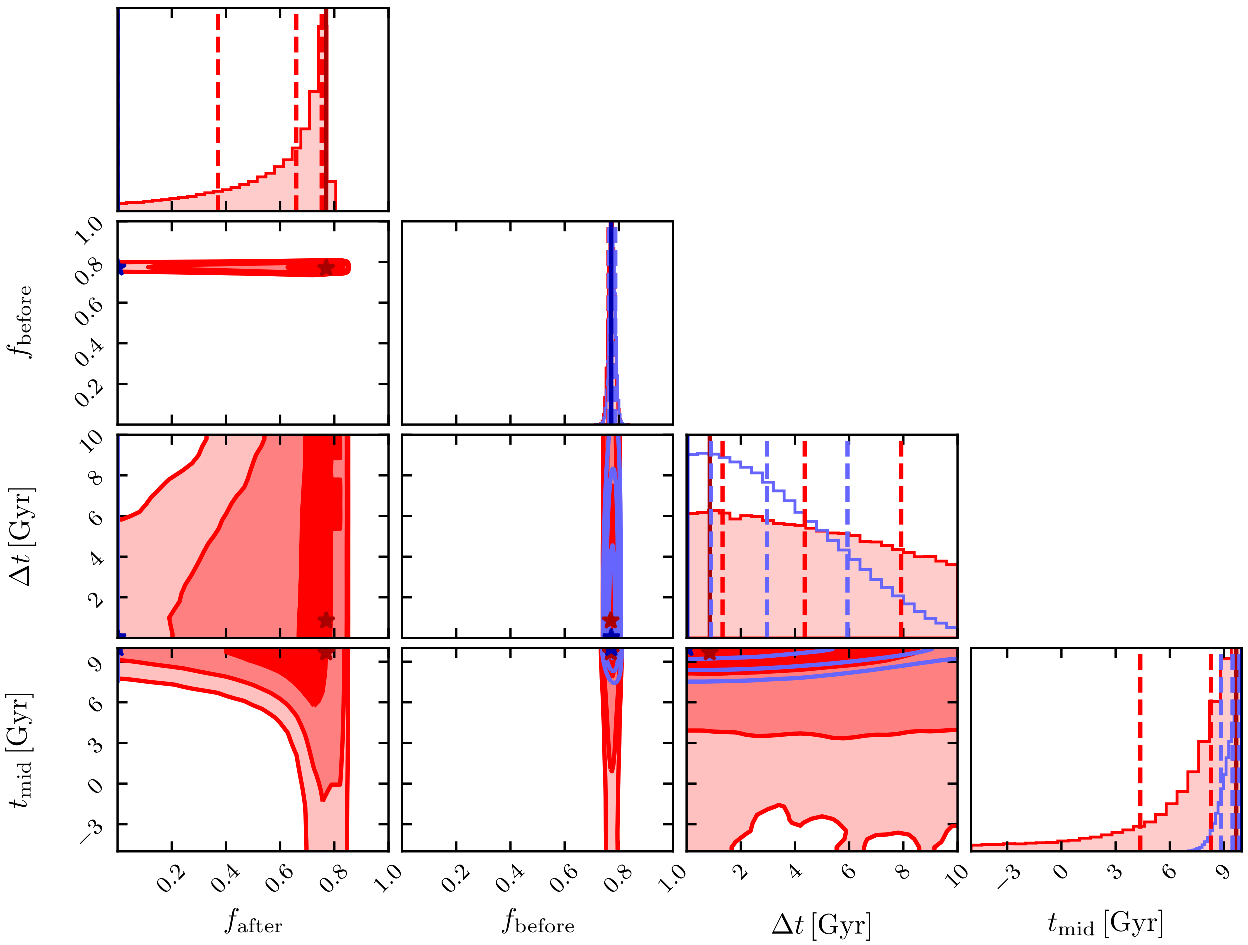


**Figure F1.** One- and two-dimensional marginalized posterior probability distributions for the parameters of the model defined in Sec. 4 constrained by the $(g-r)$ colour sample for the first stellar mass bin of the $10^{12} < M_{\rm host}/{\rm M}_\odot < 10^{13}$ sample. Open blue contours/histograms are for the fiducial case where $f_{\rm after}$ is fixed to 0 (as in Figs. 10, B1 and B2), while filled red contours/histograms are for the case where $f_{\rm after}$ is a free parameter (as in Figs. B3 and B4). Contours are drawn at 68, 95 and 99 per cent confidence intervals, and dashed lines are drawn at the $16^{\rm th}$, $50^{\rm th}$ and $84^{\rm th}$ percentiles. The stars and solid lines mark the position of the maximum likelihood parameter sample drawn in the Markov chain.

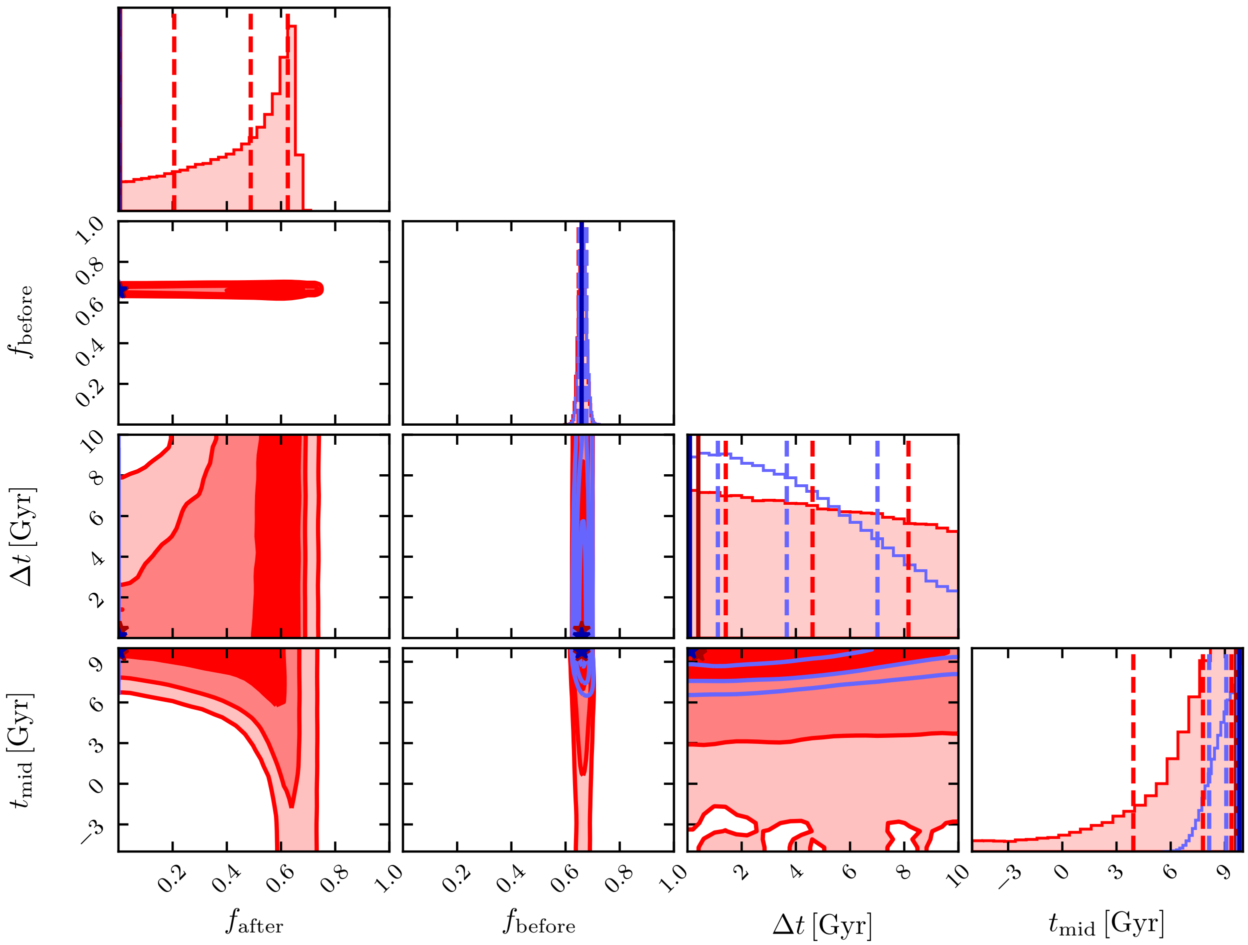


**Figure F2.** As in Fig. F1, but for the $(g-r)$ colour analysis of the $10^{12} < M_{\rm host}/{\rm M}_{\odot} < 10^{13}$ sample, second stellar mass bin.

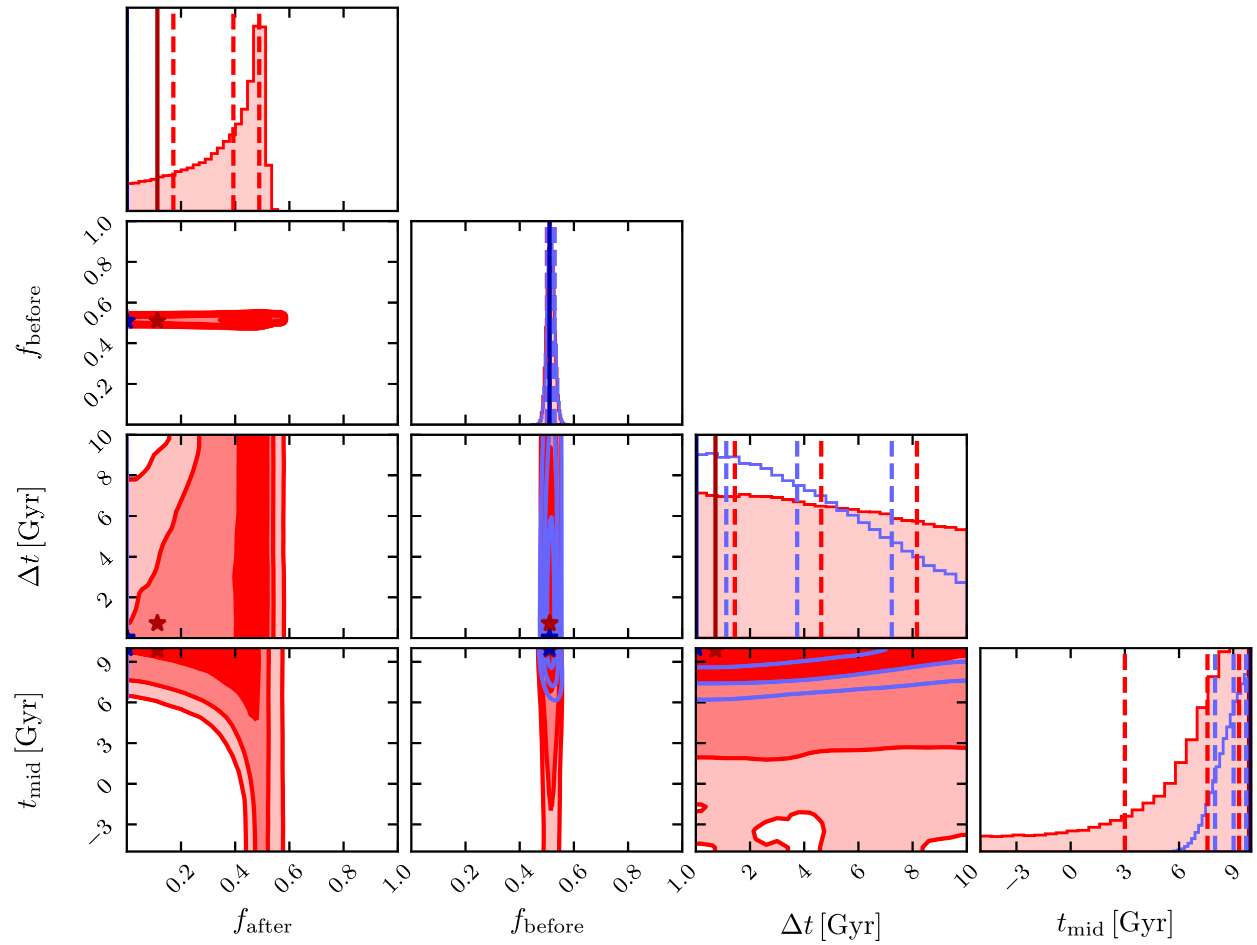


**Figure F3.** As in Fig. F1, but for the $(g - r)$ colour analysis of the $10^{12} < M_{\rm host}/{\rm M}_{\odot} < 10^{13}$ sample, third stellar mass bin.

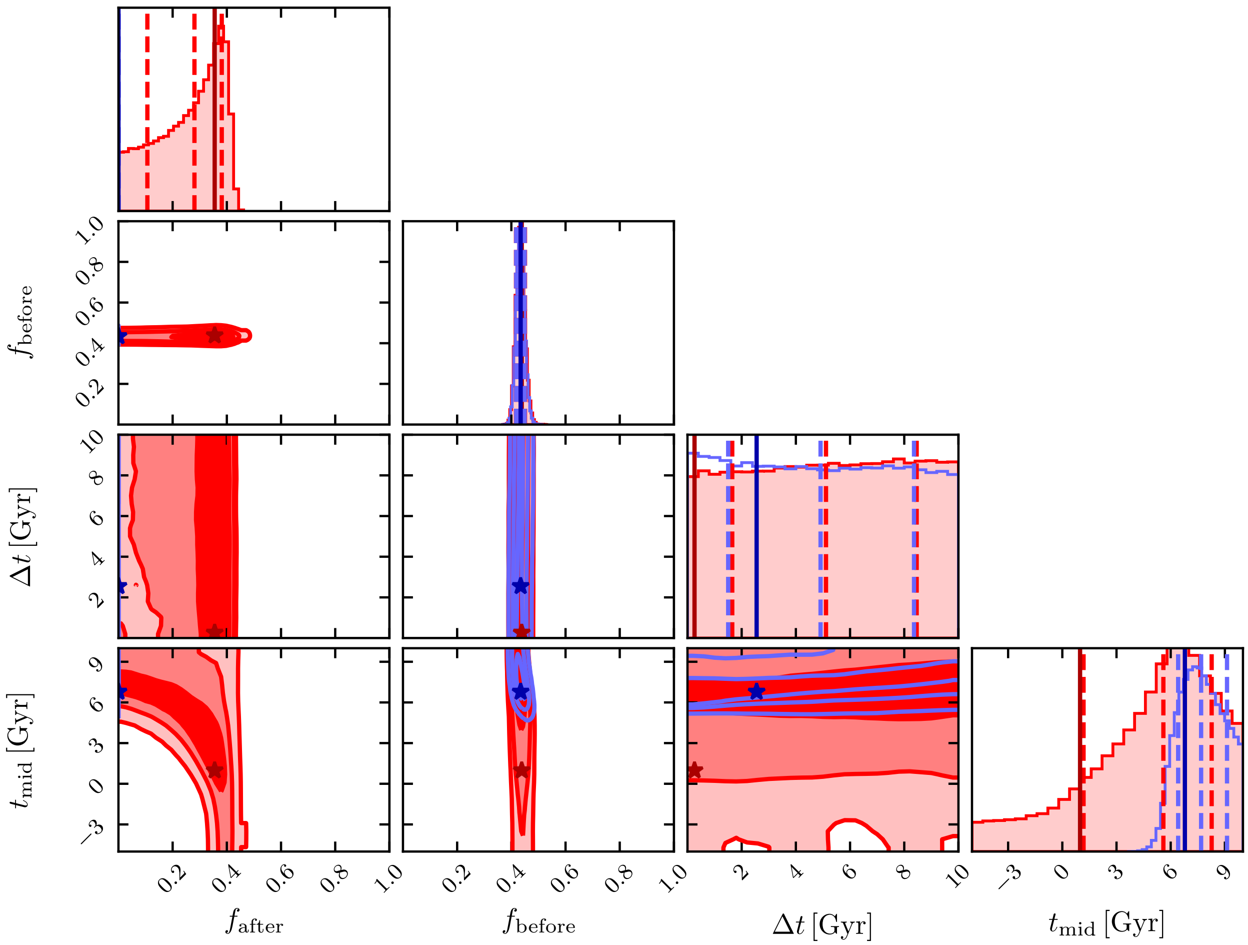


**Figure F4.** As in Fig. F1, but for the $(g-r)$ colour analysis of the $10^{12} < M_{\rm host}/{\rm M}_{\odot} < 10^{13}$ sample, fourth stellar mass bin.

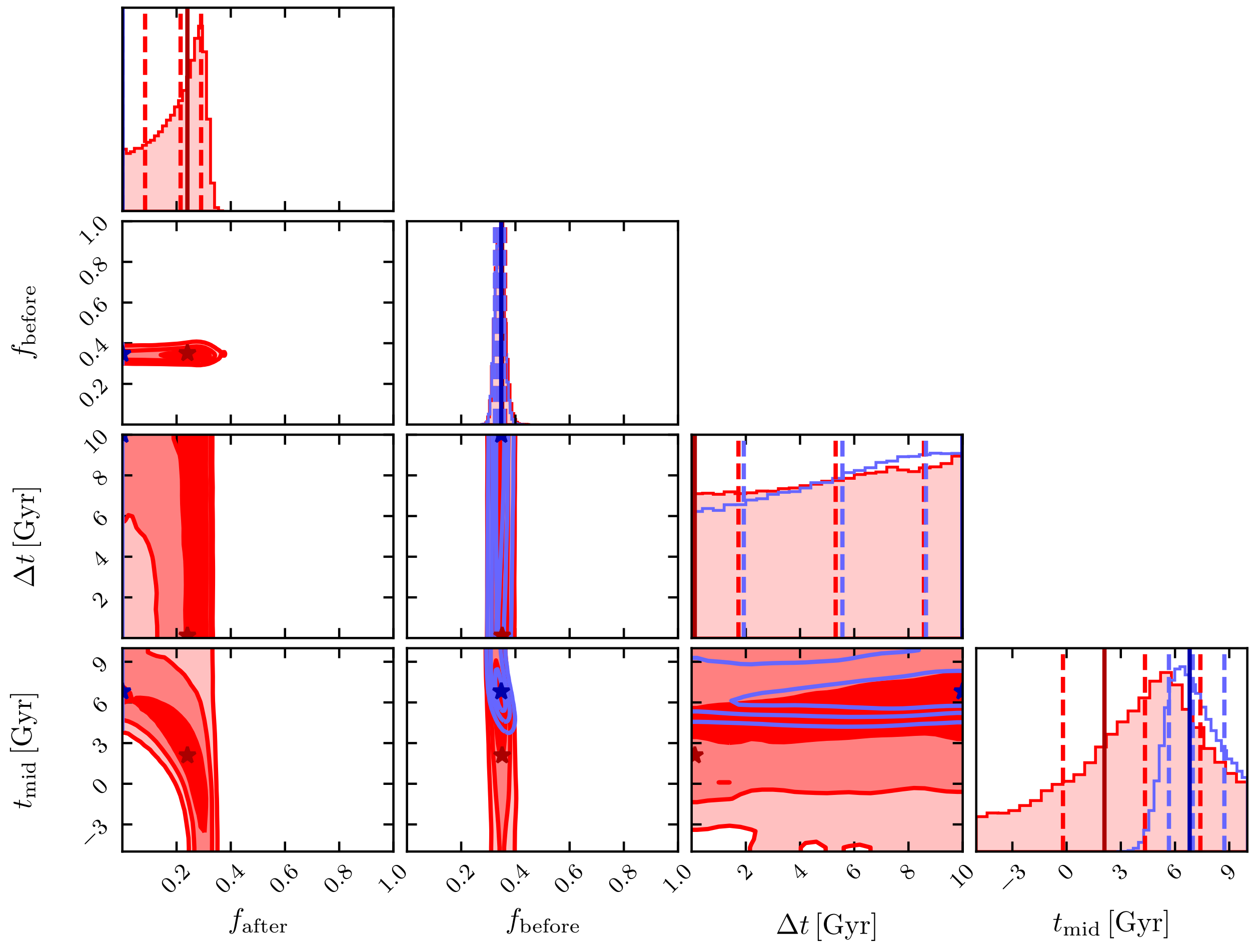


**Figure F5.** As in Fig. F1, but for the $(g-r)$ colour analysis of the $10^{12} < M_{\rm host}/{\rm M}_\odot < 10^{13}$ sample, fifth stellar mass bin.

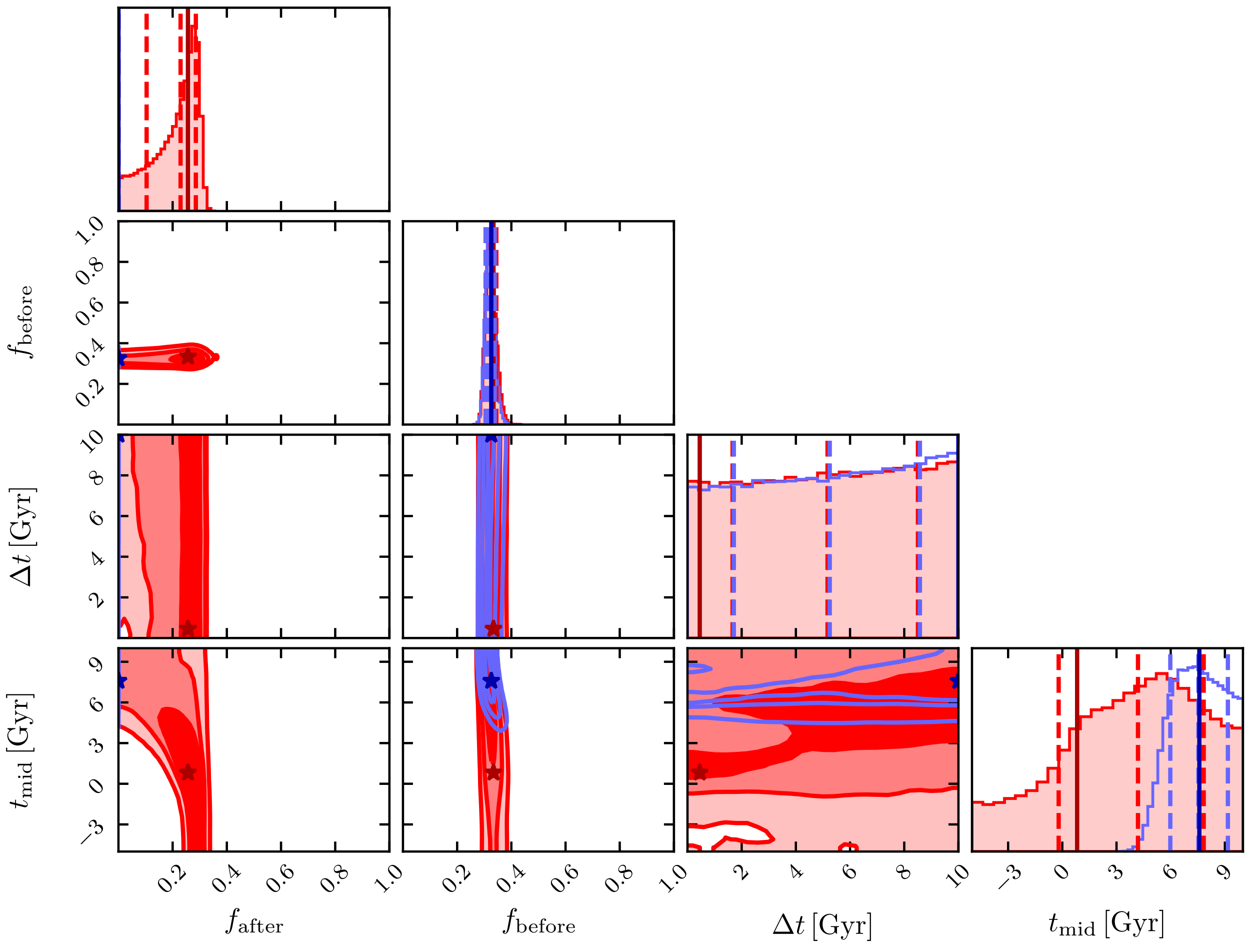


**Figure F6.** As in Fig. F1, but for the $(g-r)$ colour analysis of the $10^{12} < M_{\mathrm{host}}/\mathrm{M}_{\odot} < 10^{13}$ sample, sixth stellar mass bin.

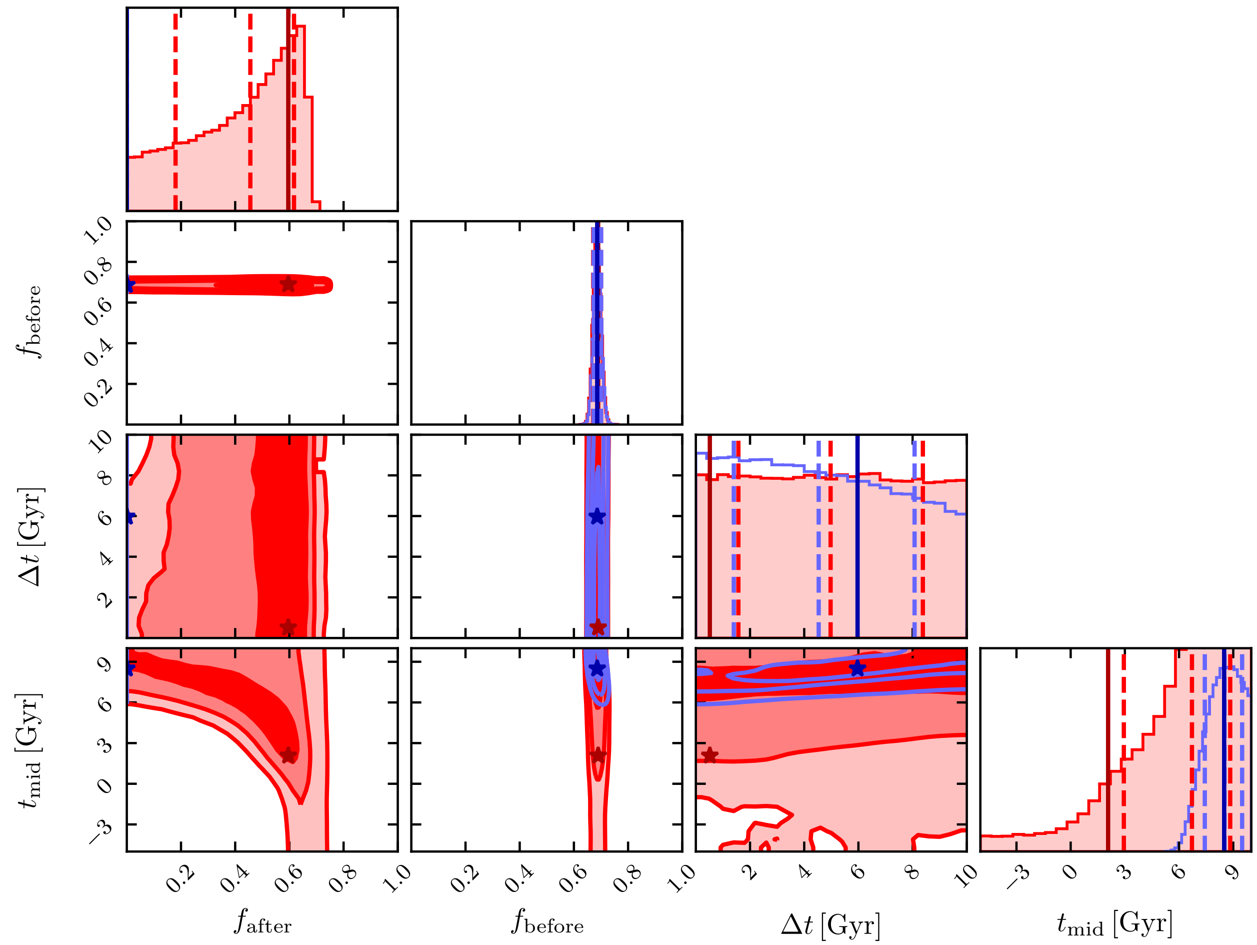


**Figure F7.** As in Fig. F1, but for the SSFR analysis of the $10^{12} < M_{\rm host}/{\rm M}_{\odot} < 10^{13}$ sample, first stellar mass bin.

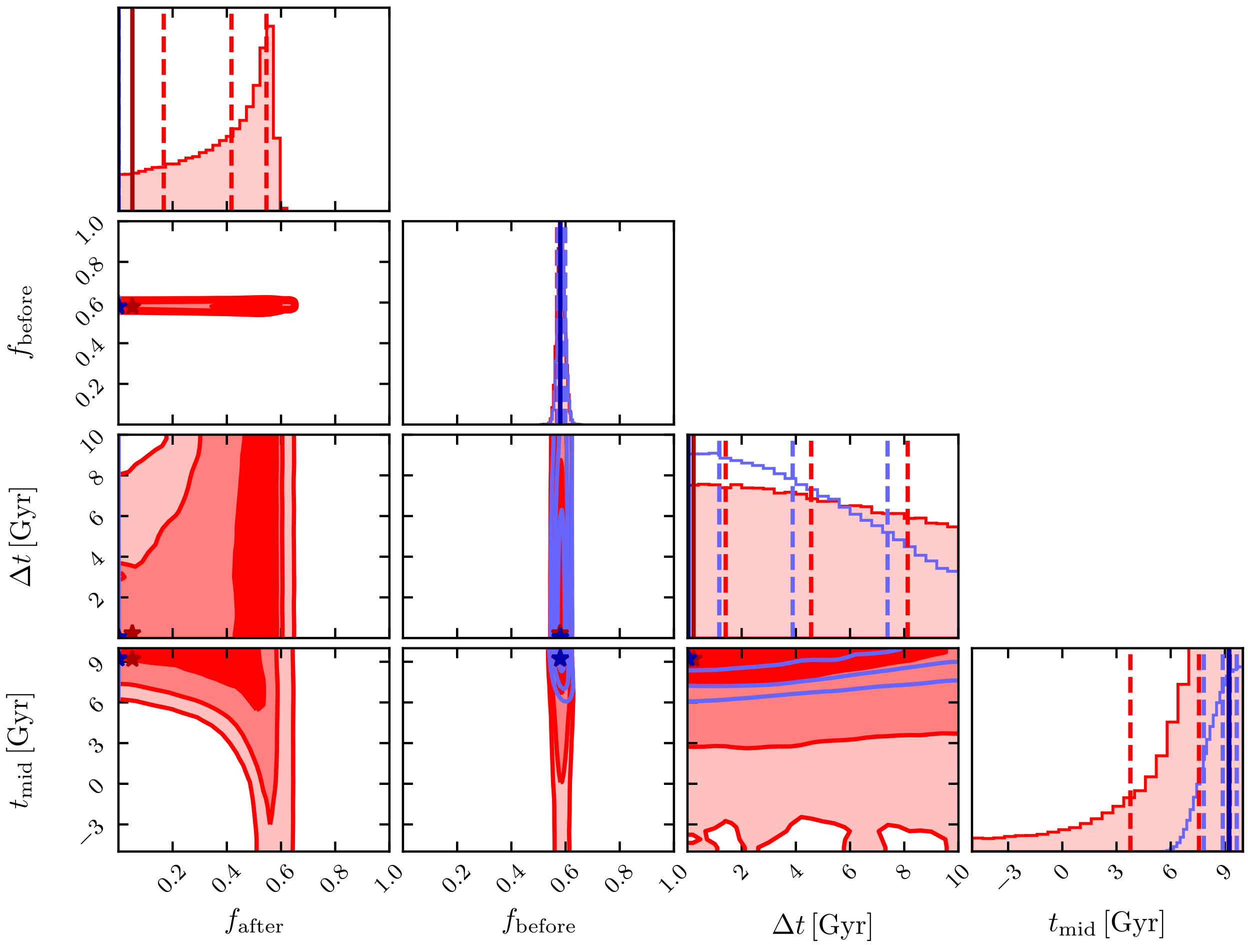


**Figure F8.** As in Fig. F1, but for the SSFR analysis of the $10^{12} < M_{\rm host}/{\rm M}_{\odot} < 10^{13}$ sample, second stellar mass bin.

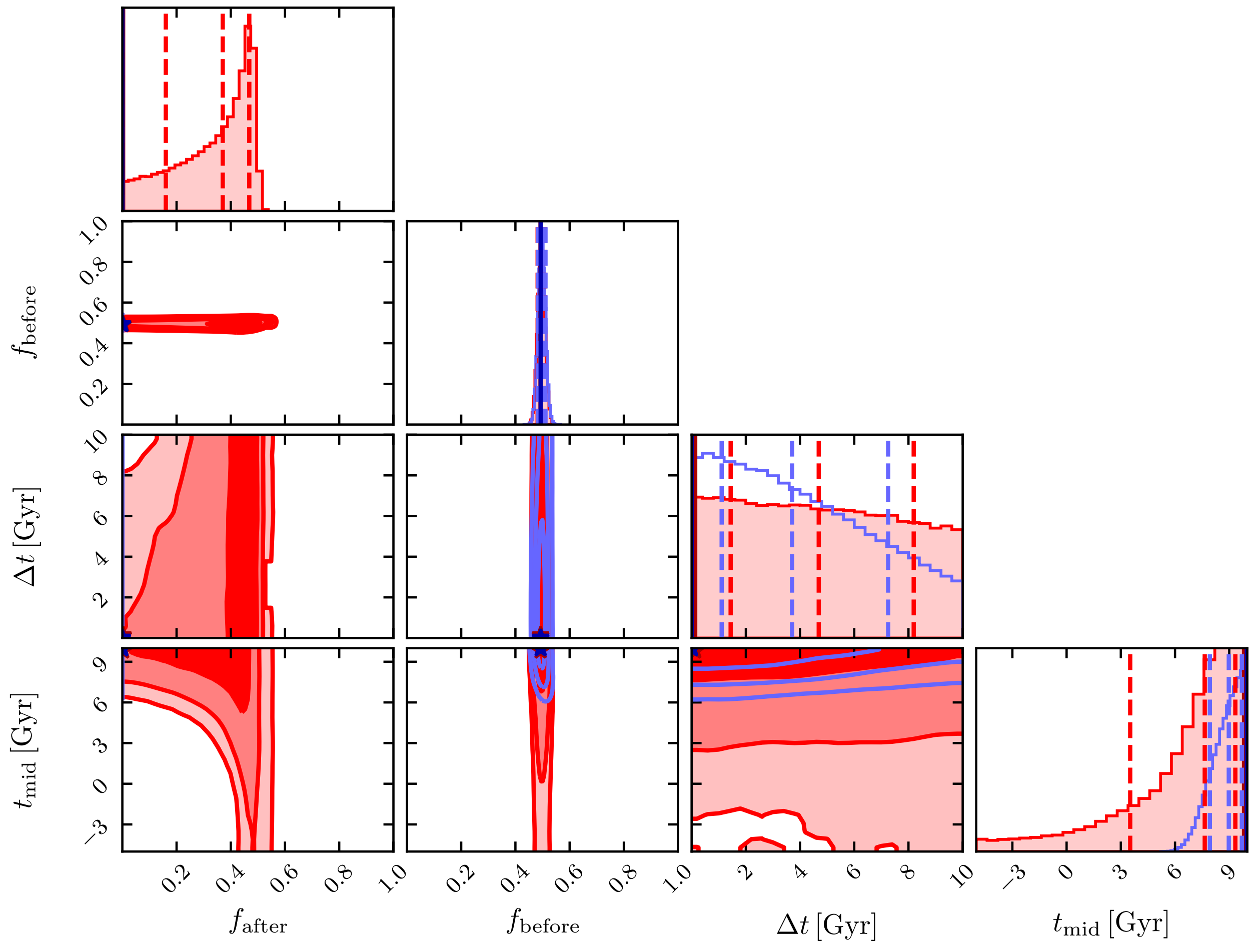


**Figure F9.** As in Fig. F1, but for the SSFR analysis of the $10^{12} < M_{\rm host}/{\rm M}_{\odot} < 10^{13}$ sample, third stellar mass bin.

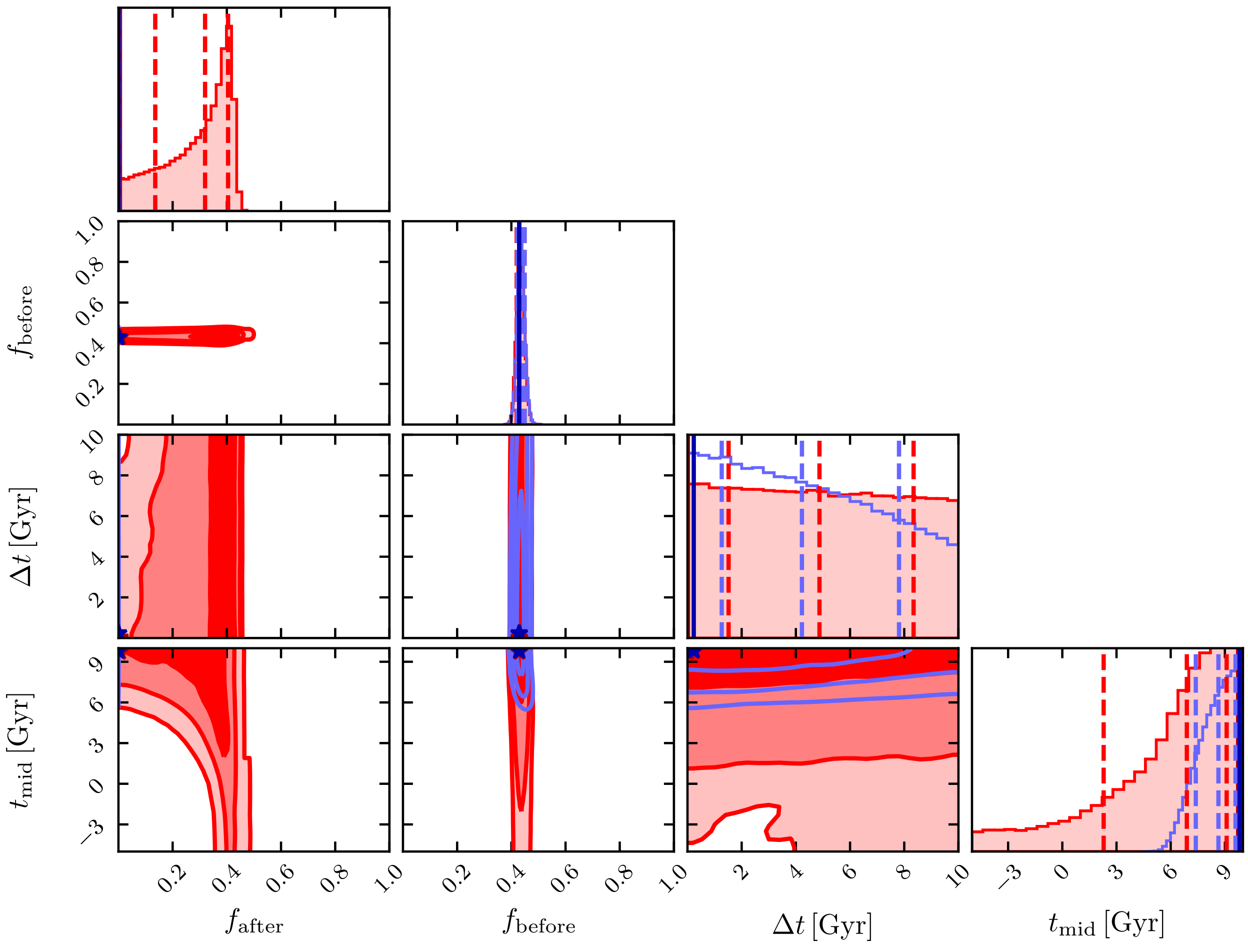


**Figure F10.** As in Fig. F1, but for the SSFR analysis of the $10^{12} < M_{\rm host}/{\rm M}_{\odot} < 10^{13}$ sample, fourth stellar mass bin.

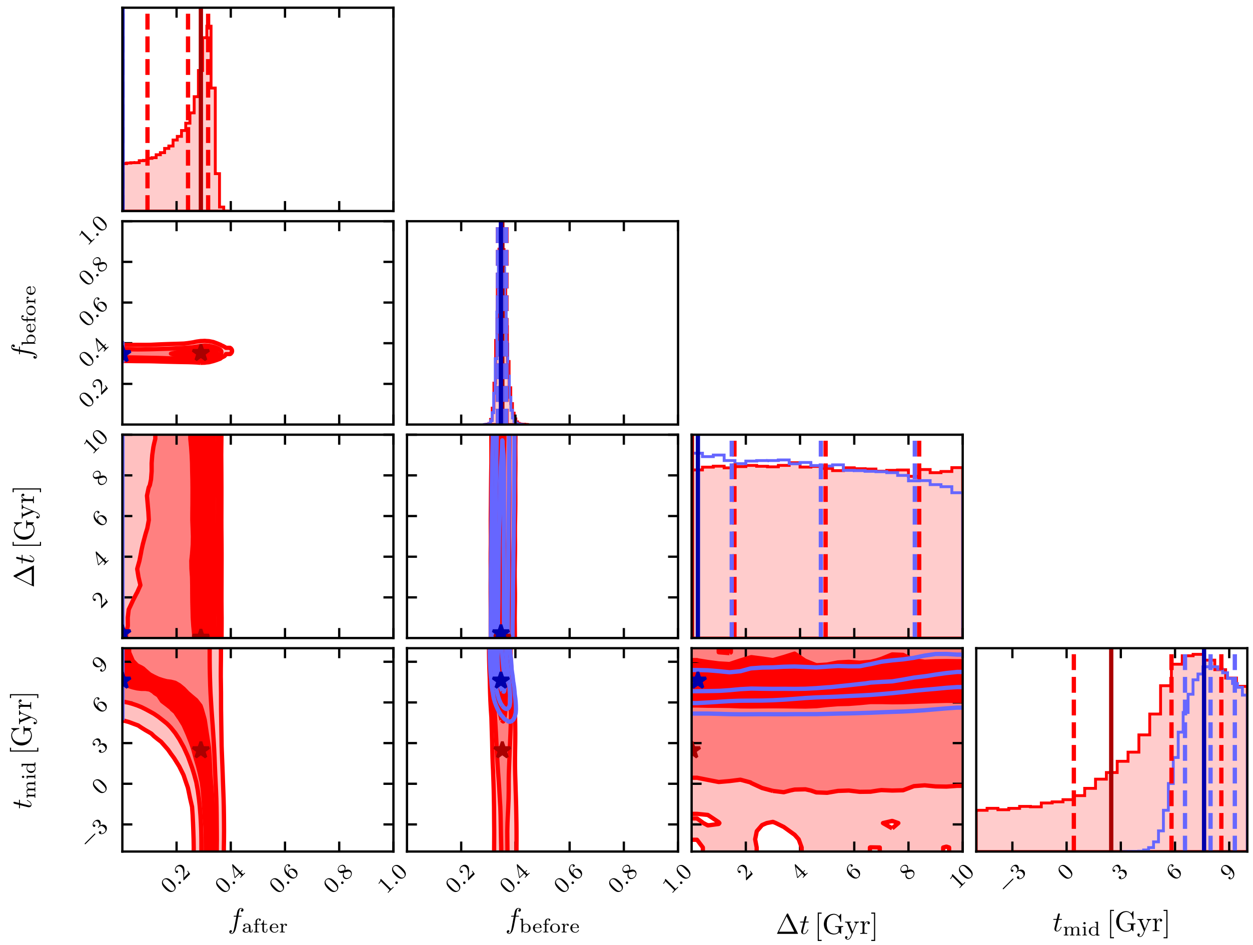


**Figure F11.** As in Fig. F1, but for the SSFR analysis of the $10^{12} < M_{\rm host}/{\rm M}_{\odot} < 10^{13}$ sample, fifth stellar mass bin.

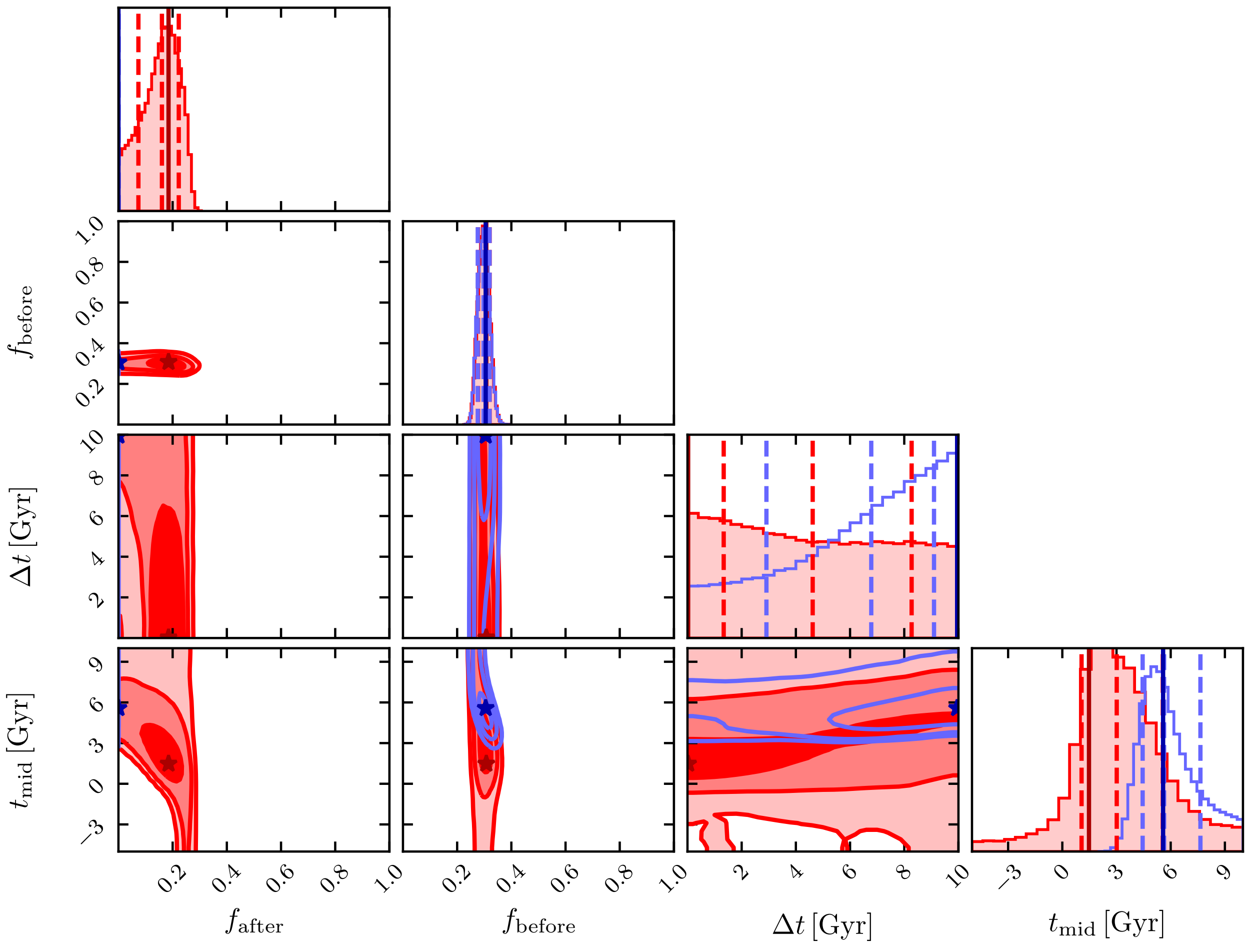


**Figure F12.** As in Fig. F1, but for the SSFR analysis of the $10^{12} < M_{\rm host}/{\rm M}_{\odot} < 10^{13}$ sample, sixth stellar mass bin.

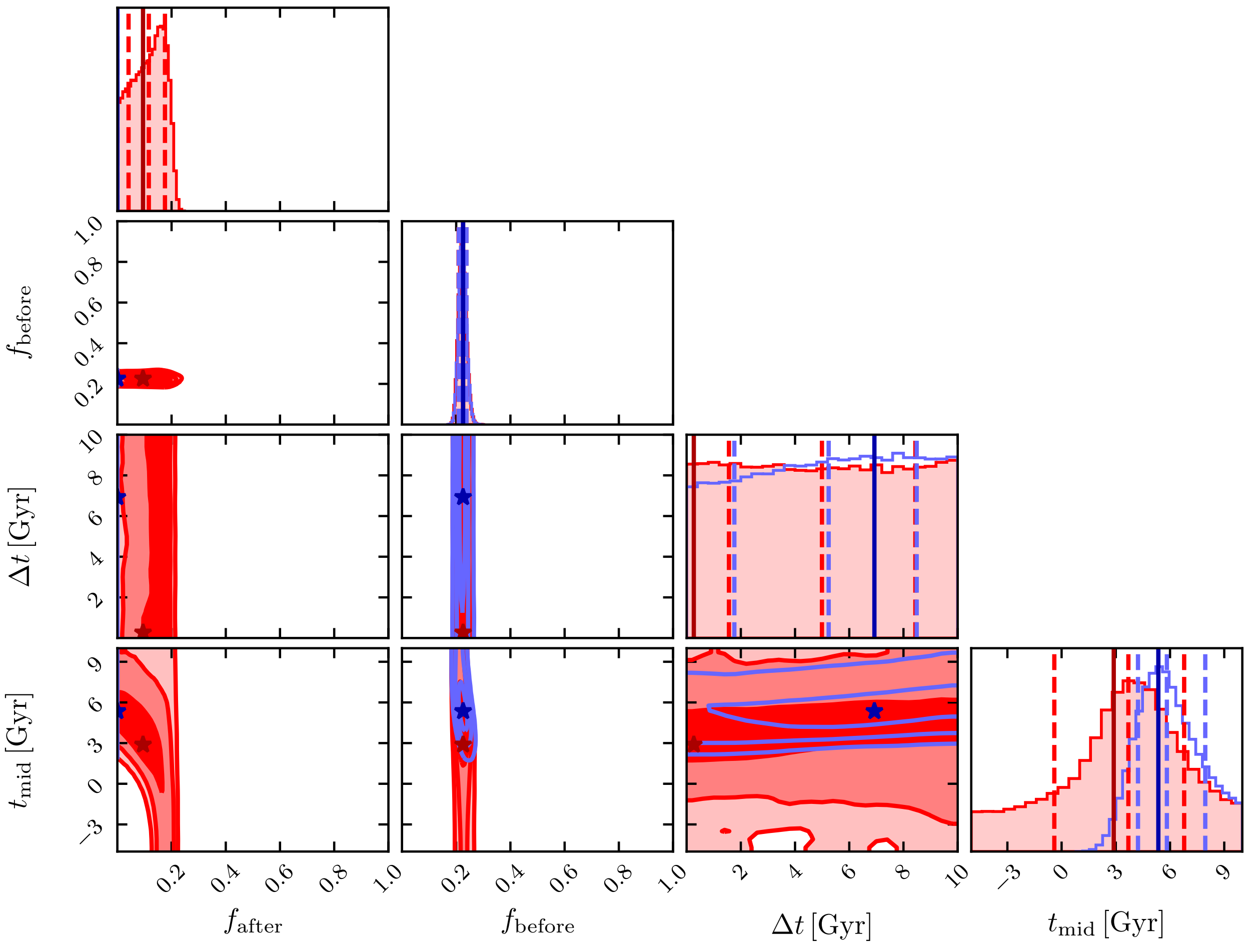


**Figure F13.** As in Fig. F1, but for the gas analysis of the $10^{12} < M_{\rm host}/{\rm M}_\odot < 10^{13}$ sample, first stellar mass bin.

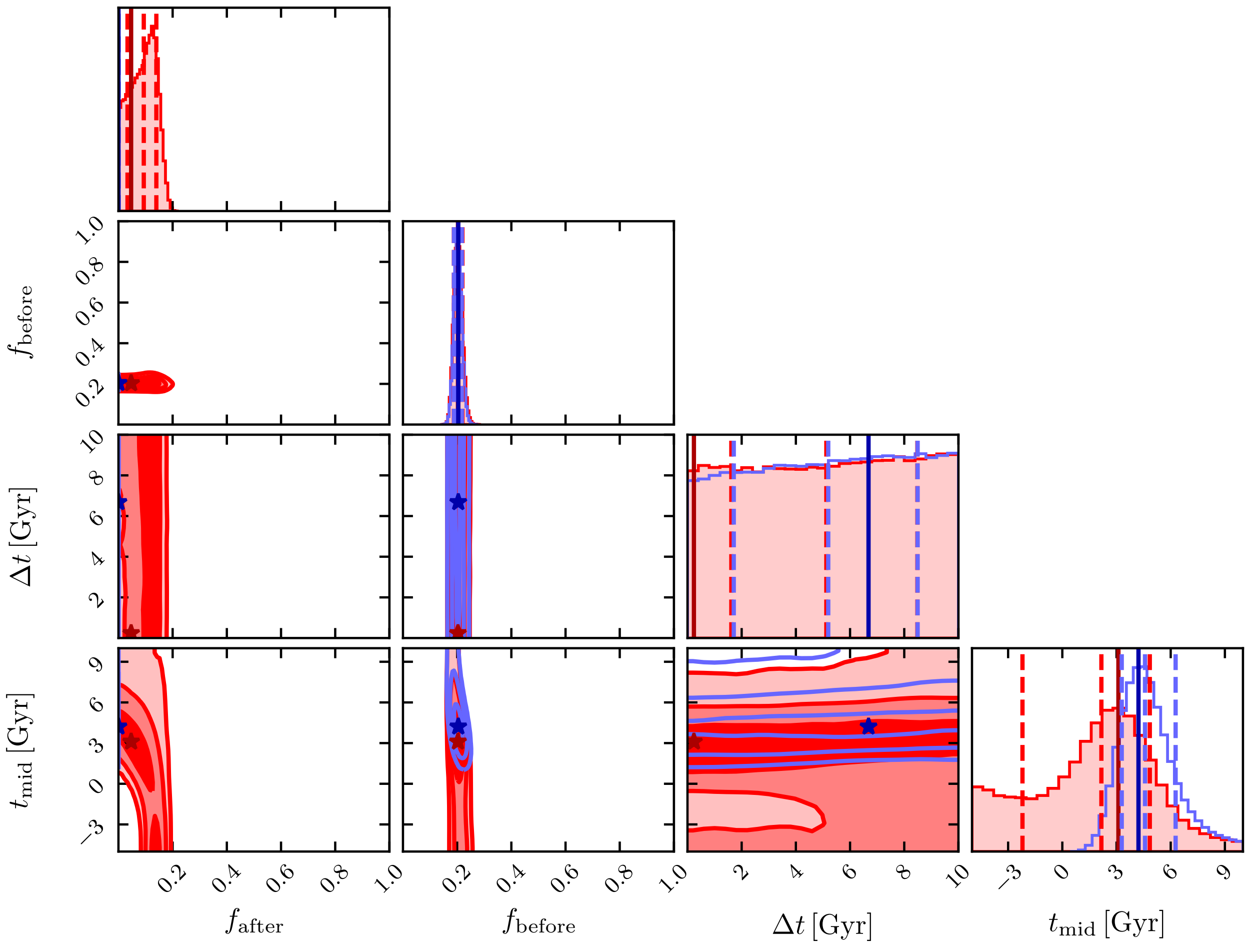


**Figure F14.** As in Fig. F1, but for the gas analysis of the $10^{12} < M_{\rm host}/{\rm M}_{\odot} < 10^{13}$ sample, second stellar mass bin.

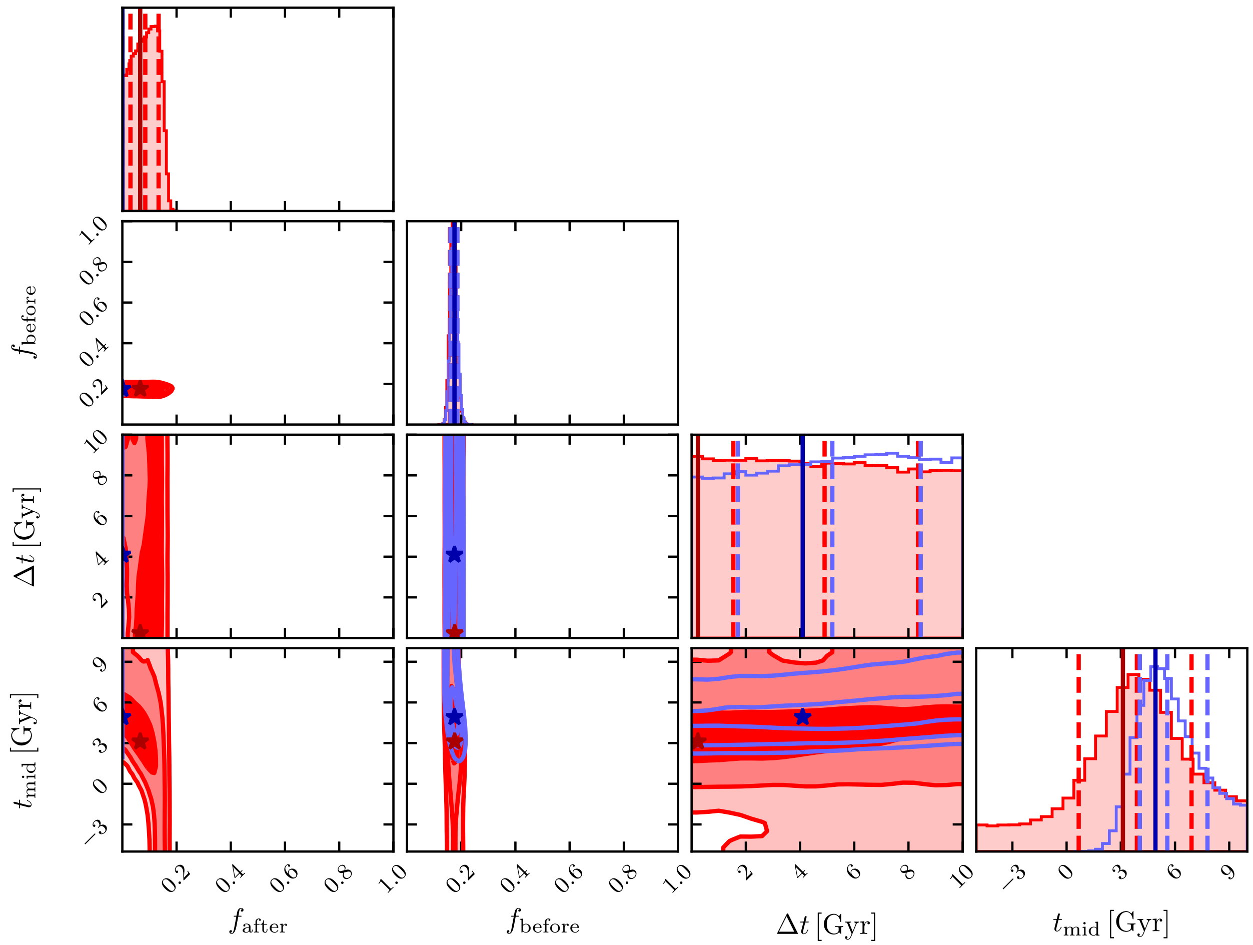


**Figure F15.** As in Fig. F1, but for the gas analysis of the $10^{12} < M_{\rm host}/{\rm M}_{\odot} < 10^{13}$ sample, third stellar mass bin.

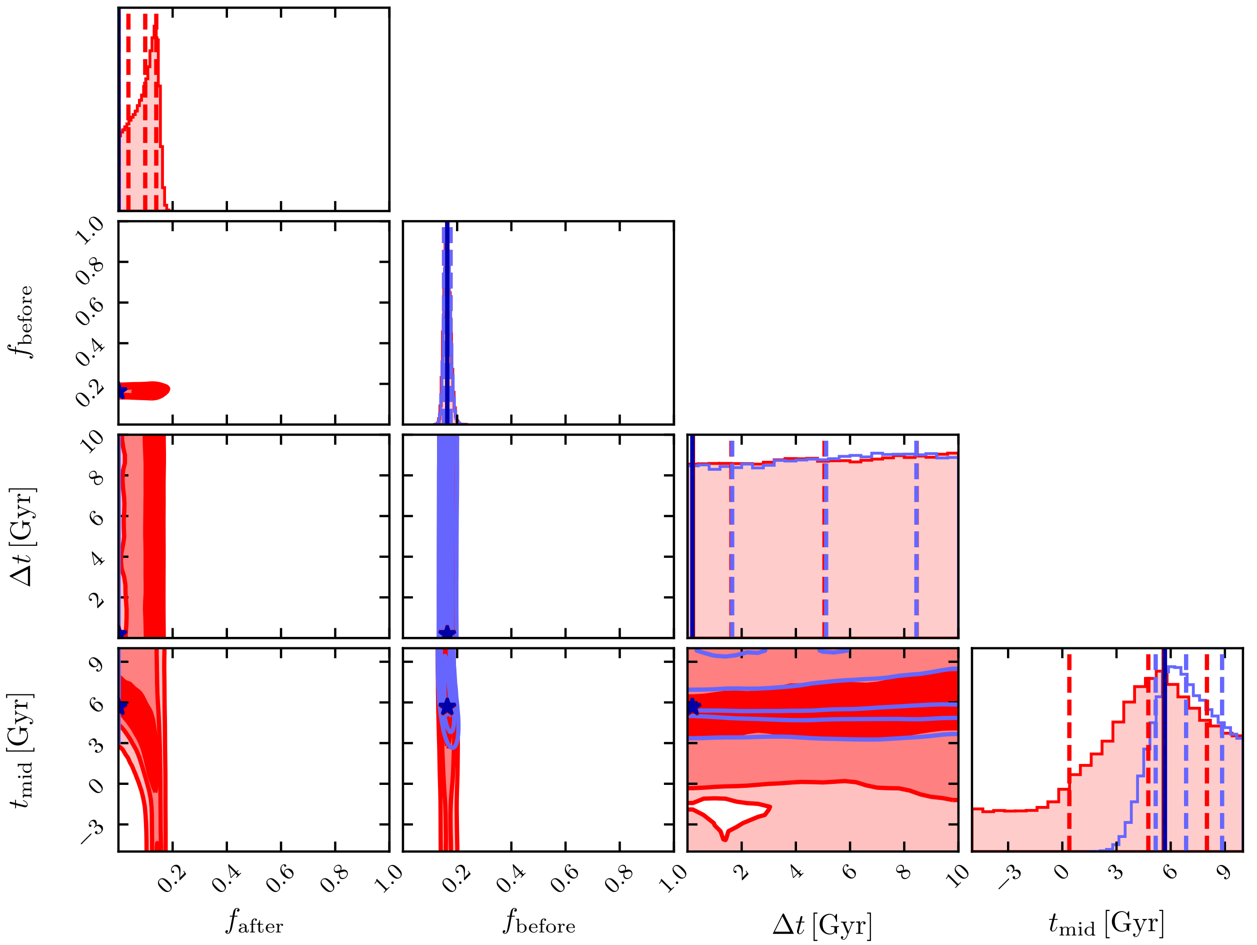


**Figure F16.** As in Fig. F1, but for the gas analysis of the $10^{12} < M_{\mathrm{host}}/\mathrm{M}_{\odot} < 10^{13}$ sample, fourth stellar mass bin.

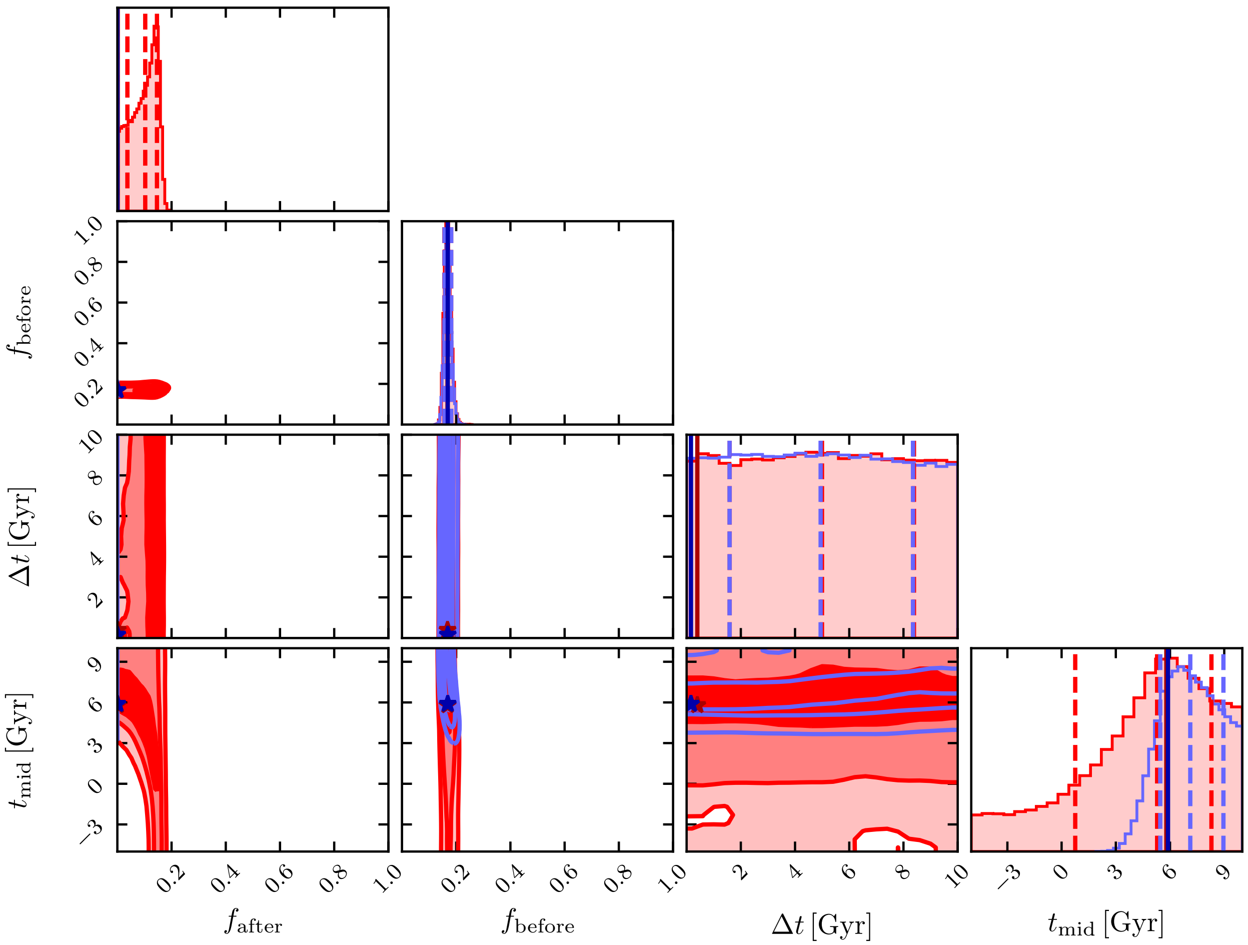


**Figure F17.** As in Fig. F1, but for the gas analysis of the $10^{12} < M_{\rm host}/{\rm M}_{\odot} < 10^{13}$ sample, fifth stellar mass bin.

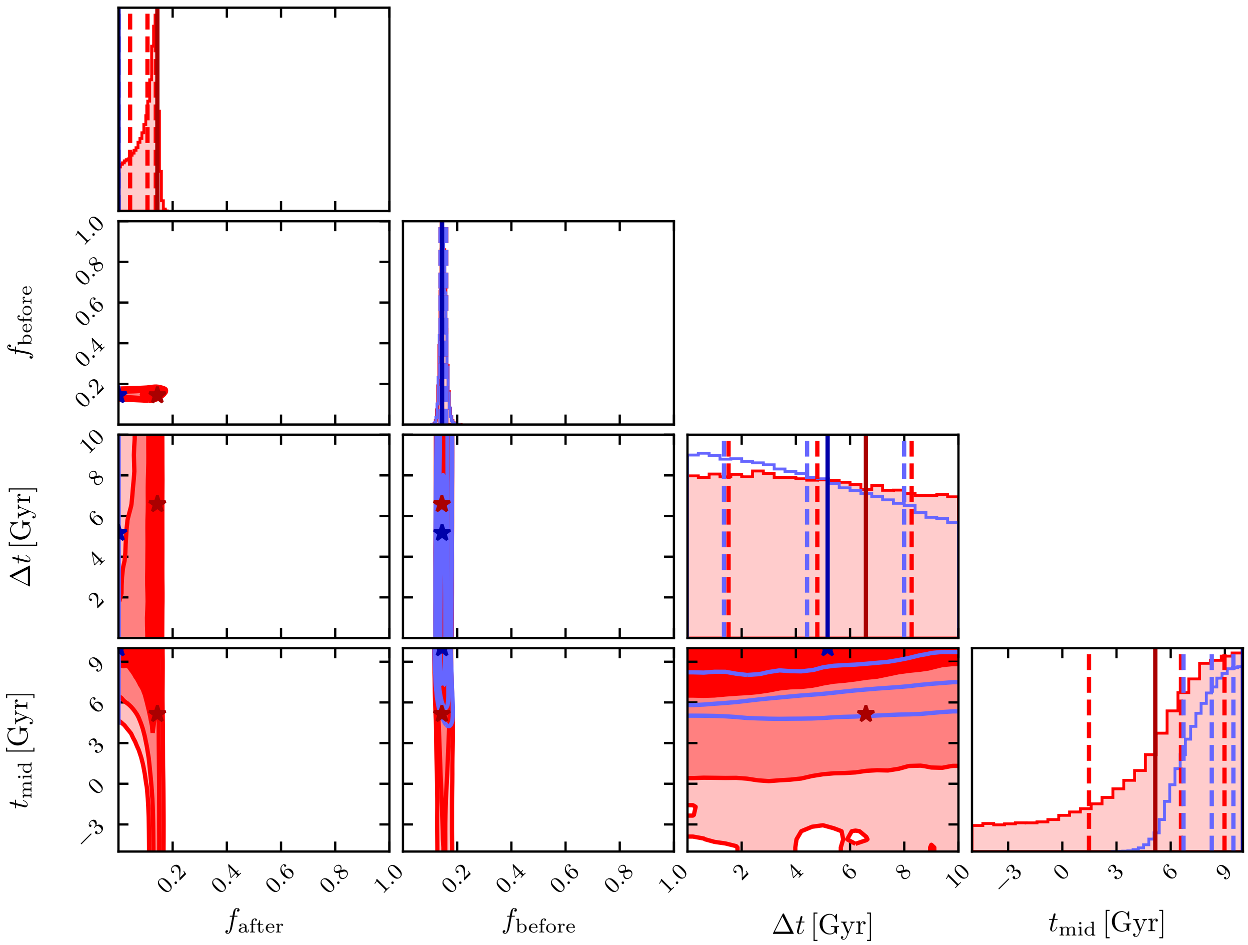


**Figure F18.** As in Fig. F1, but for the gas analysis of the $10^{12} < M_{\rm host}/{\rm M}_{\odot} < 10^{13}$ sample, sixth stellar mass bin.

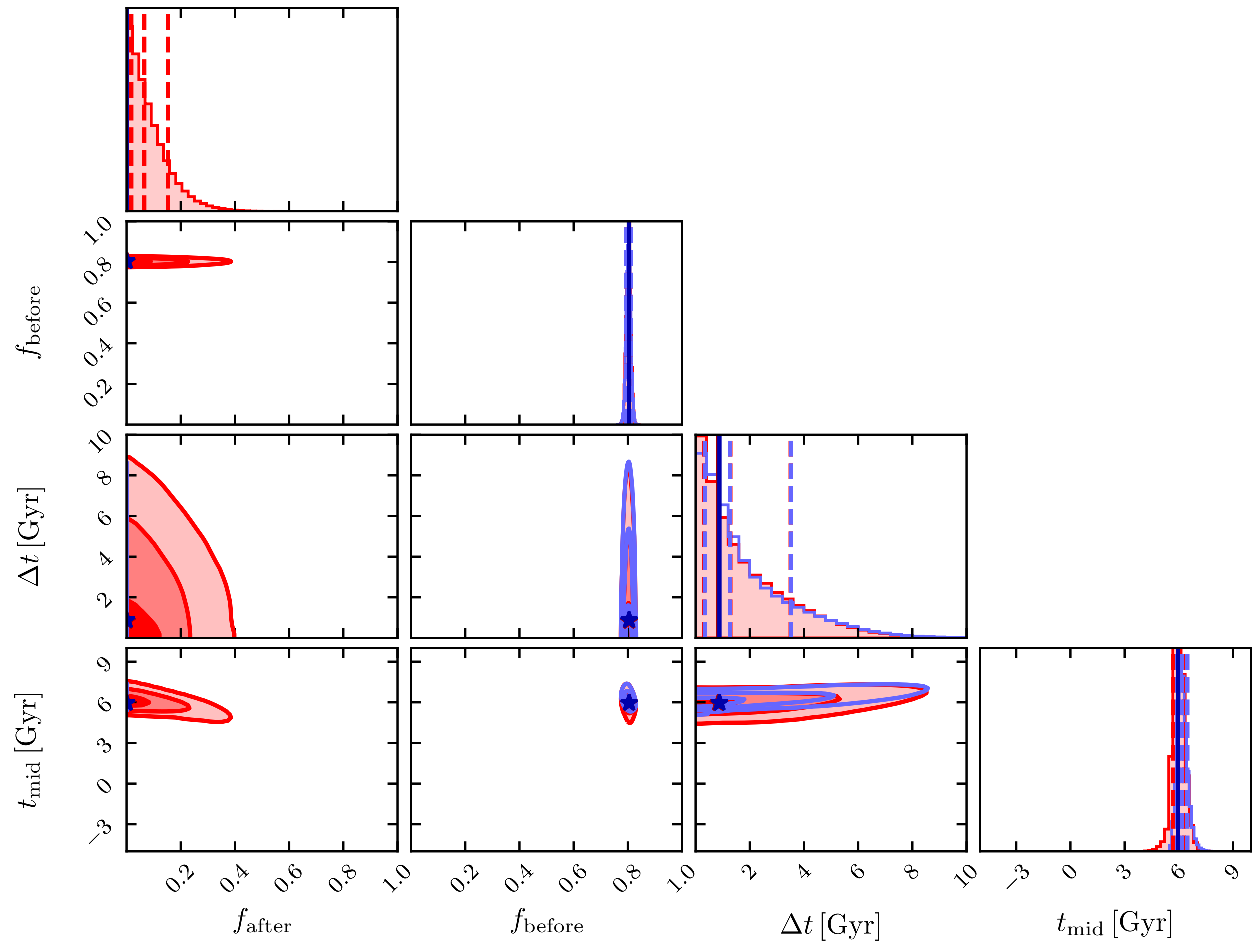


**Figure F19.** As in Fig. F1, but for the $(g-r)$ colour analysis of the $10^{13} < M_{\rm host}/{\rm M}_{\odot} < 10^{14}$ sample, first stellar mass bin.

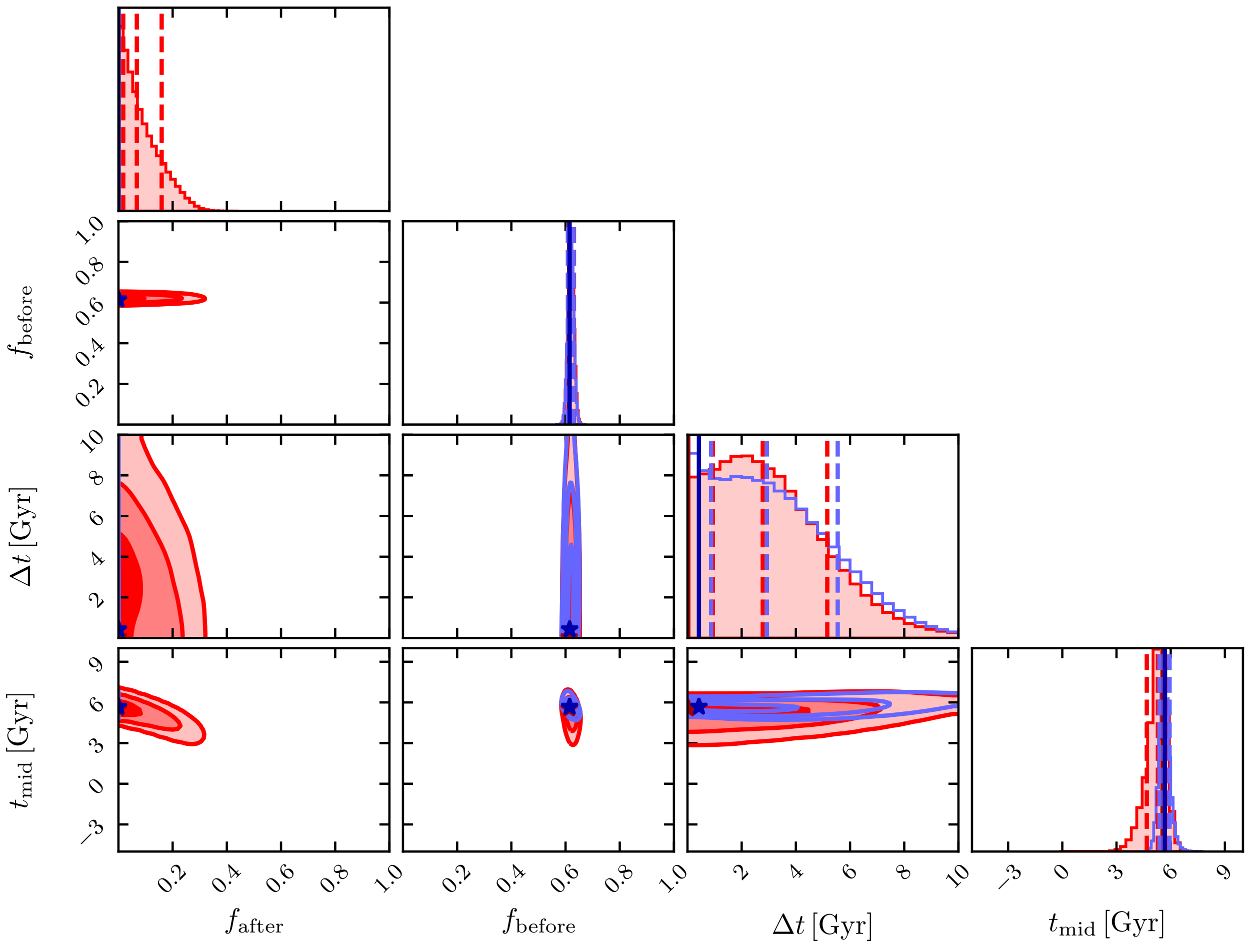


**Figure F20.** As in Fig. F1, but for the $(g-r)$ colour analysis of the $10^{13} < M_{\rm host}/{\rm M}_{\odot} < 10^{14}$ sample, second stellar mass bin.

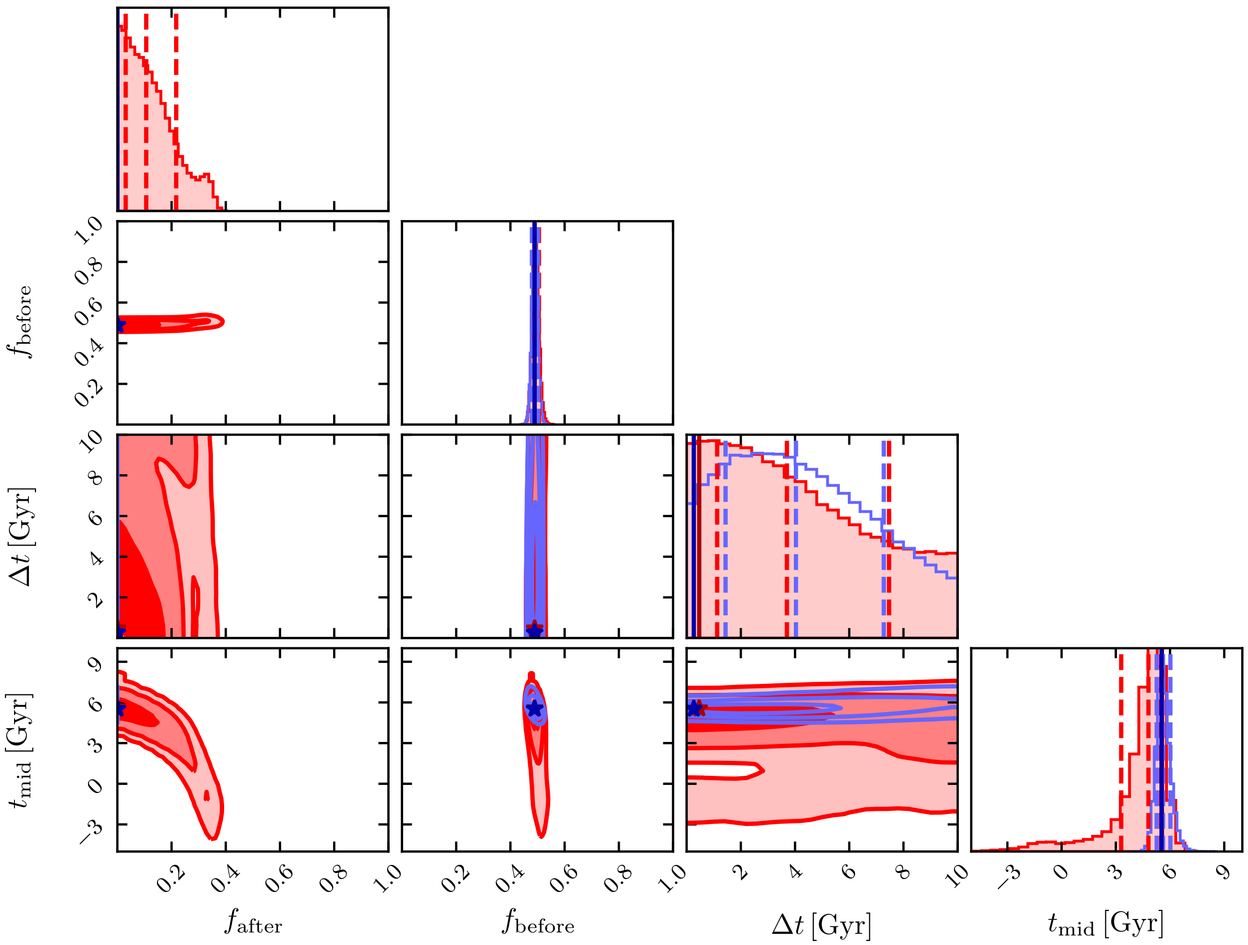


**Figure F21.** As in Fig. F1, but for the $(g-r)$ colour analysis of the $10^{13} < M_{\rm host}/{\rm M}_{\odot} < 10^{14}$ sample, third stellar mass bin.

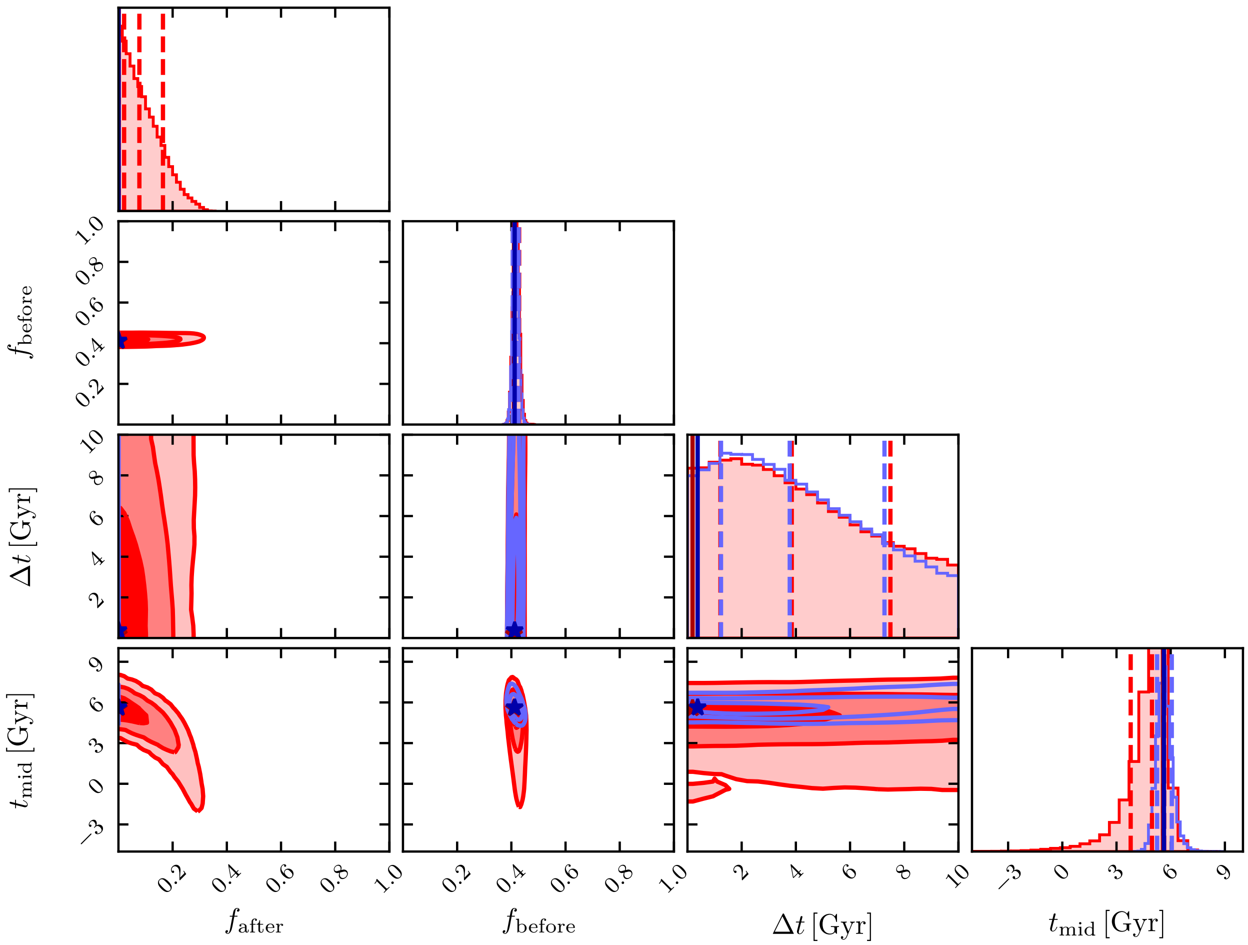


**Figure F22.** As in Fig. F1, but for the $(g-r)$ colour analysis of the $10^{13} < M_{\rm host}/{\rm M}_\odot < 10^{14}$ sample, fourth stellar mass bin.

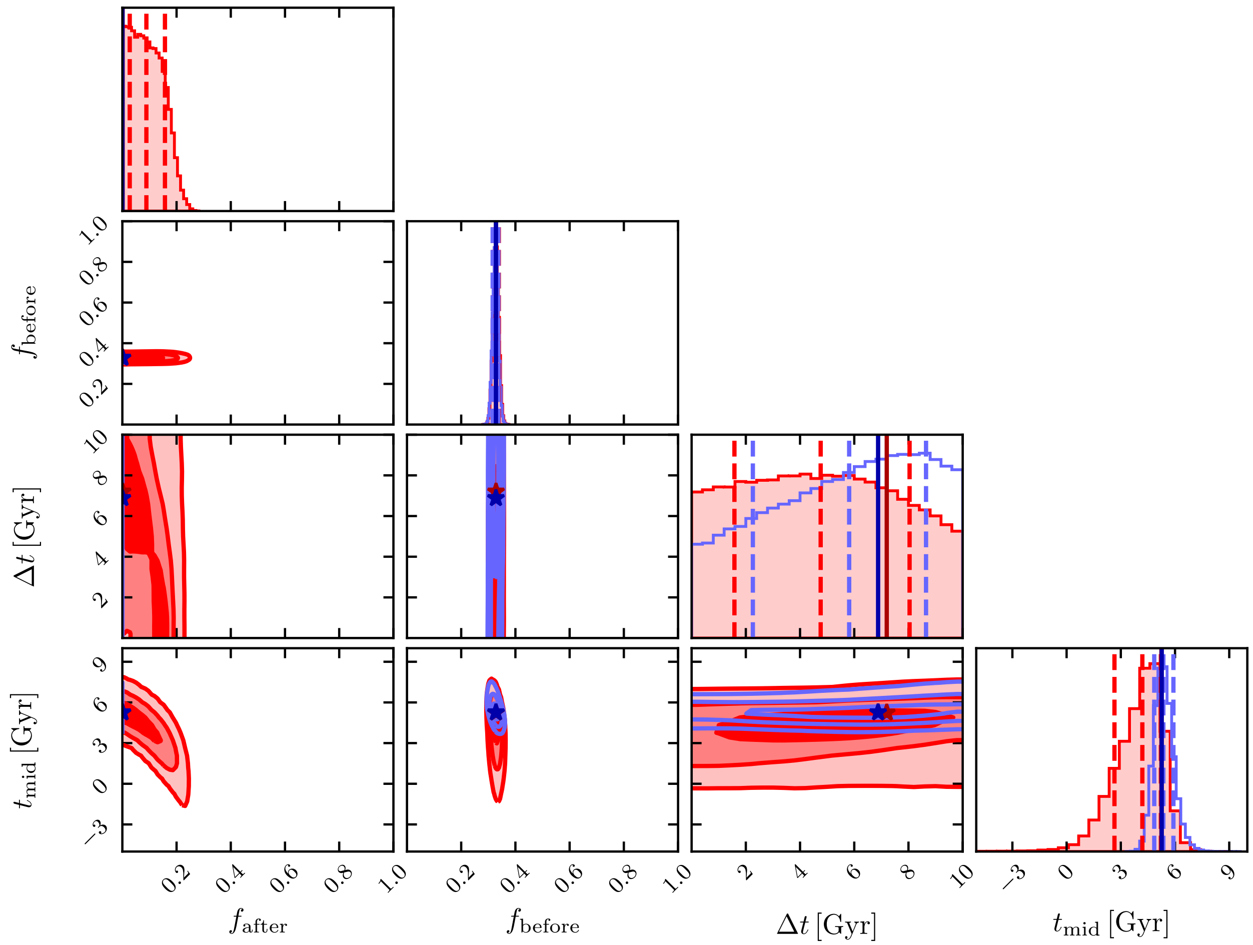


**Figure F23.** As in Fig. F1, but for the $(g-r)$ colour analysis of the $10^{13} < M_{\rm host}/{\rm M}_{\odot} < 10^{14}$ sample, fifth stellar mass bin.

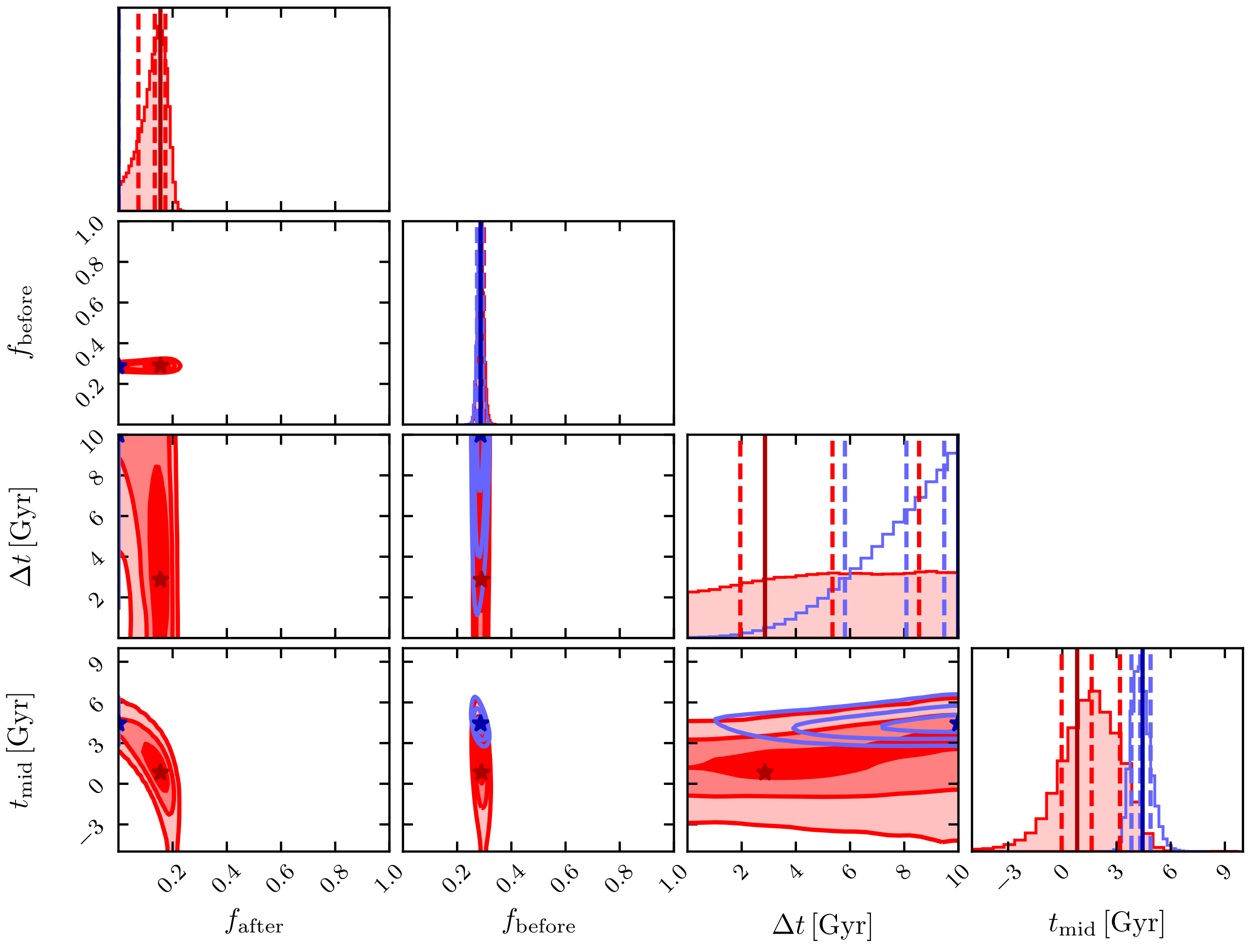


**Figure F24.** As in Fig. F1, but for the $(g-r)$ colour analysis of the $10^{13} < M_{\rm host}/{\rm M}_{\odot} < 10^{14}$ sample, sixth stellar mass bin.

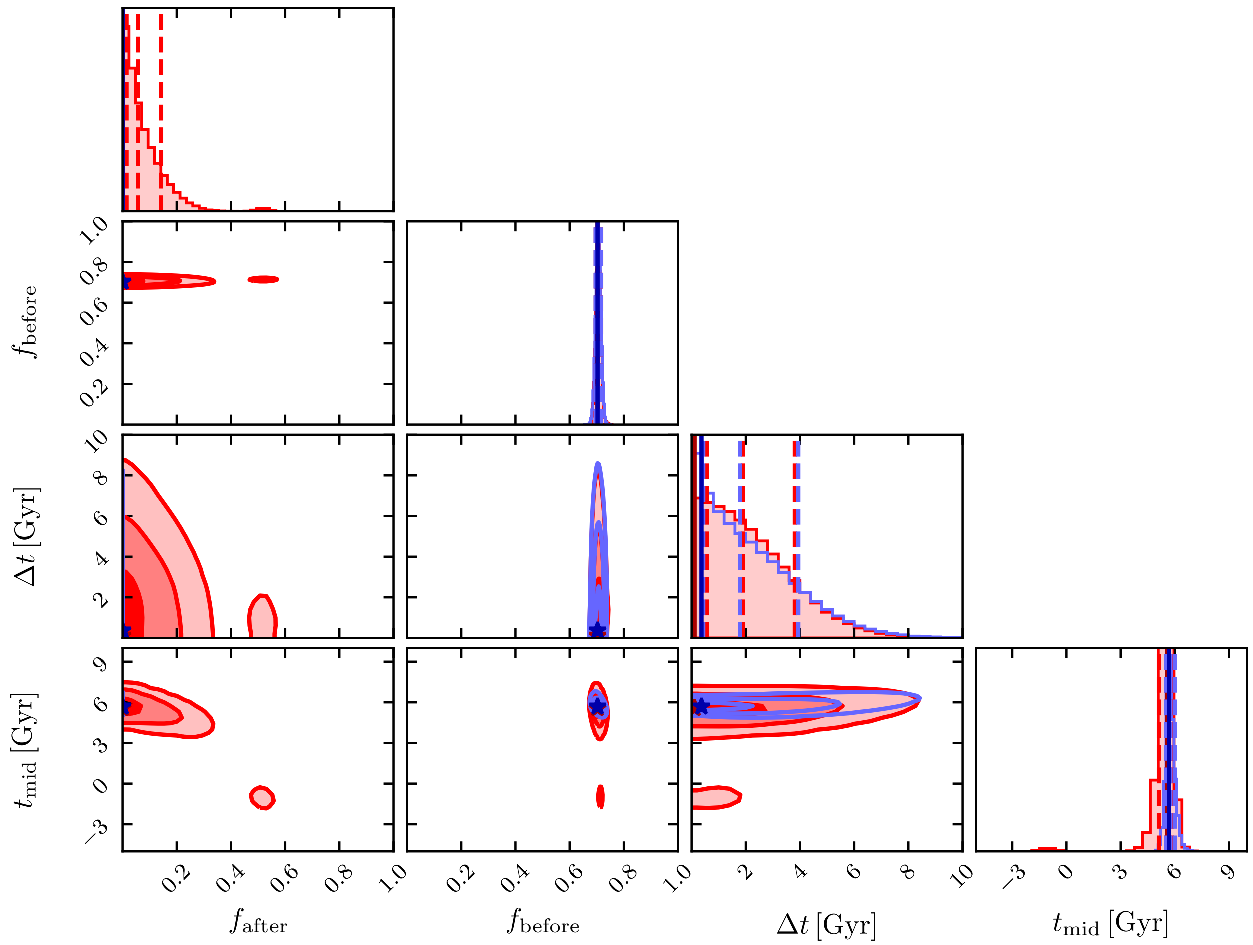


**Figure F25.** As in Fig. F1, but for the SSFR analysis of the $10^{13} < M_{\rm host}/{\rm M}_\odot < 10^{14}$ sample, first stellar mass bin.

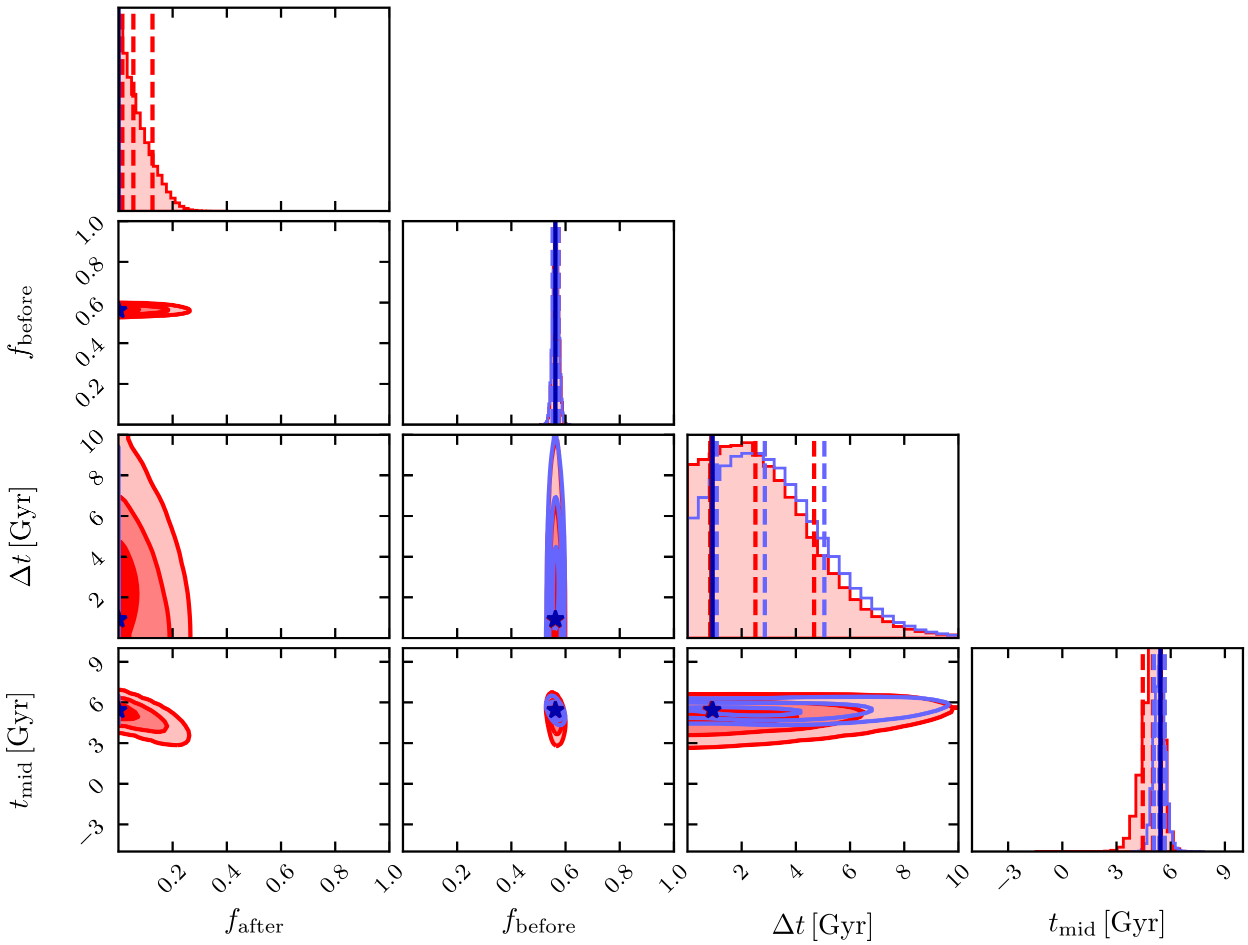


**Figure F26.** As in Fig. F1, but for the SSFR analysis of the $10^{13} < M_{\rm host}/{\rm M}_{\odot} < 10^{14}$ sample, second stellar mass bin.

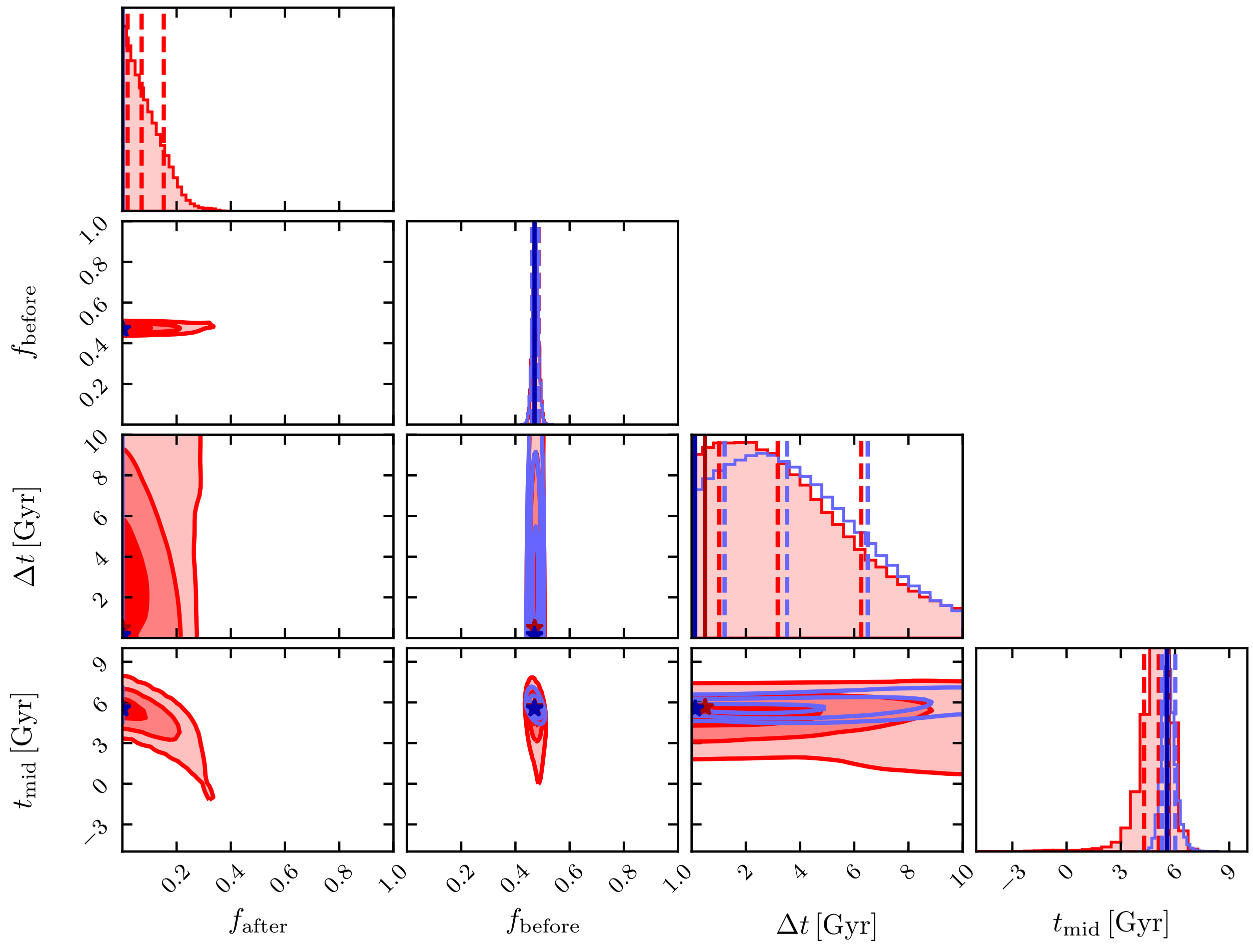


**Figure F27.** As in Fig. F1, but for the SSFR analysis of the $10^{13} < M_{\rm host}/{\rm M}_{\odot} < 10^{14}$ sample, third stellar mass bin.

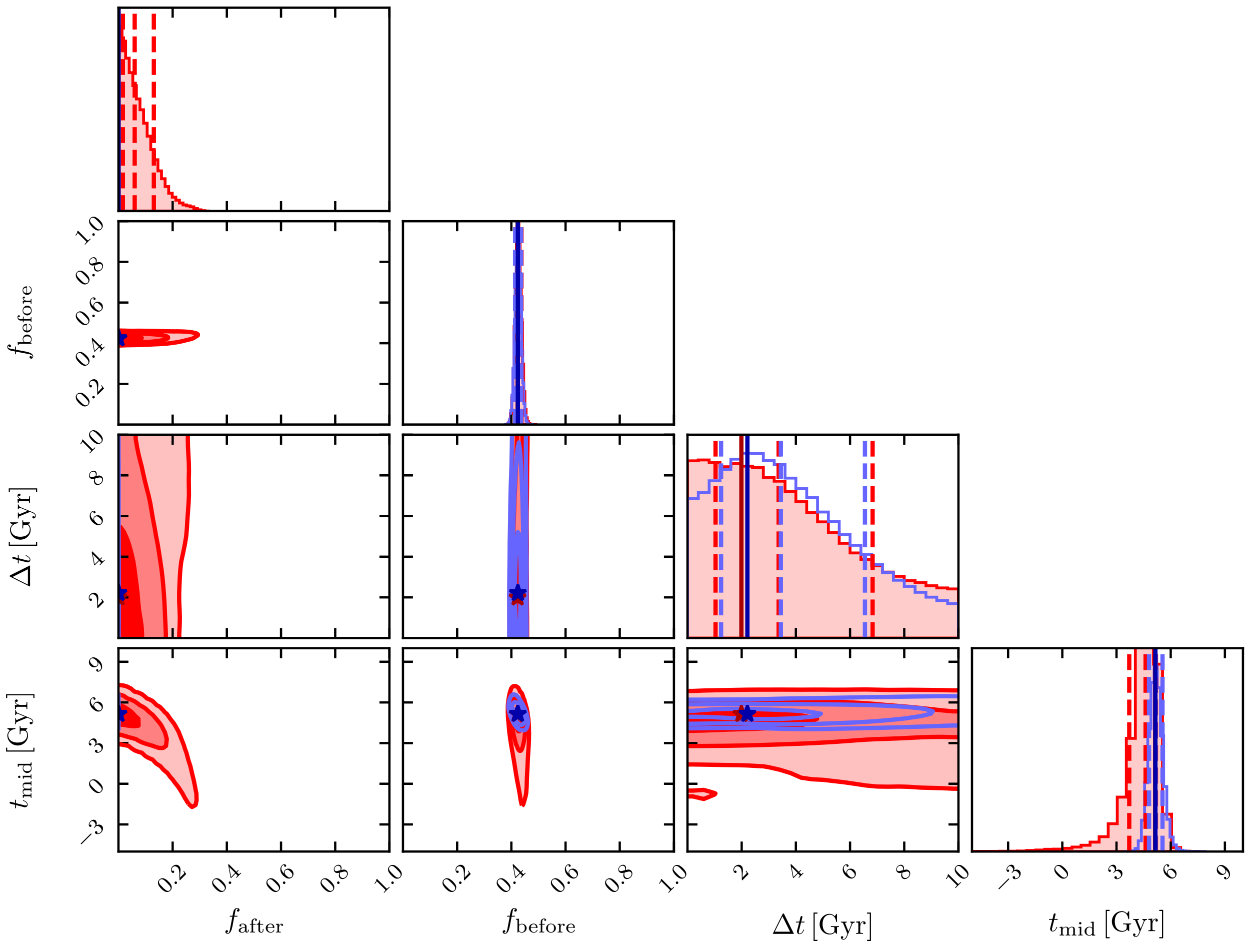


**Figure F28.** As in Fig. F1, but for the SSFR analysis of the $10^{13} < M_{\rm host}/{\rm M}_{\odot} < 10^{14}$ sample, fourth stellar mass bin.

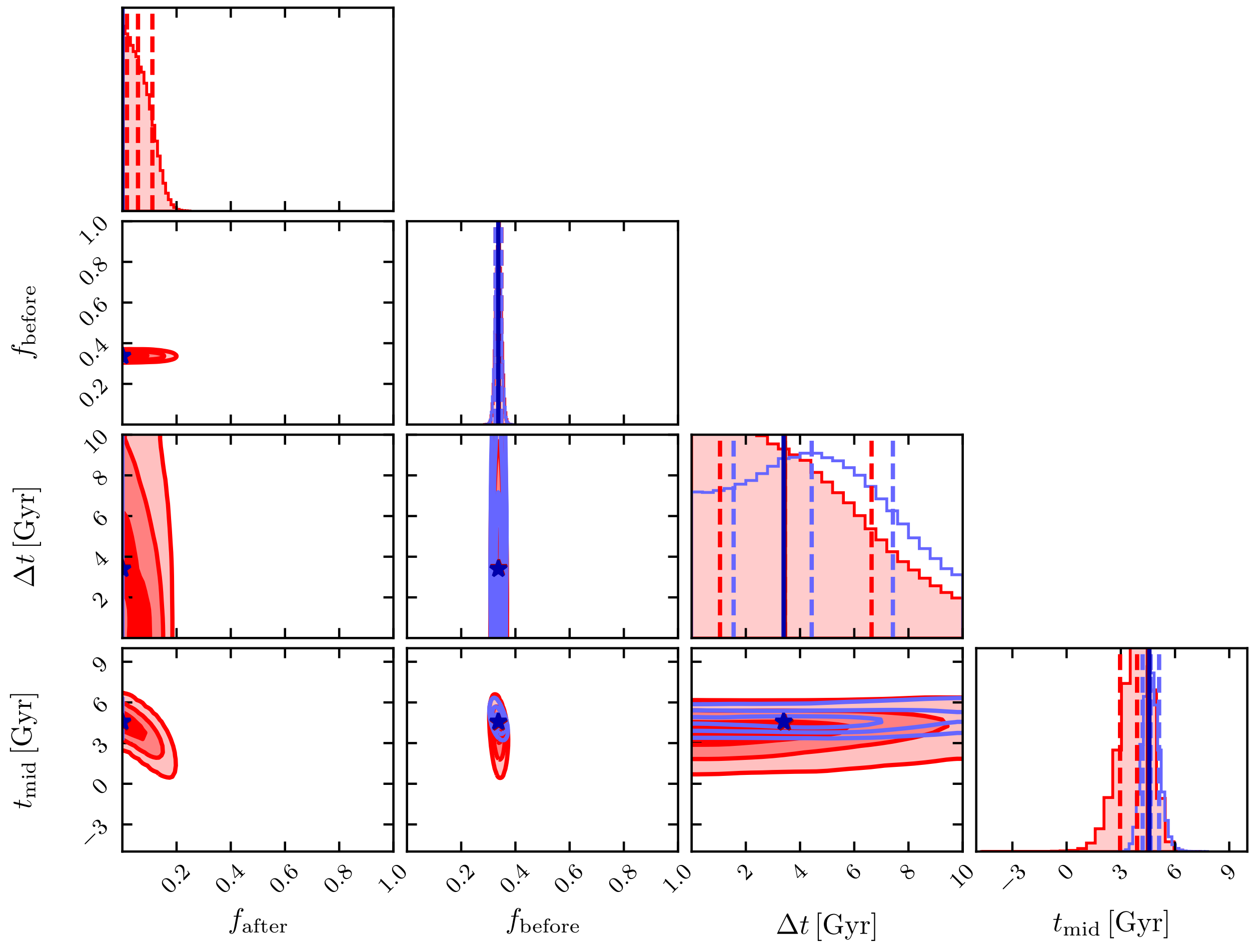


**Figure F29.** As in Fig. F1, but for the SSFR analysis of the $10^{13} < M_{\mathrm{host}}/\mathrm{M}_{\odot} < 10^{14}$ sample, fifth stellar mass bin.

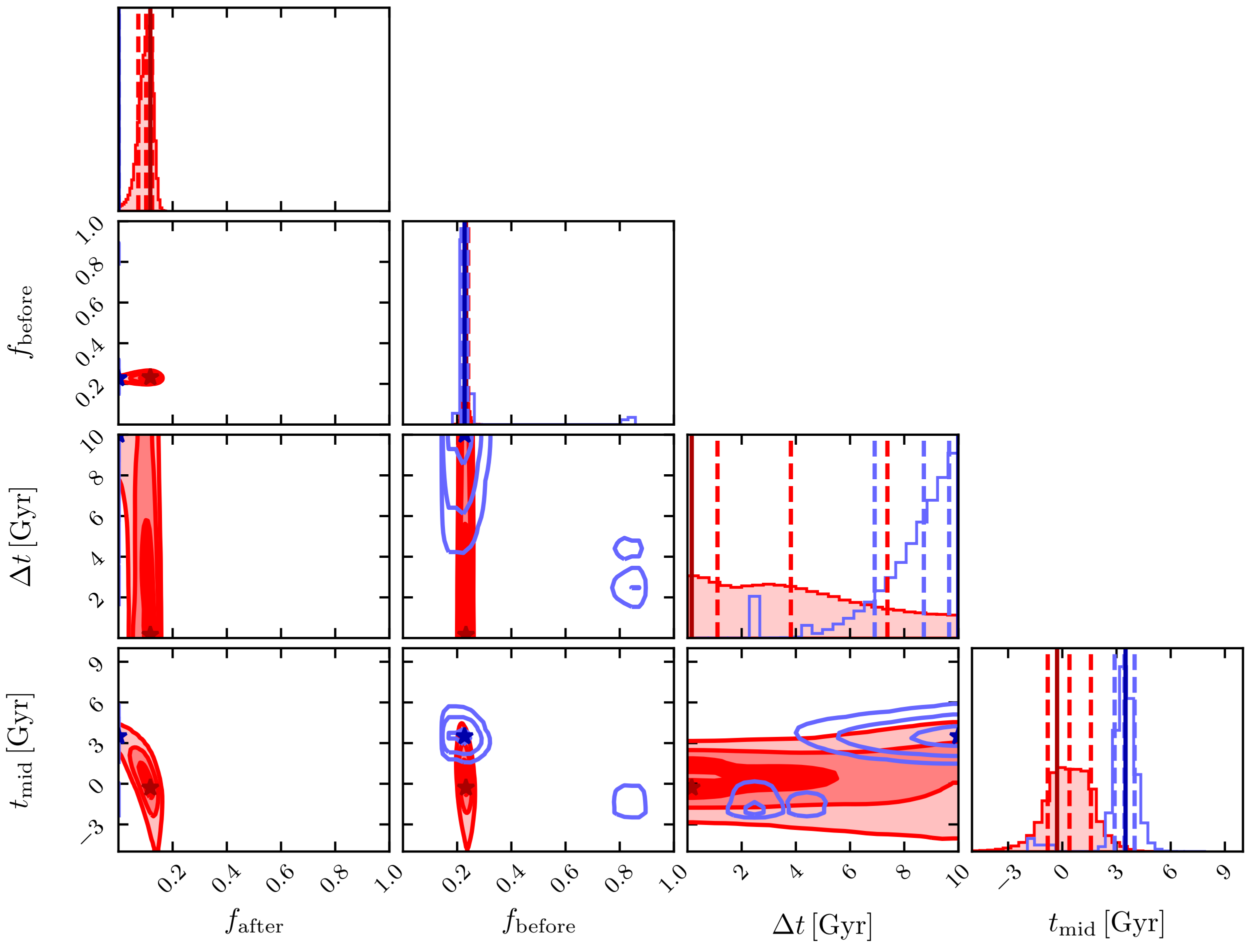


**Figure F30.** As in Fig. F1, but for the SSFR analysis of the $10^{13} < M_{\rm host}/{\rm M}_{\odot} < 10^{14}$ sample, sixth stellar mass bin.

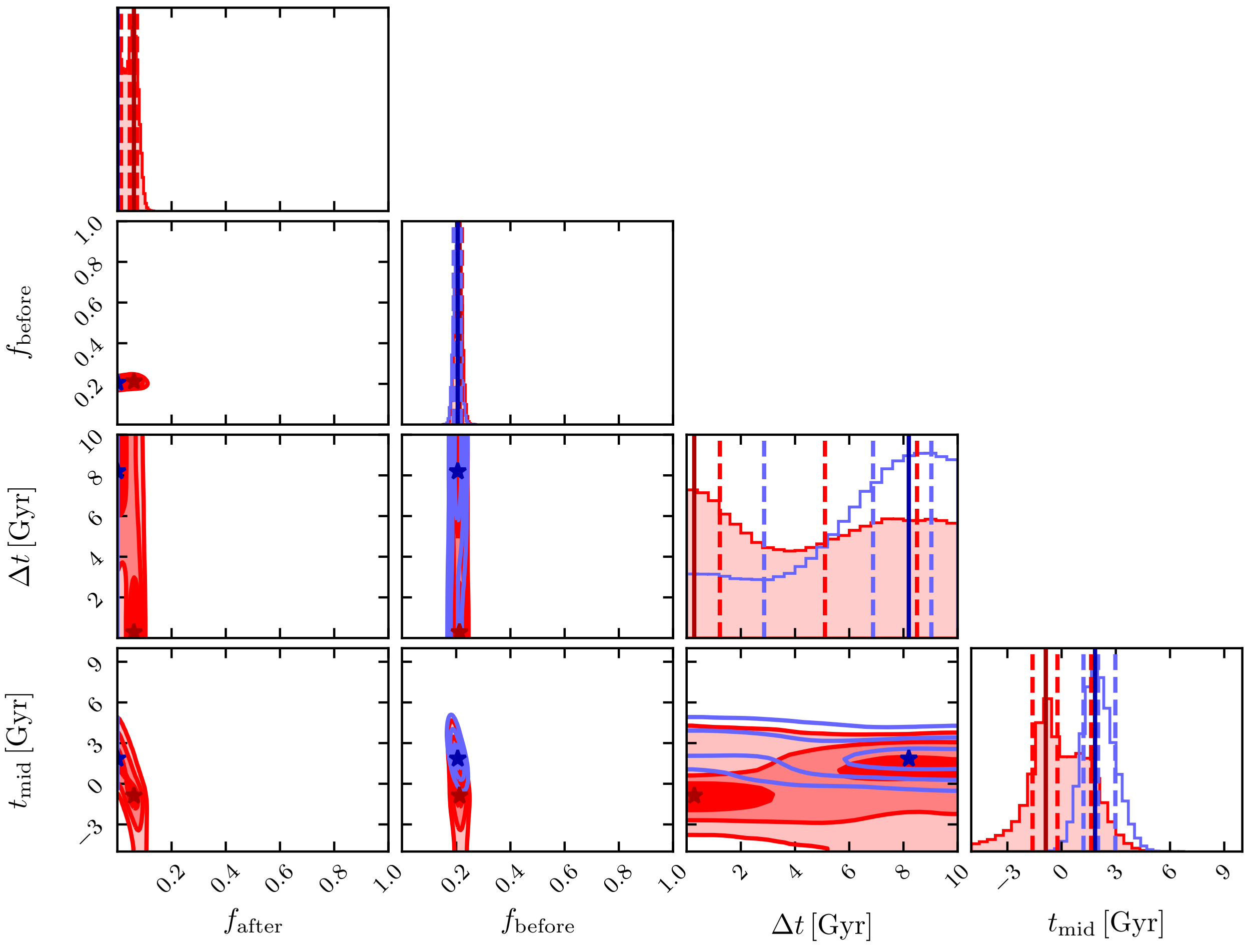


**Figure F31.** As in Fig. F1, but for the gas analysis of the $10^{13} < M_{\rm host}/{\rm M}_\odot < 10^{14}$ sample, first stellar mass bin.

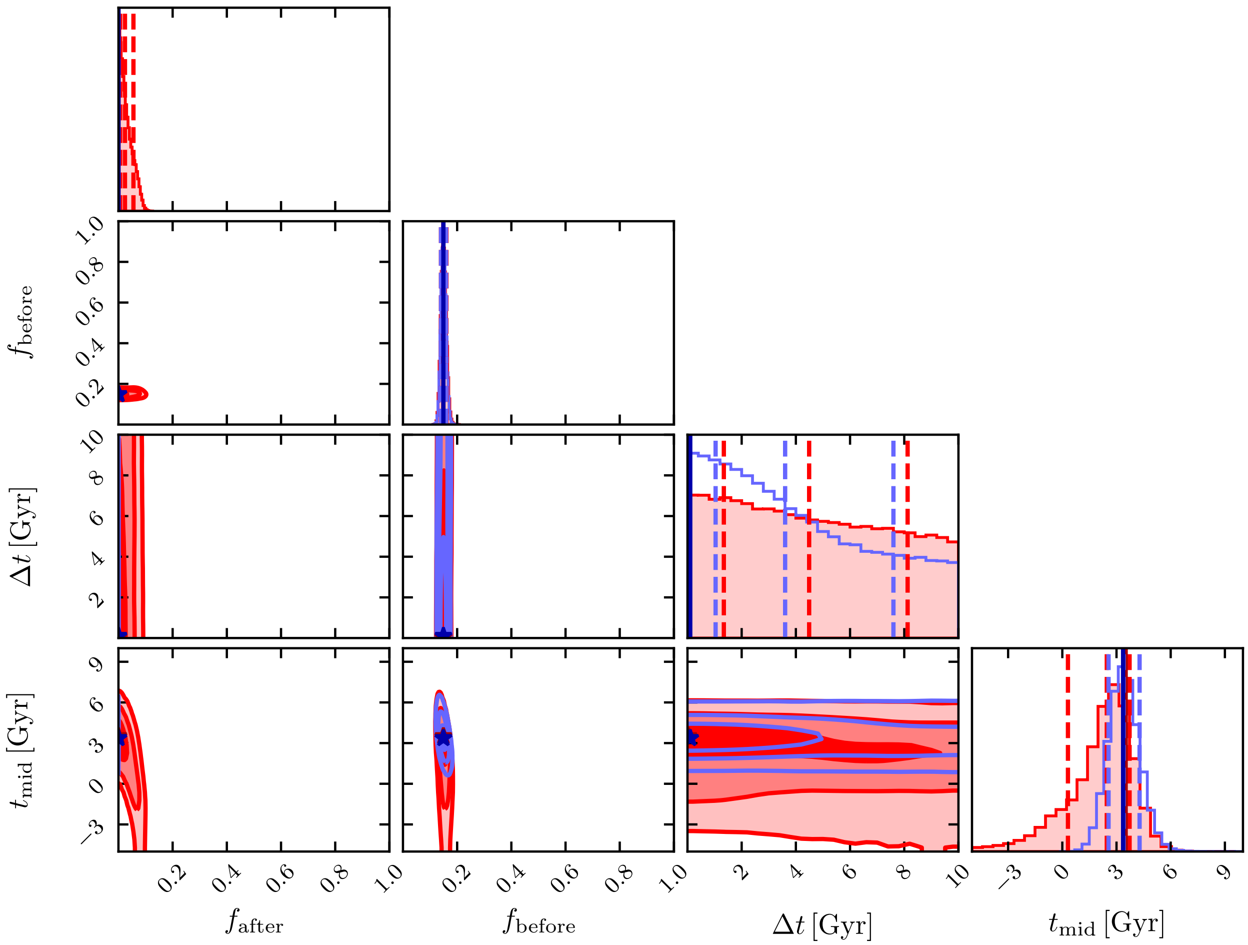


**Figure F32.** As in Fig. F1, but for the gas analysis of the $10^{13} < M_{\rm host}/{\rm M}_{\odot} < 10^{14}$ sample, second stellar mass bin.

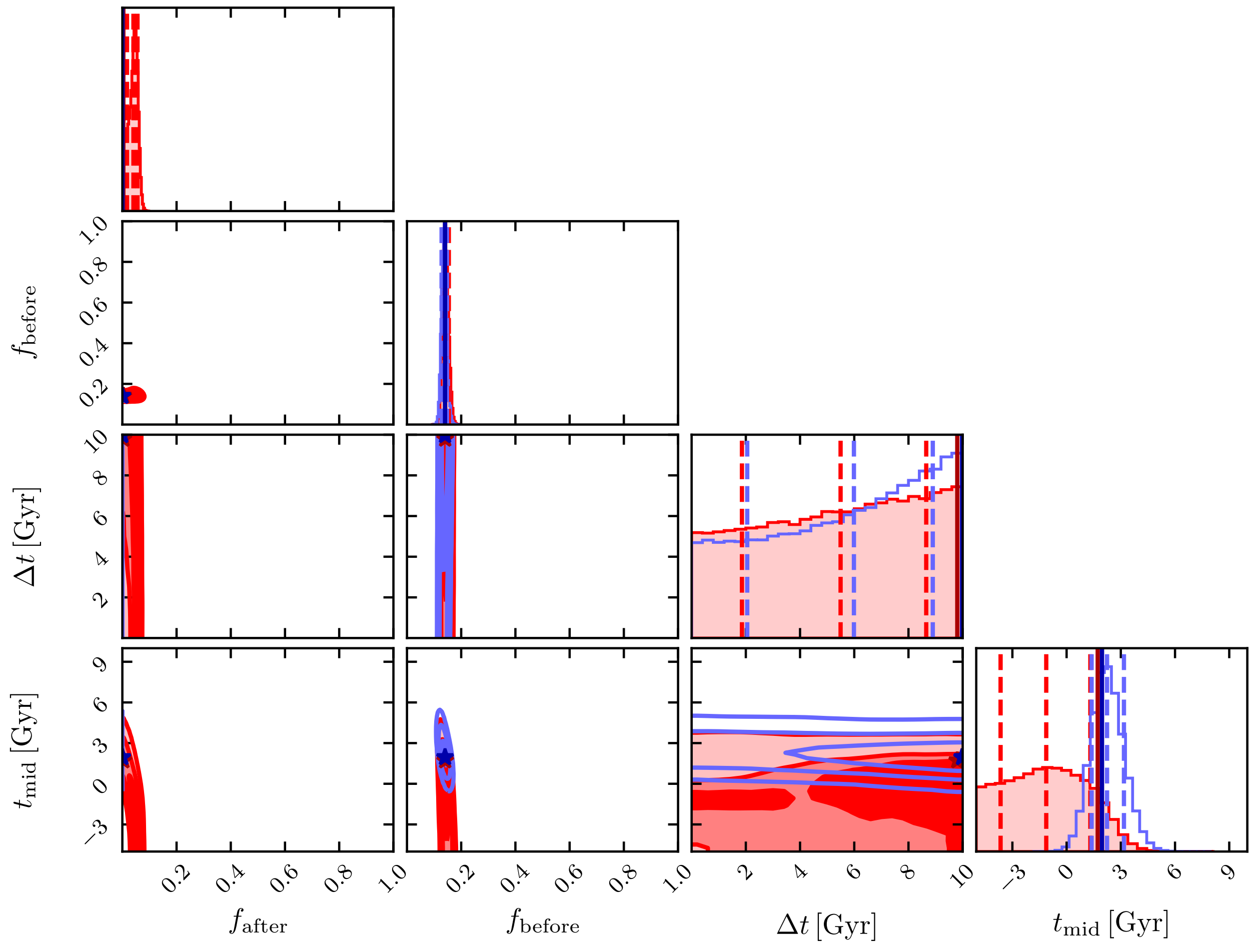


**Figure F33.** As in Fig. F1, but for the gas analysis of the $10^{13} < M_{\rm host}/{\rm M}_{\odot} < 10^{14}$ sample, third stellar mass bin.

© 0000 RAS, MNRAS **000**, 000–000

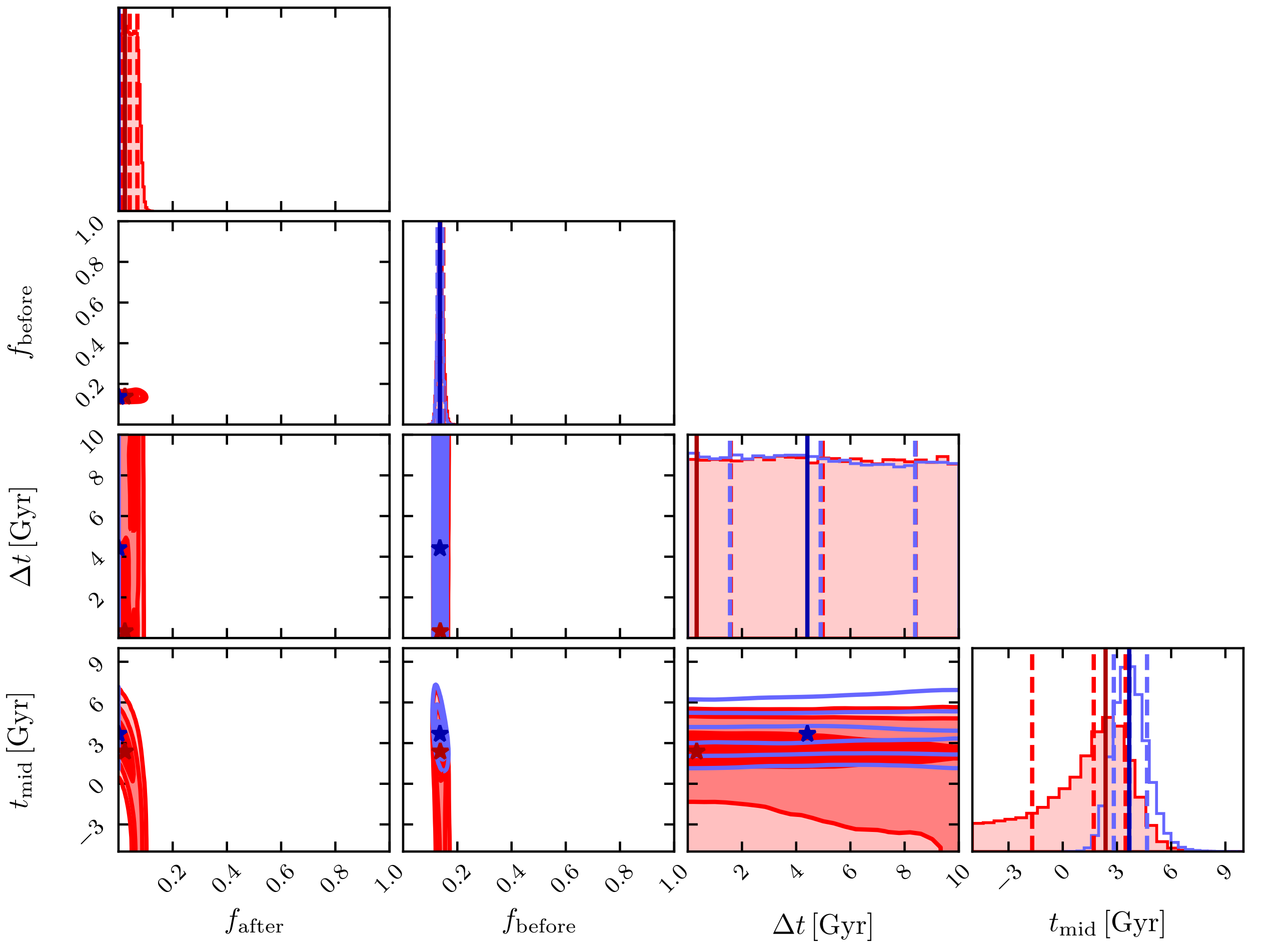


**Figure F34.** As in Fig. F1, but for the gas analysis of the $10^{13} < M_{\rm host}/{\rm M}_{\odot} < 10^{14}$ sample, fourth stellar mass bin.

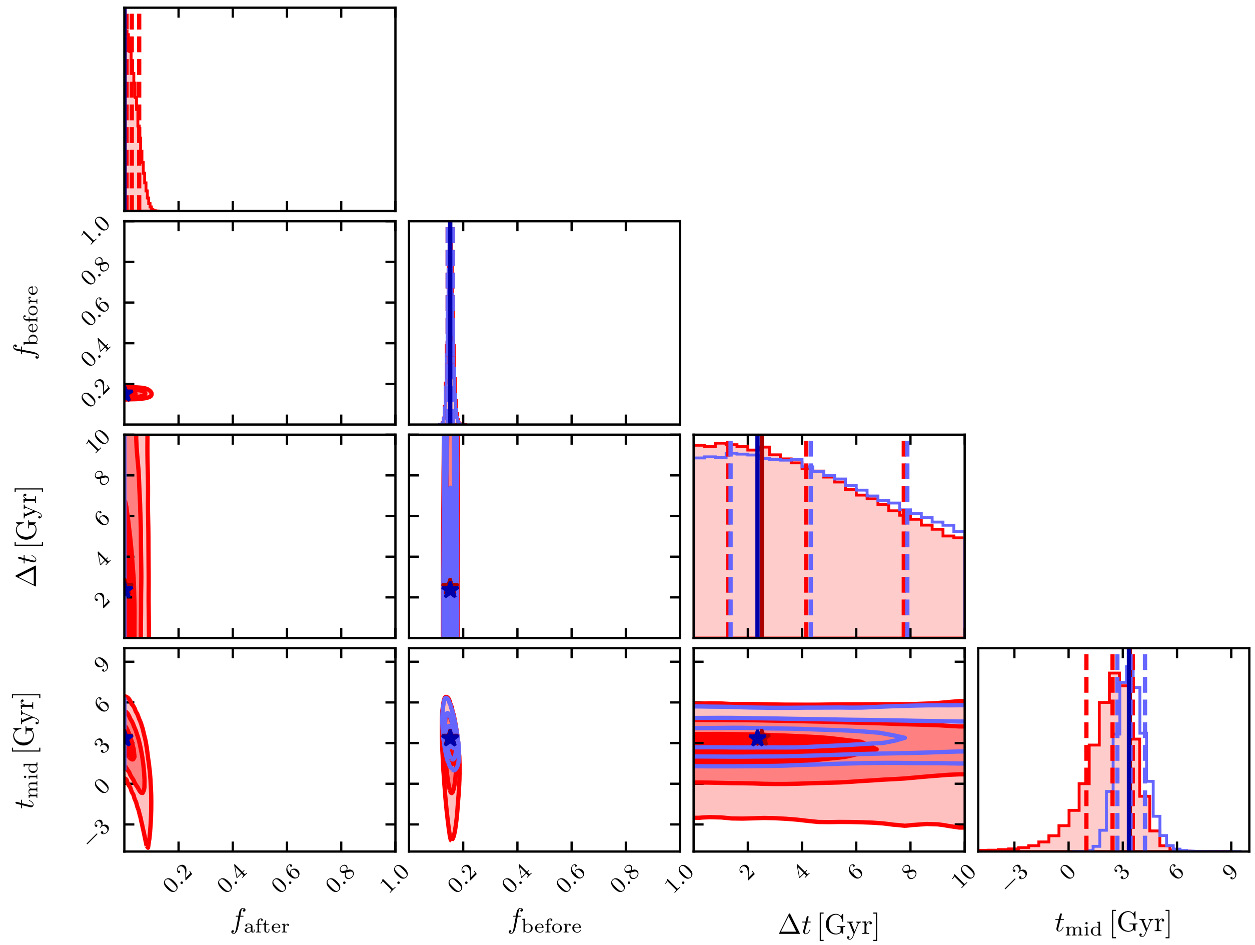


**Figure F35.** As in Fig. F1, but for the gas analysis of the $10^{13} < M_{\rm host}/{\rm M}_{\odot} < 10^{14}$ sample, fifth stellar mass bin.

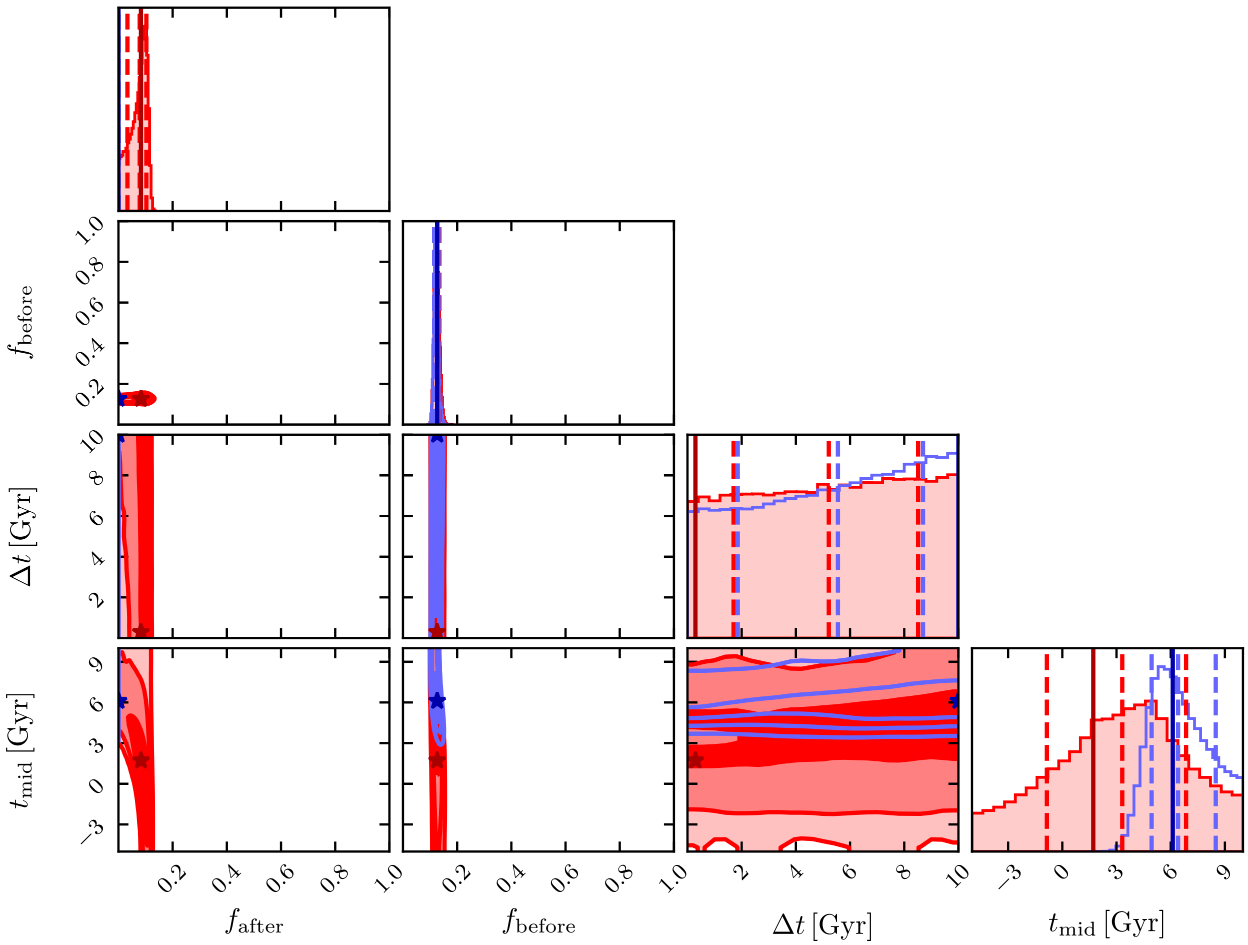


**Figure F36.** As in Fig. F1, but for the gas analysis of the $10^{13} < M_{\mathrm{host}}/\mathrm{M}_{\odot} < 10^{14}$ sample, sixth stellar mass bin.

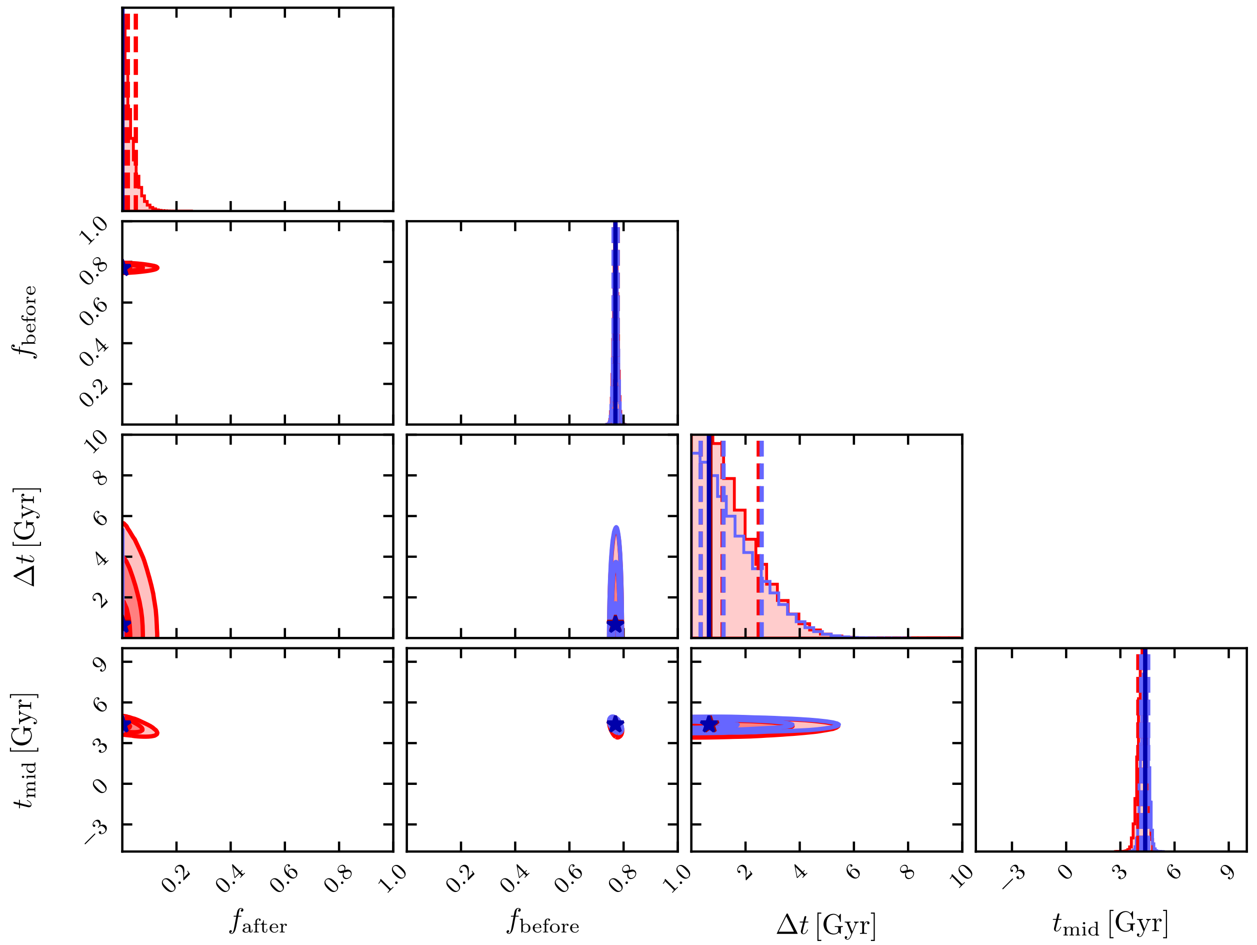


**Figure F37.** As in Fig. F1, but for the $(g-r)$ colour analysis of the $M_{\rm host}/{\rm M}_{\odot} > 10^{14}$ sample, first stellar mass bin.

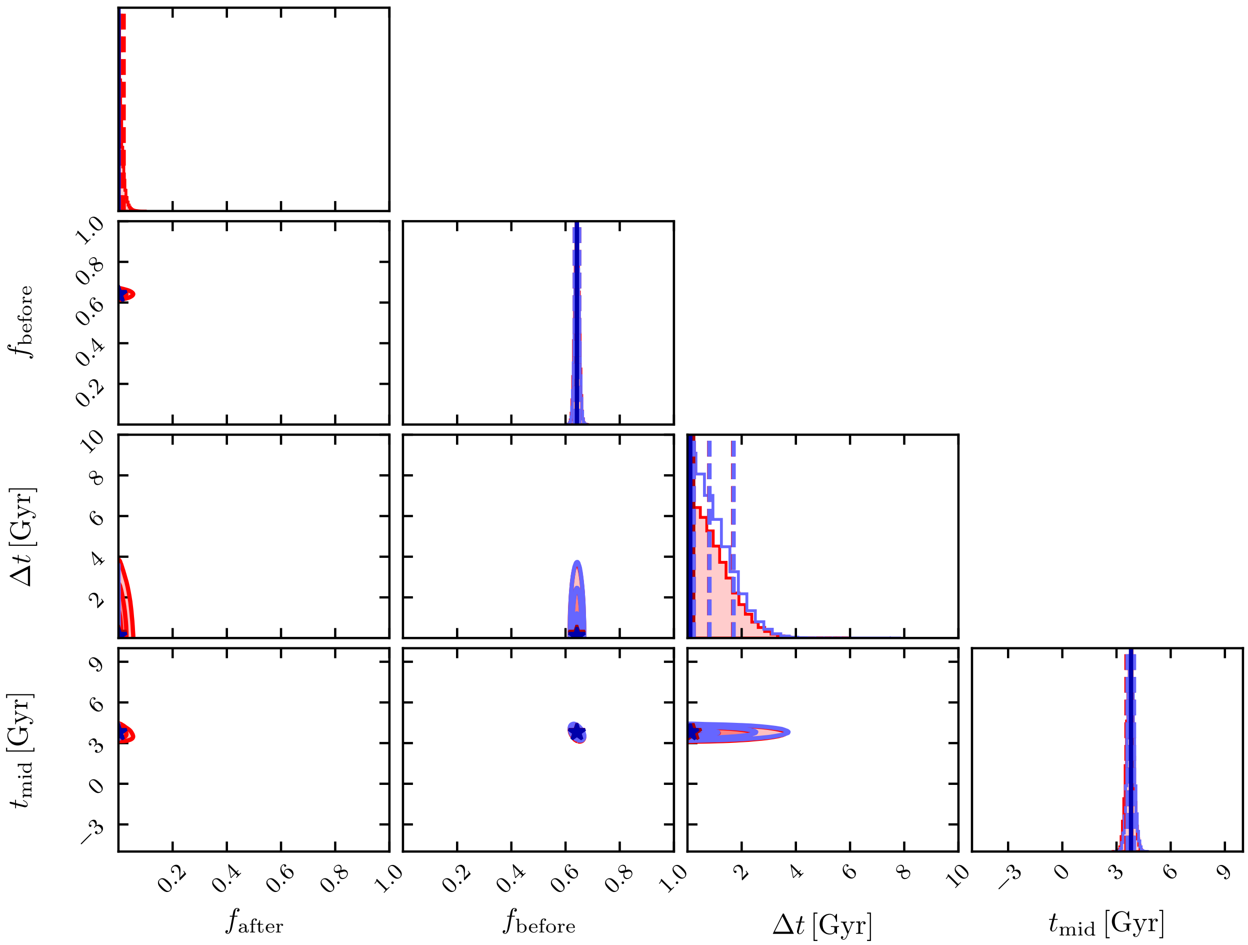


**Figure F38.** As in Fig. F1, but for the $(g-r)$ colour analysis of the $M_{\rm host}/{\rm M}_{\odot} > 10^{14}$ sample, second stellar mass bin.

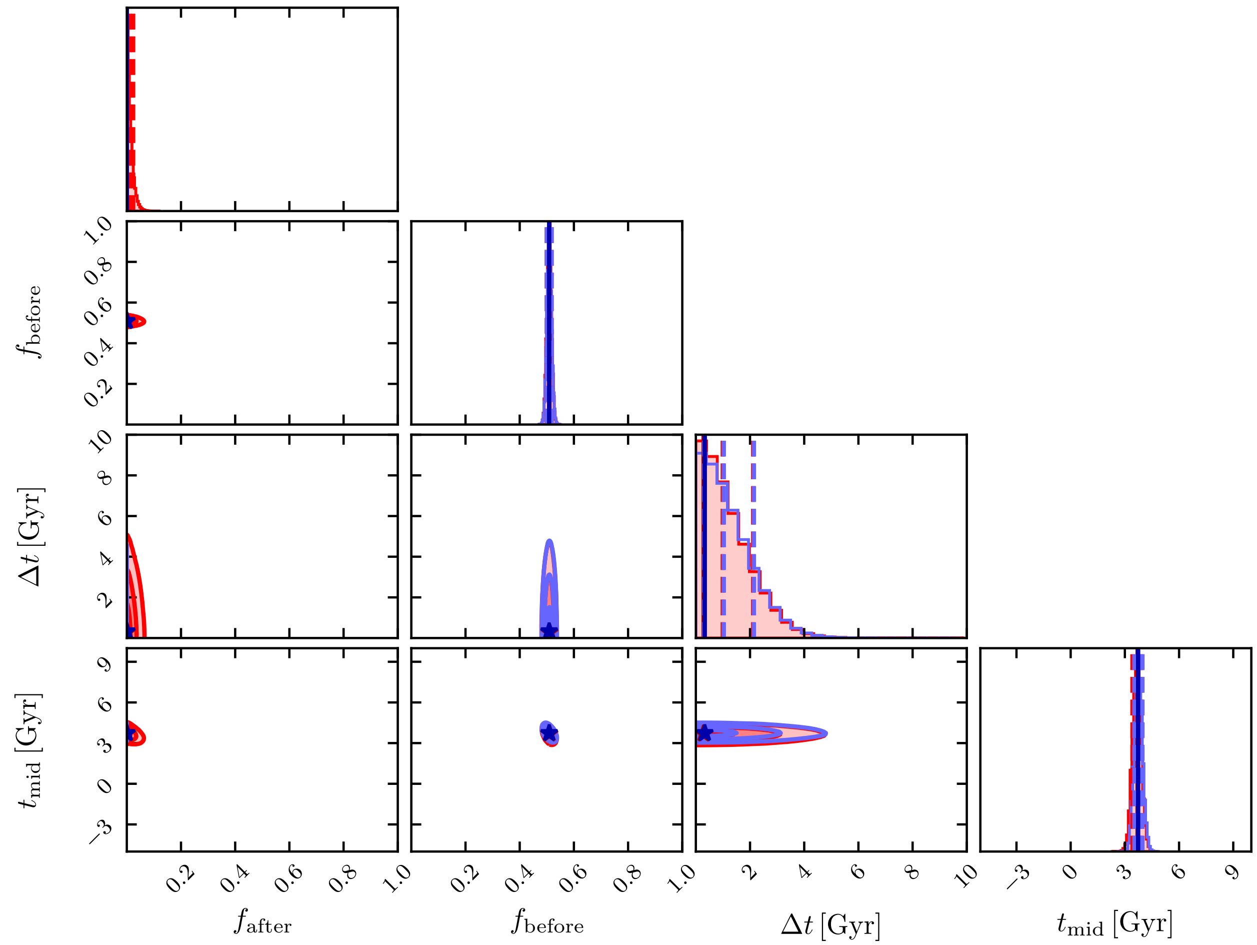


**Figure F39.** As in Fig. F1, but for the $(g-r)$ colour analysis of the $M_{\rm host}/{\rm M}_{\odot} > 10^{14}$ sample, third stellar mass bin.

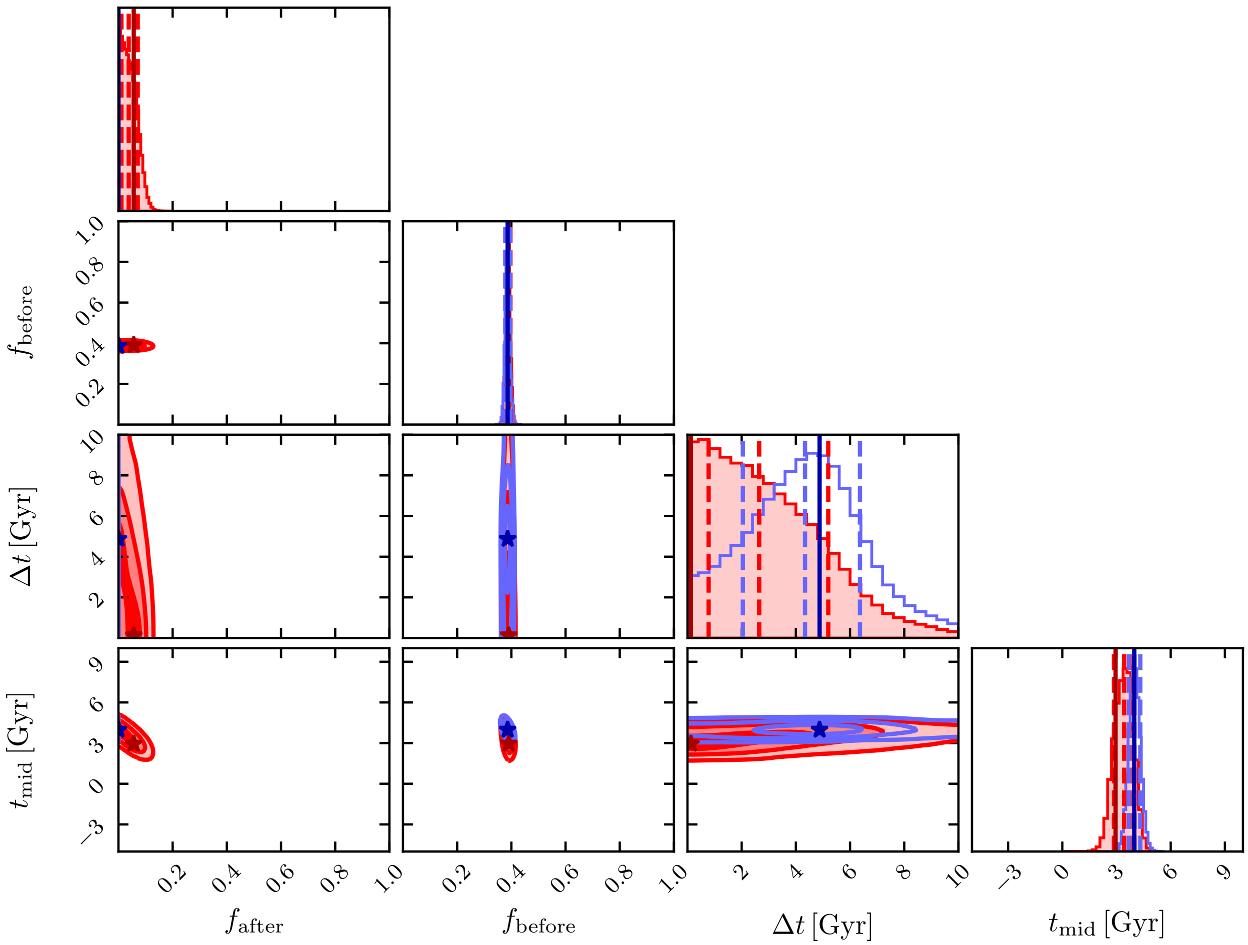


**Figure F40.** As in Fig. F1, but for the $(g-r)$ colour analysis of the $M_{\rm host}/{\rm M}_{\odot} > 10^{14}$ sample, fourth stellar mass bin.

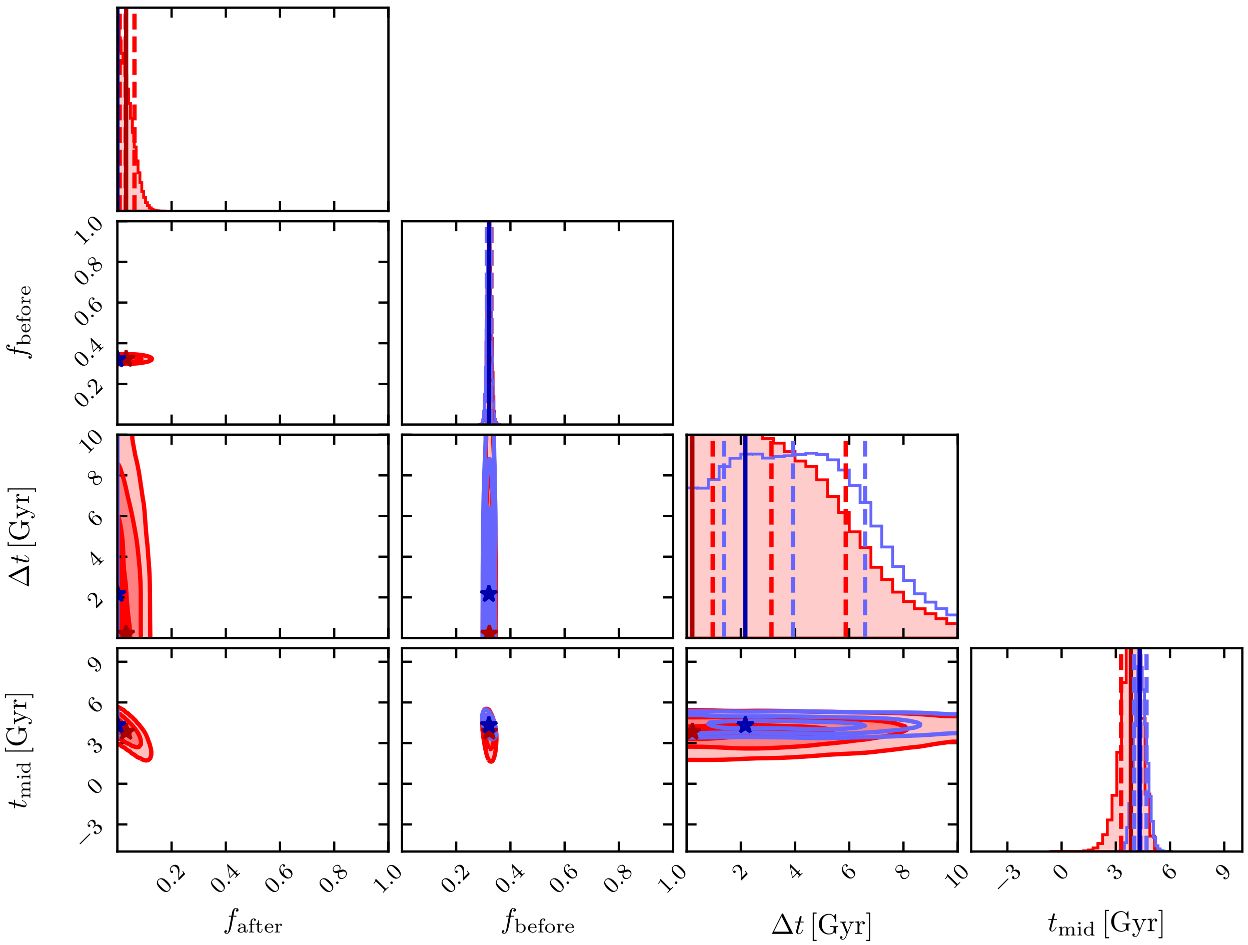


**Figure F41.** As in Fig. F1, but for the $(g-r)$ colour analysis of the $M_{\rm host}/{\rm M}_{\odot} > 10^{14}$ sample, fifth stellar mass bin.

© 0000 RAS, MNRAS **000**, 000–000

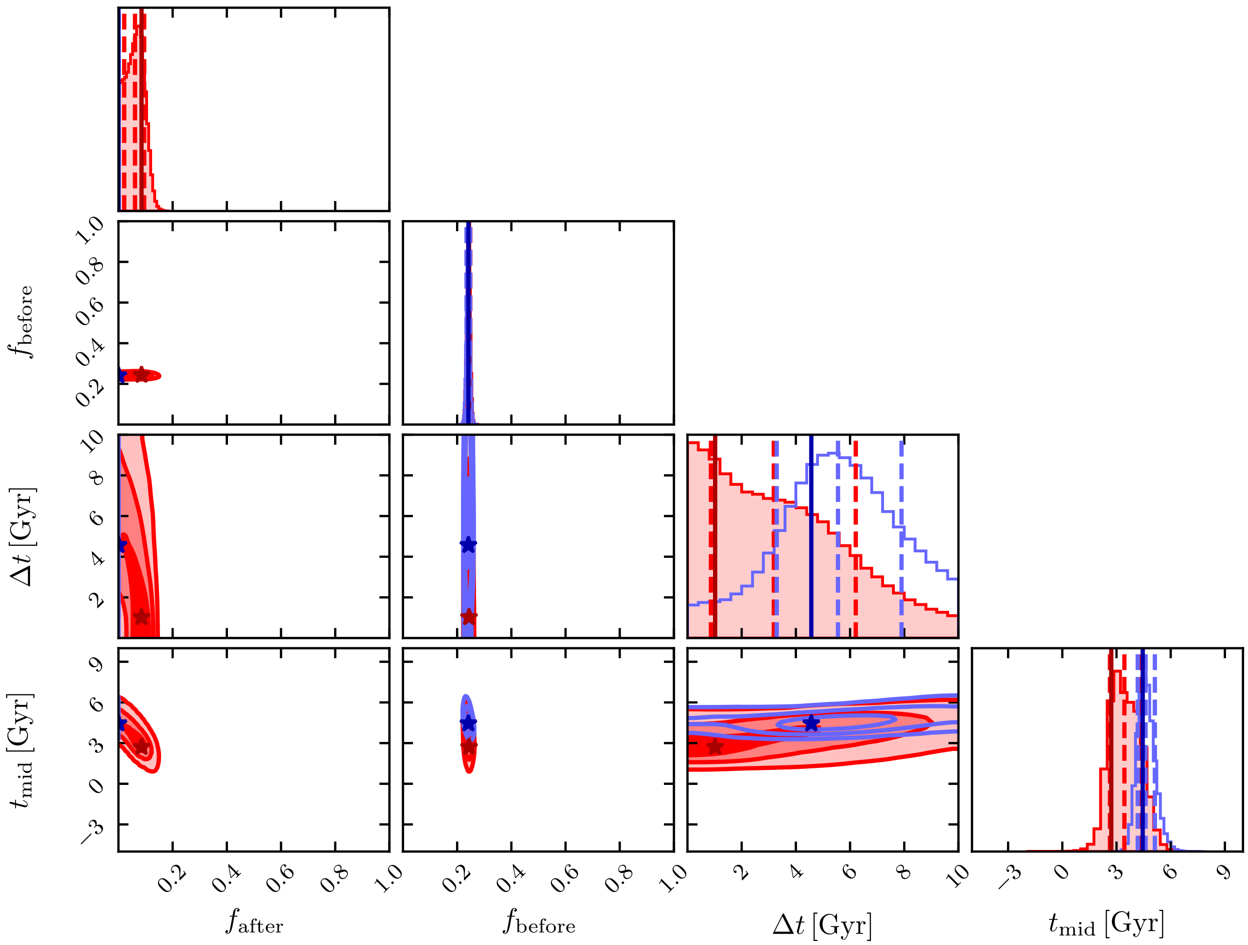


**Figure F42.** As in Fig. F1, but for the $(g-r)$ colour analysis of the $M_{\rm host}/{\rm M}_\odot > 10^{14}$ sample, sixth stellar mass bin.

© 0000 RAS, MNRAS **000**, 000–000

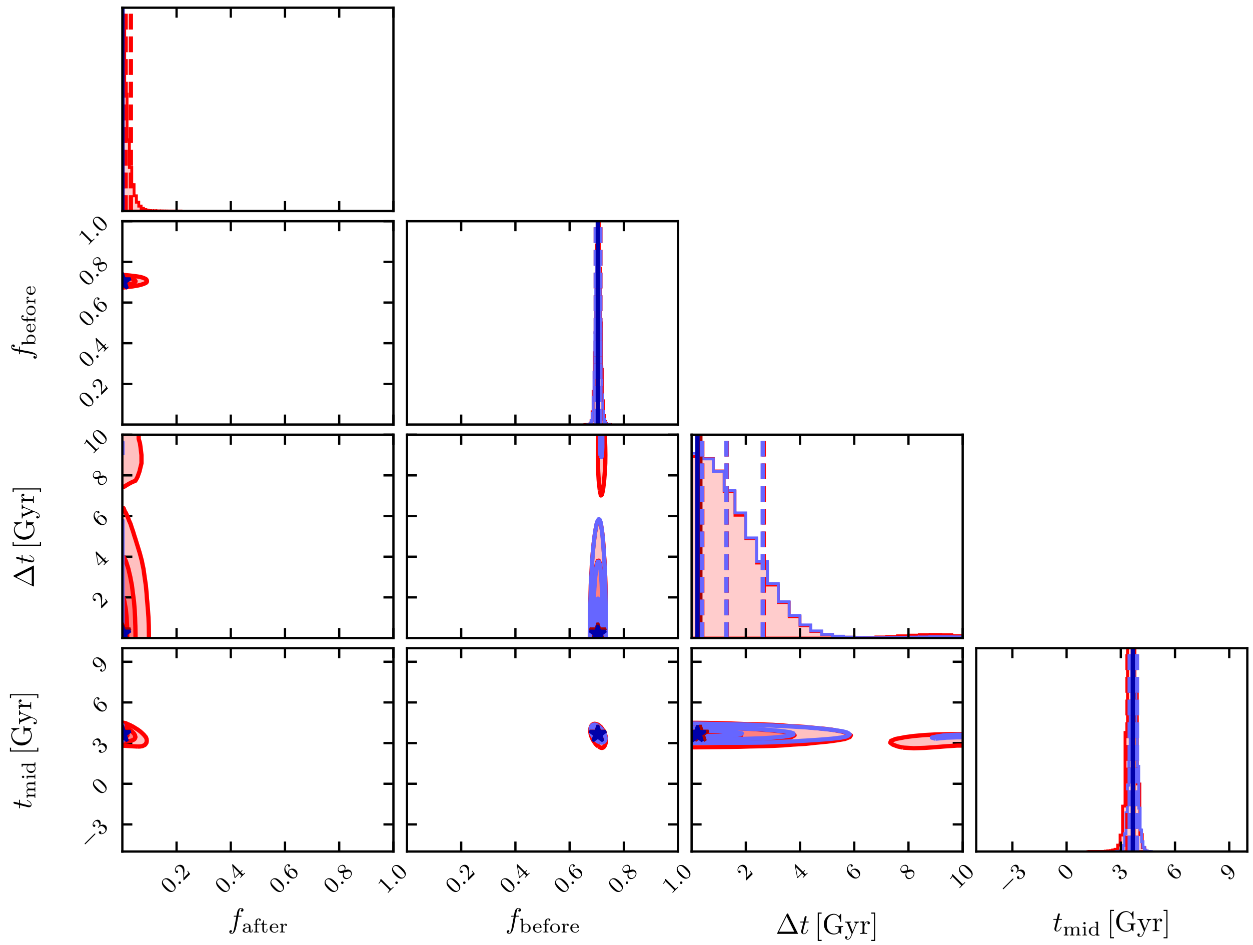


**Figure F43.** As in Fig. F1, but for the SSFR analysis of the $M_{\rm host}/{\rm M}_\odot > 10^{14}$ sample, first stellar mass bin.

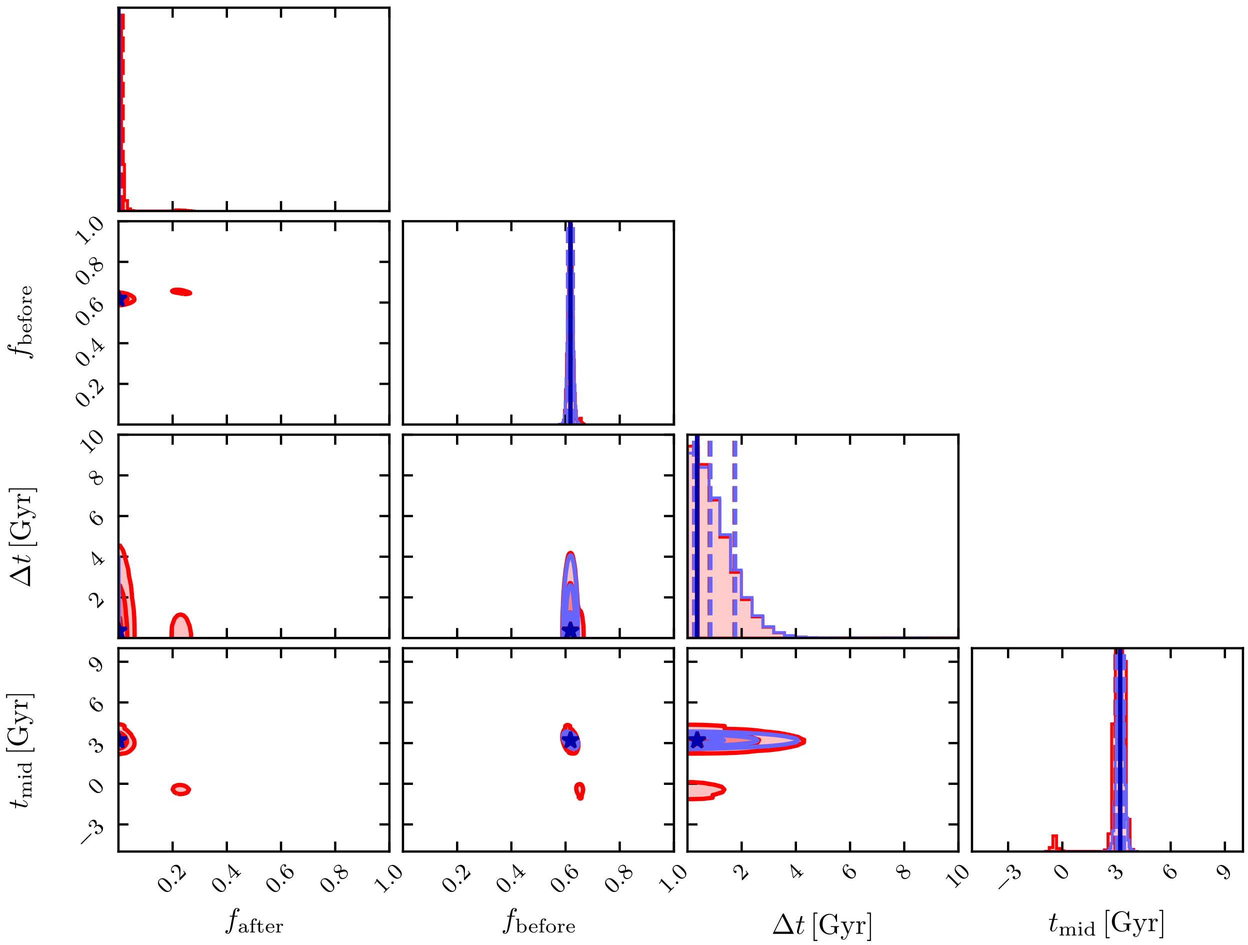


**Figure F44.** As in Fig. F1, but for the SSFR analysis of the $M_{\rm host}/{\rm M}_{\odot} > 10^{14}$ sample, second stellar mass bin.

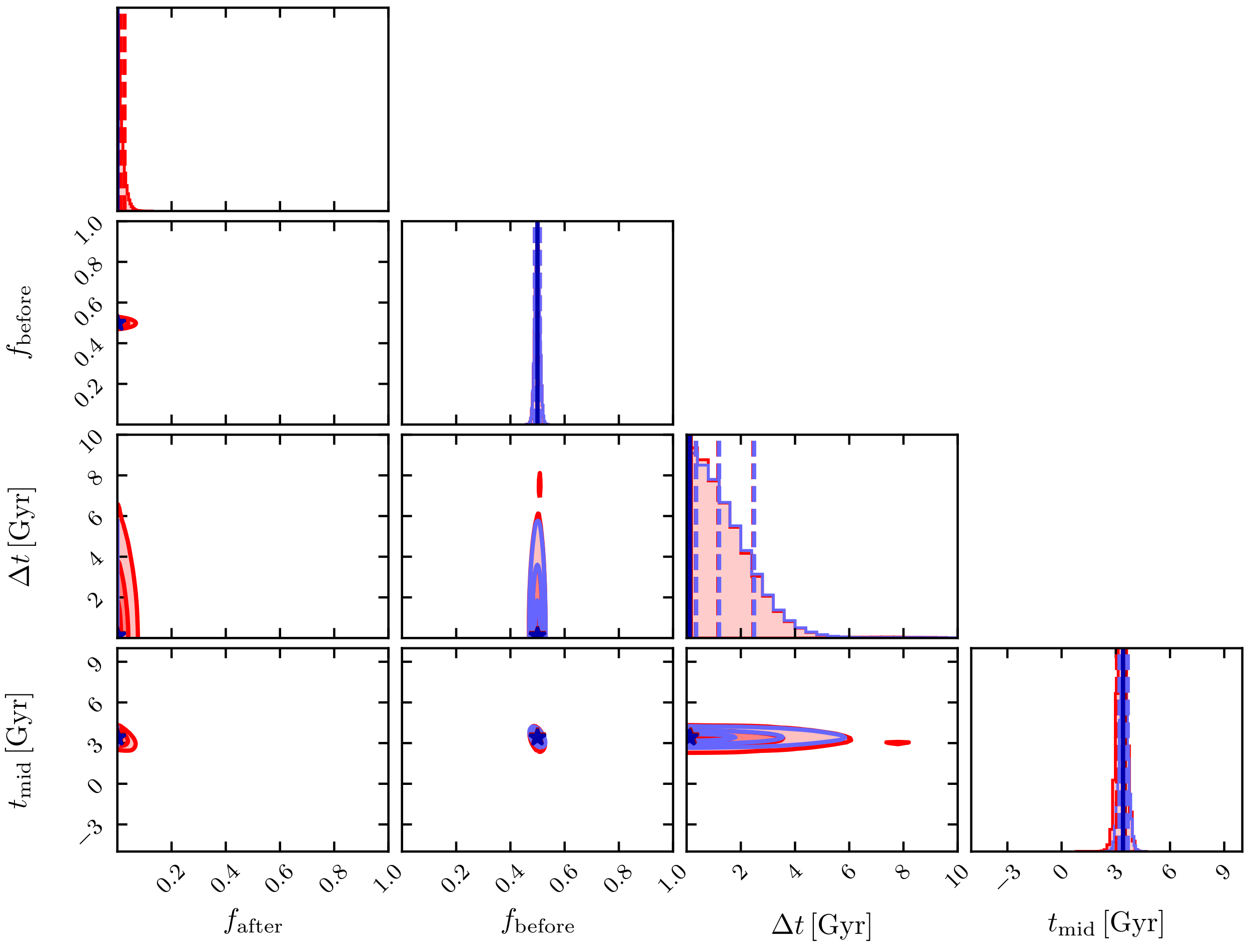


**Figure F45.** As in Fig. F1, but for the SSFR analysis of the $M_{\rm host}/{\rm M}_{\odot} > 10^{14}$ sample, third stellar mass bin.

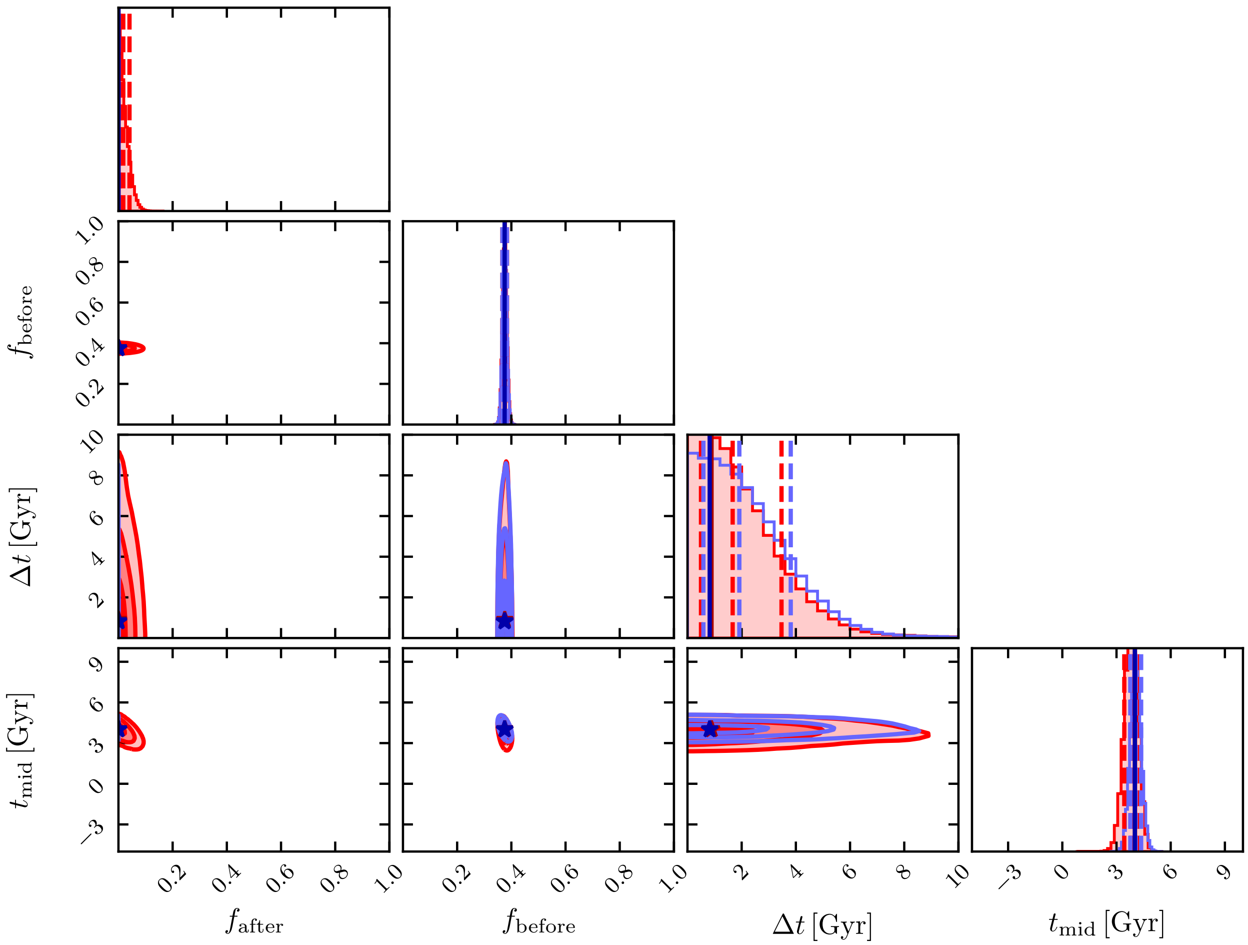


**Figure F46.** As in Fig. F1, but for the SSFR analysis of the $M_{\rm host}/{\rm M}_{\odot} > 10^{14}$ sample, fourth stellar mass bin.

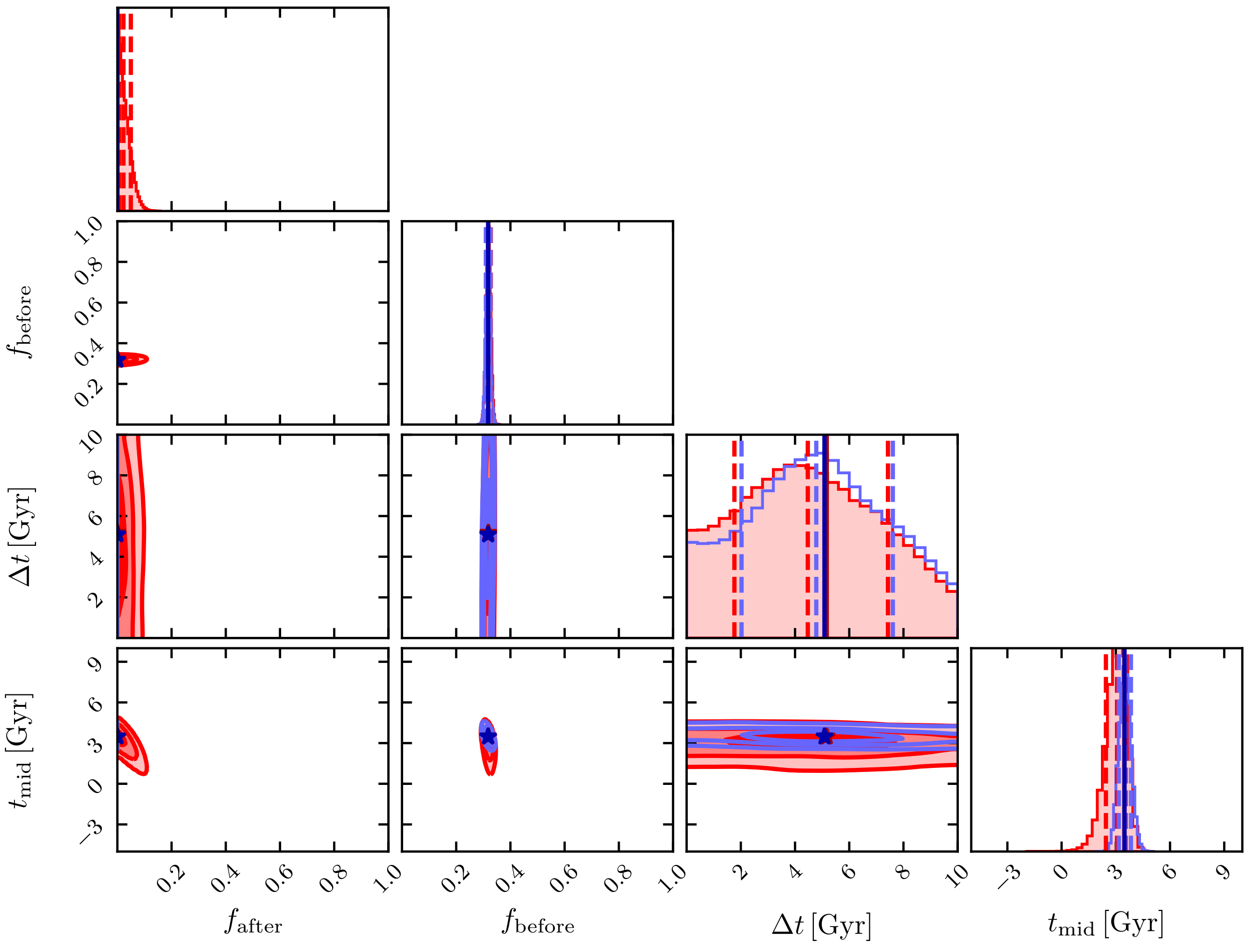


**Figure F47.** As in Fig. F1, but for the SSFR analysis of the $M_{\rm host}/{\rm M}_{\odot} > 10^{14}$ sample, fifth stellar mass bin.

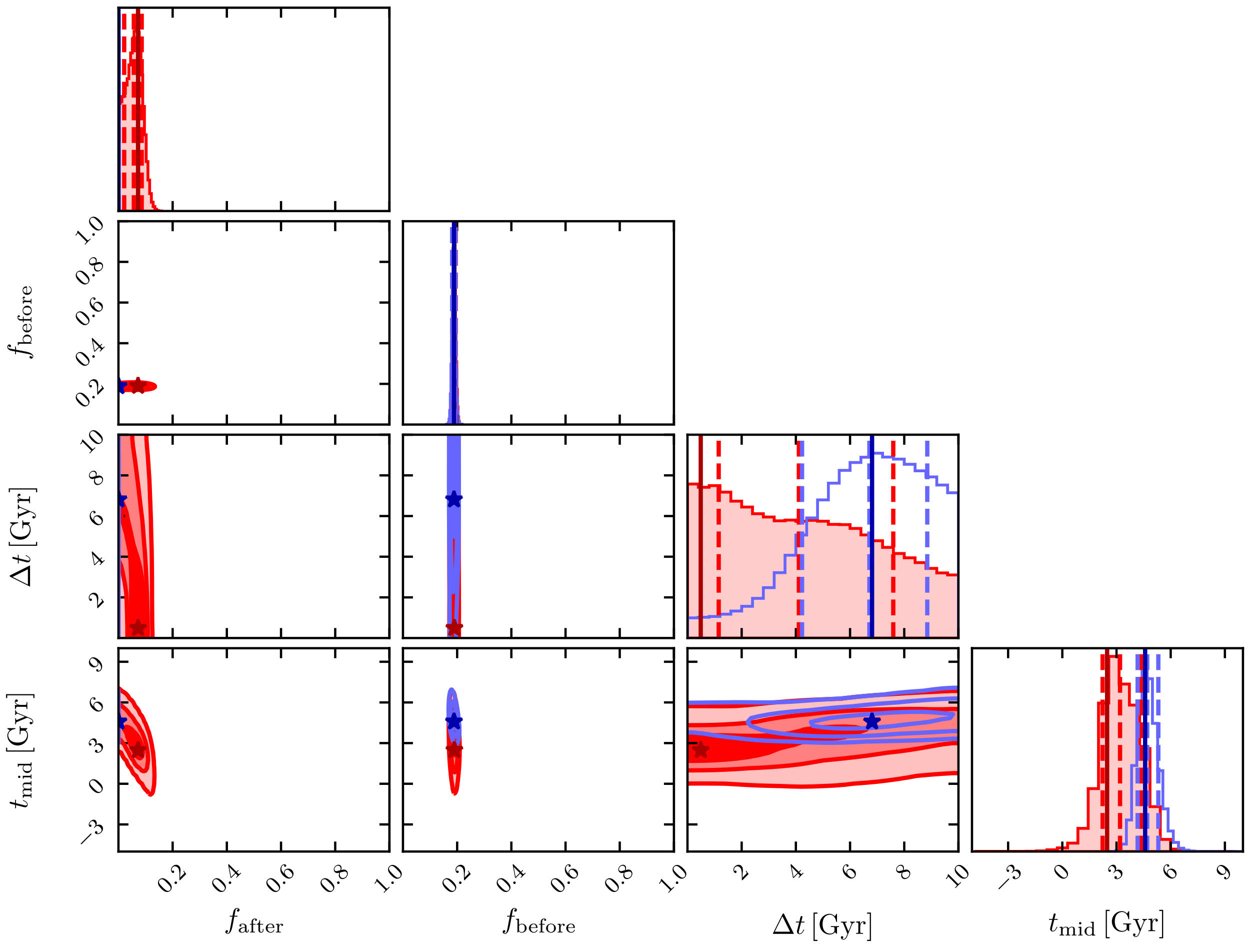


**Figure F48.** As in Fig. F1, but for the SSFR analysis of the $M_{\rm host}/{\rm M}_{\odot} > 10^{14}$ sample, sixth stellar mass bin.

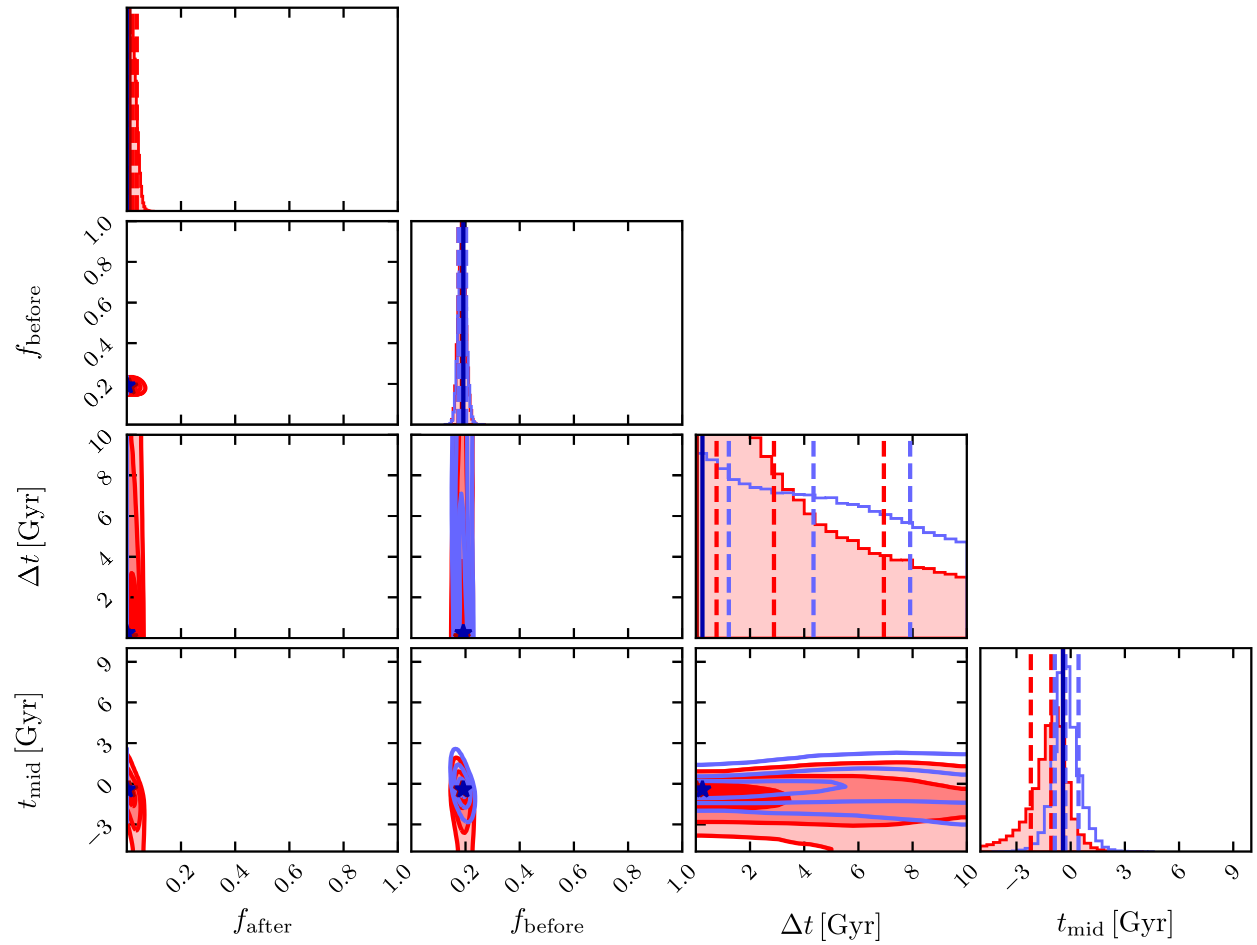


**Figure F49.** As in Fig. F1, but for the gas analysis of the $M_{\rm host}/{\rm M}_{\odot} > 10^{14}$ sample, first stellar mass bin.

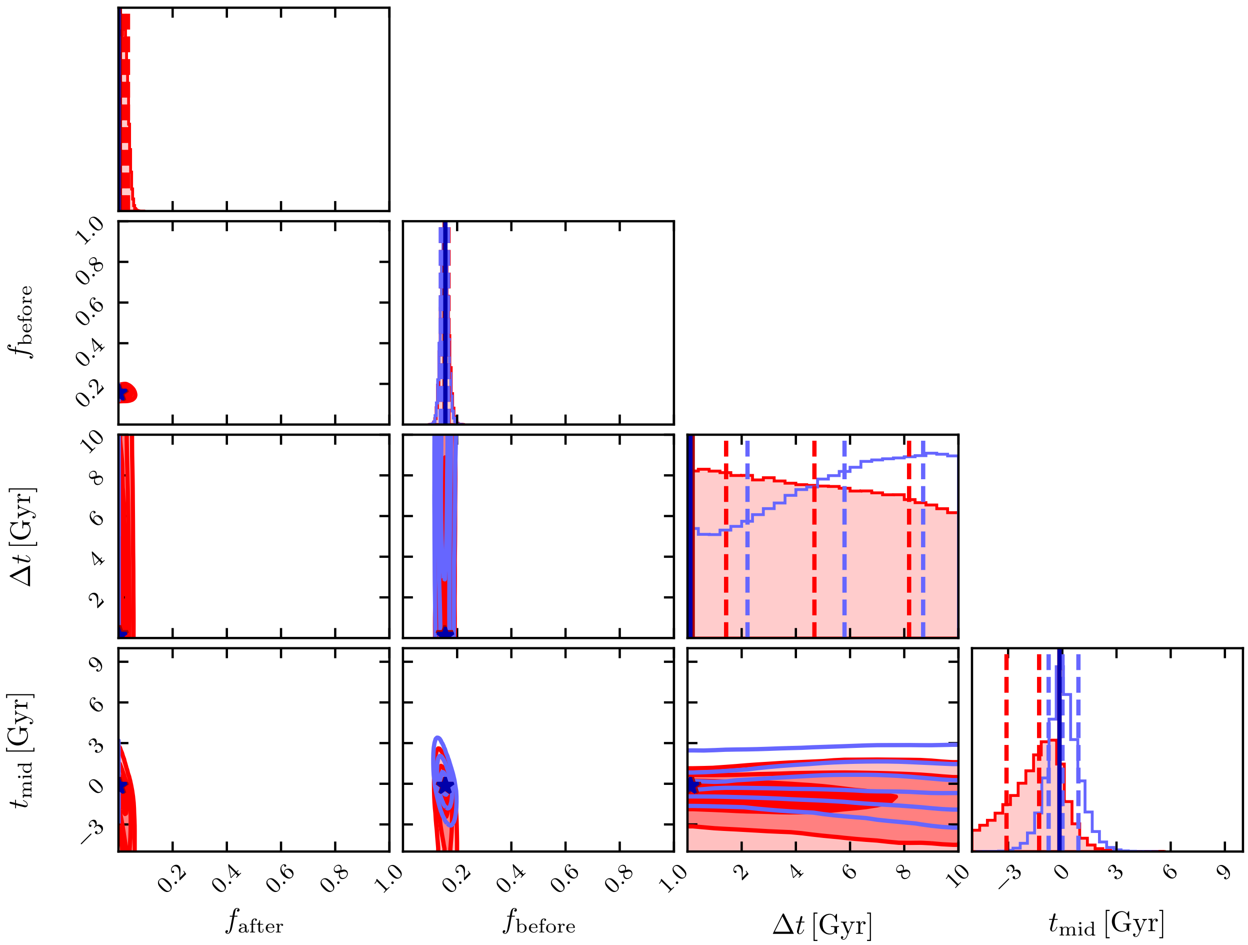


**Figure F50.** As in Fig. F1, but for the gas analysis of the $M_{\mathrm{host}}/\mathrm{M}_{\odot} > 10^{14}$ sample, second stellar mass bin.

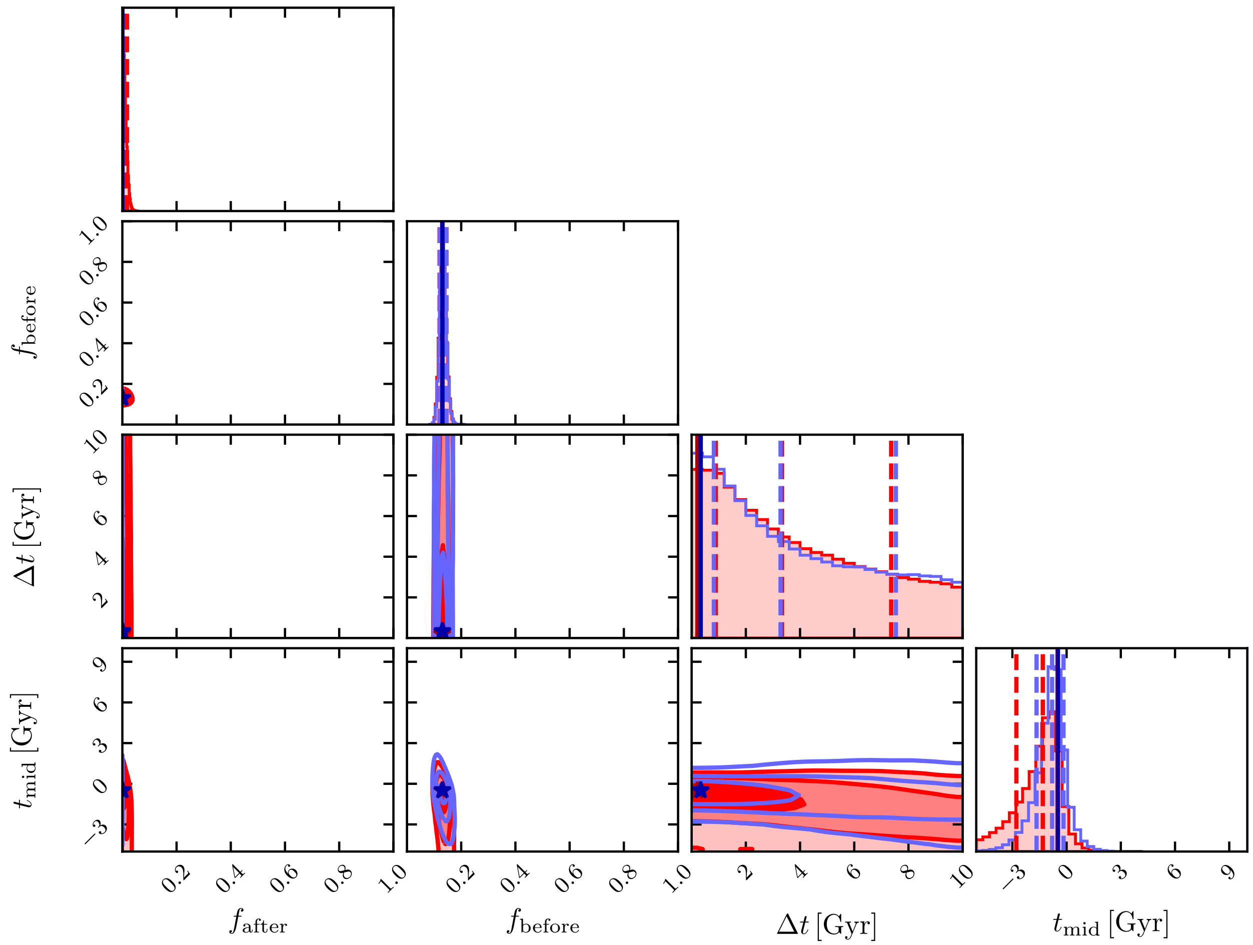


**Figure F51.** As in Fig. F1, but for the gas analysis of the $M_{\rm host}/{\rm M}_{\odot} > 10^{14}$ sample, third stellar mass bin.

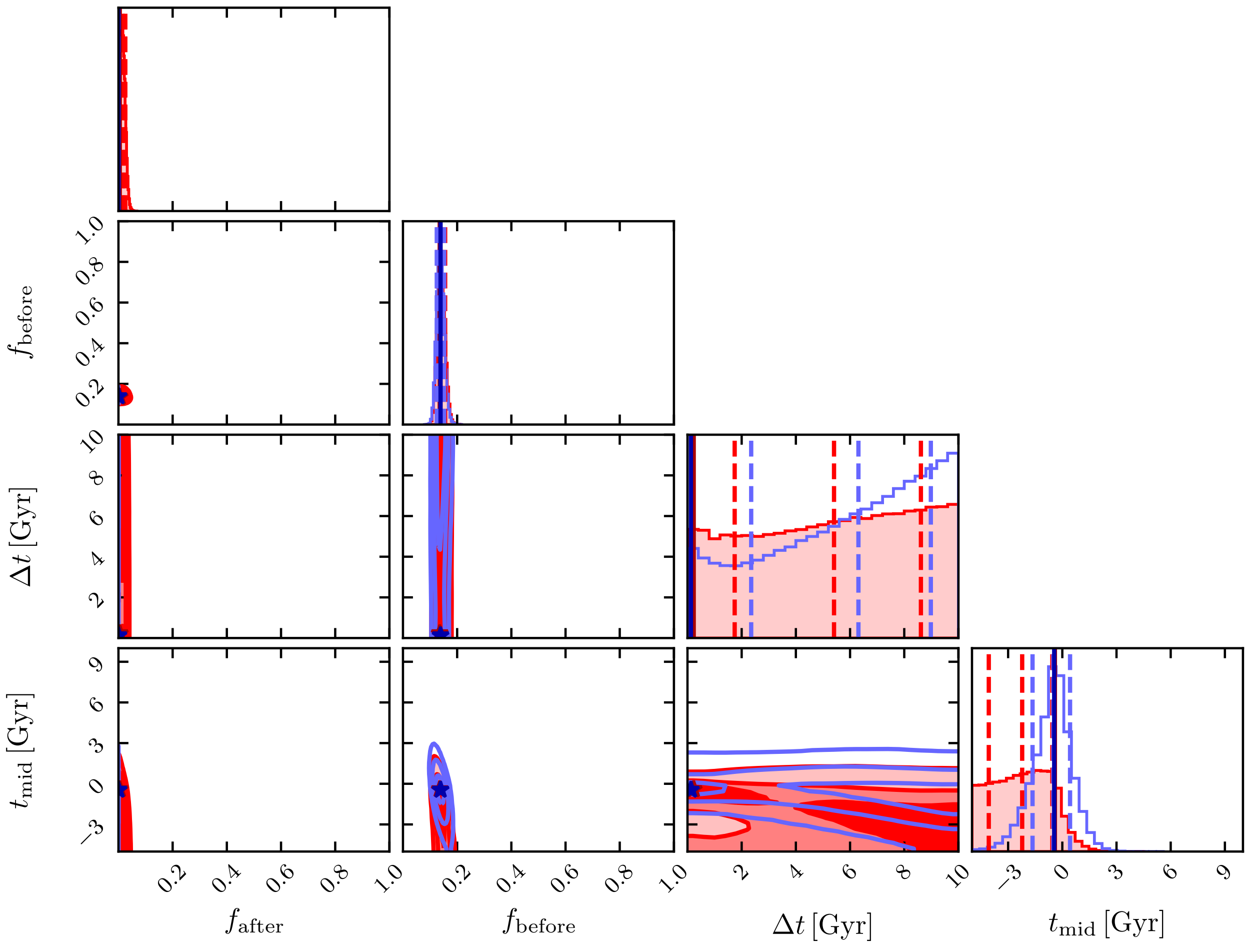


**Figure F52.** As in Fig. F1, but for the gas analysis of the $M_{\rm host}/{\rm M}_{\odot} > 10^{14}$ sample, fourth stellar mass bin.

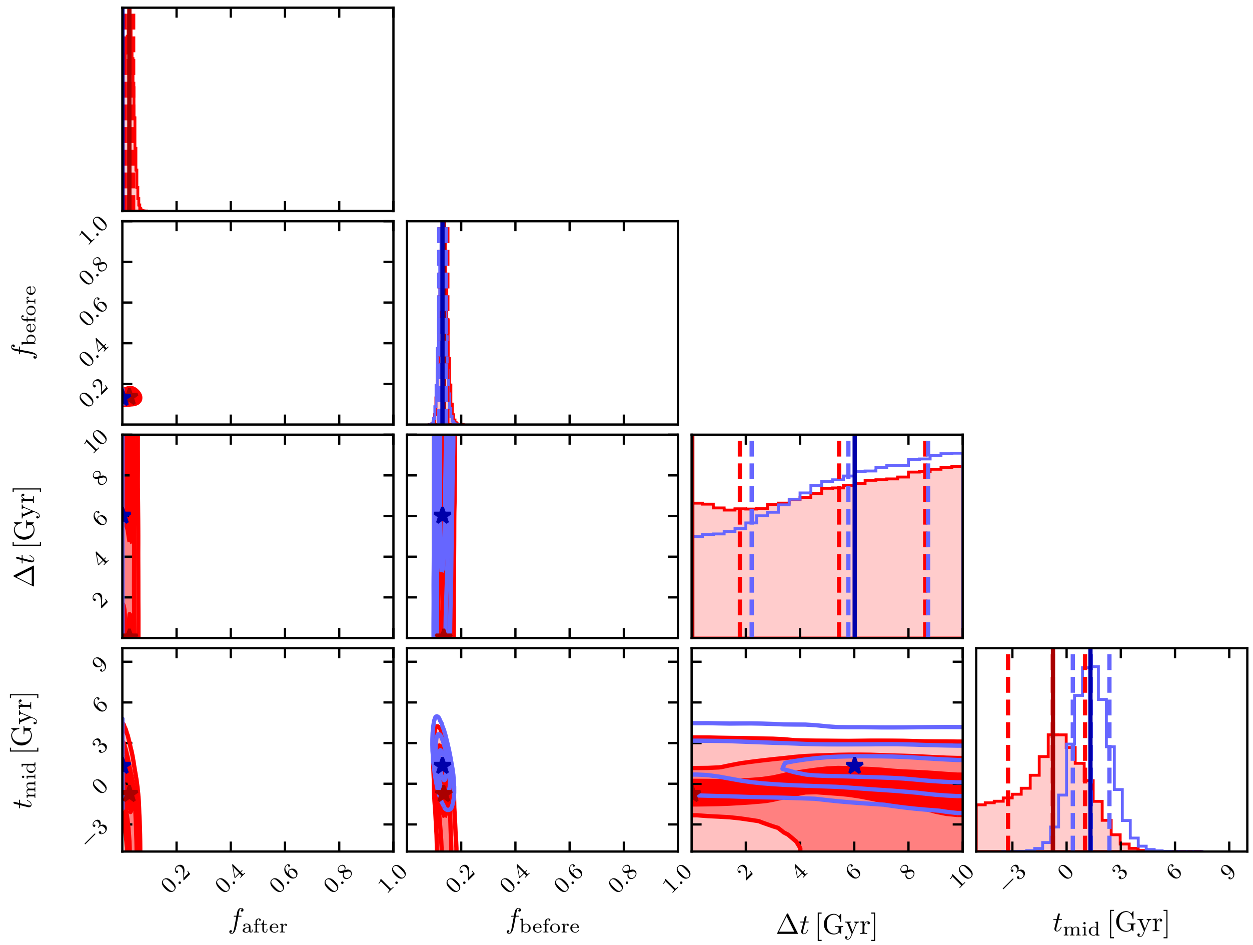


**Figure F53.** As in Fig. F1, but for the gas analysis of the $M_{\rm host}/{\rm M}_{\odot} > 10^{14}$ sample, fifth stellar mass bin.

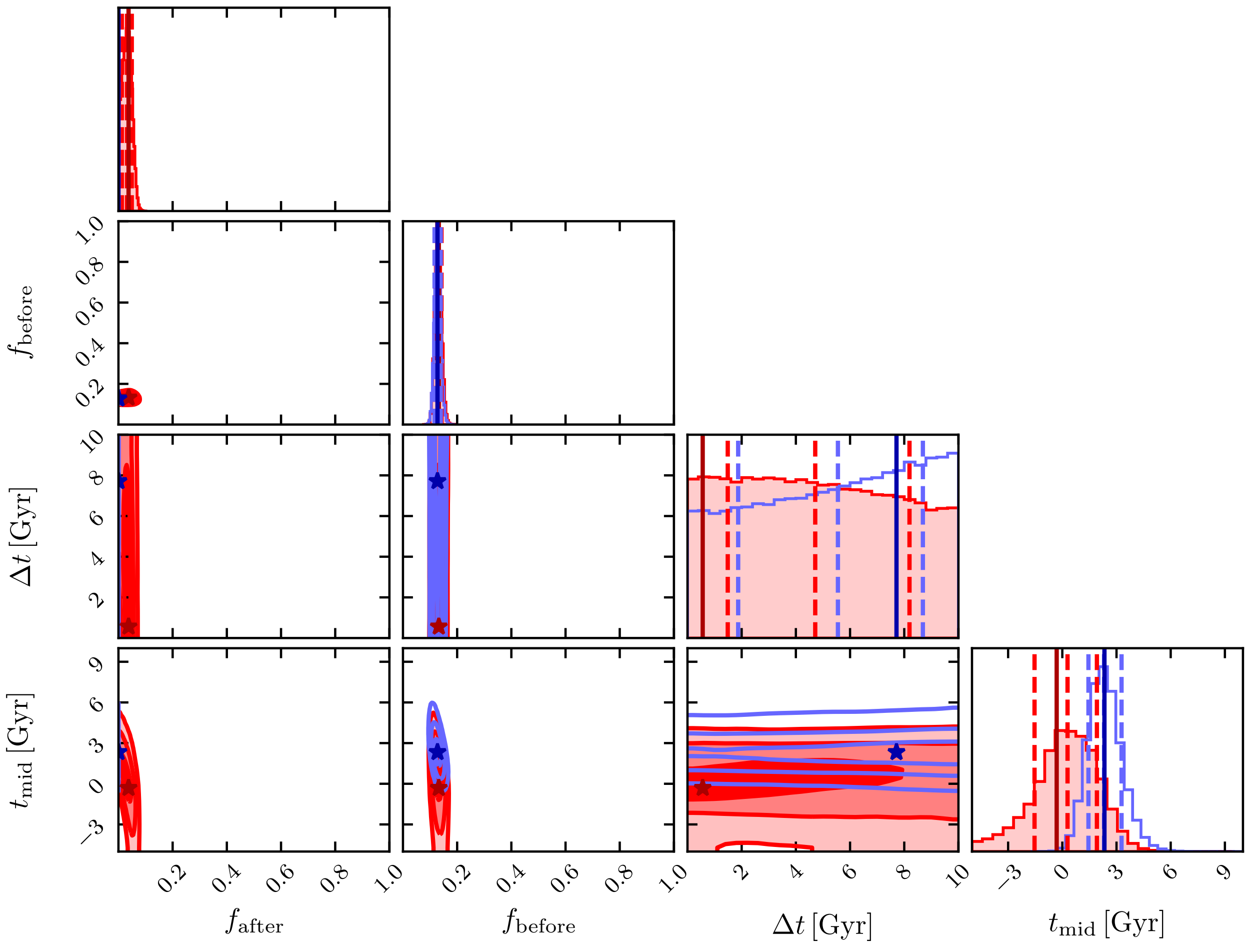


**Figure F54.** As in Fig. F1, but for the gas analysis of the $M_{\rm host}/{\rm M}_{\odot} > 10^{14}$ sample, sixth stellar mass bin.

© 0000 RAS, MNRAS **000**, 000–000
